# Supplementary material for: Bridge functions of classical one-component plasmas
Source: arXiv:2108.09574 ancillary file (2021-10-01)
Supplement: Supplementary file 1 [file supplementary_material_final.pdf]

# Bridge functions of classical one-component plasmas
# Supplementary material

F. Lucco Castello and P. Tolias
*Space and Plasma Physics, Royal Institute of Technology, Stockholm, SE-100 44, Sweden*

Supplementary material for the manuscript entitled "Bridge functions of classical one-component plasmas". The **first part** features a detailed comparison of the indirectly extracted OCP bridge functions with our newly-proposed parametrization and with other parametrizations earlier proposed in the literature as well as a comprehensive presentation of the error bars. The **second part** features extensive comparisons of the results of the original and updated versions of the IEMHNC approach with computer simulation results. In particular, it contains extensive tabulations of key functional properties of the YOCP radial distribution functions and of reduced excess internal energies.

## Contents of the first part

**Figure 1**: OCP bridge function results for $\Gamma = 170$.

**Figure 2**: OCP bridge function results for $\Gamma = 160$.

**Figure 3**: OCP bridge function results for $\Gamma = 150$.

**Figure 4**: OCP bridge function results for $\Gamma = 140$.

**Figure 5**: OCP bridge function results for $\Gamma = 130$.

**Figure 6**: OCP bridge function results for $\Gamma = 120$.

**Figure 7**: OCP bridge function results for $\Gamma = 110$.

**Figure 8**: OCP bridge function results for $\Gamma = 100$.

**Figure 9**: OCP bridge function results for $\Gamma = 90$.

**Figure 10**: OCP bridge function results for $\Gamma = 80$.

**Figure 11**: OCP bridge function results for $\Gamma = 70$.

**Figure 12**: OCP bridge function results for $\Gamma = 60$.

**Figure 13**: OCP bridge function results for $\Gamma = 50$.

**Figure 14**: OCP bridge function results for $\Gamma = 40$.

**Figure 15**: OCP bridge function results for $\Gamma = 30$.

**Figure 16**: OCP bridge function results for $\Gamma = 20$.

**Figure 17**: OCP bridge function results for $\Gamma = 10$.

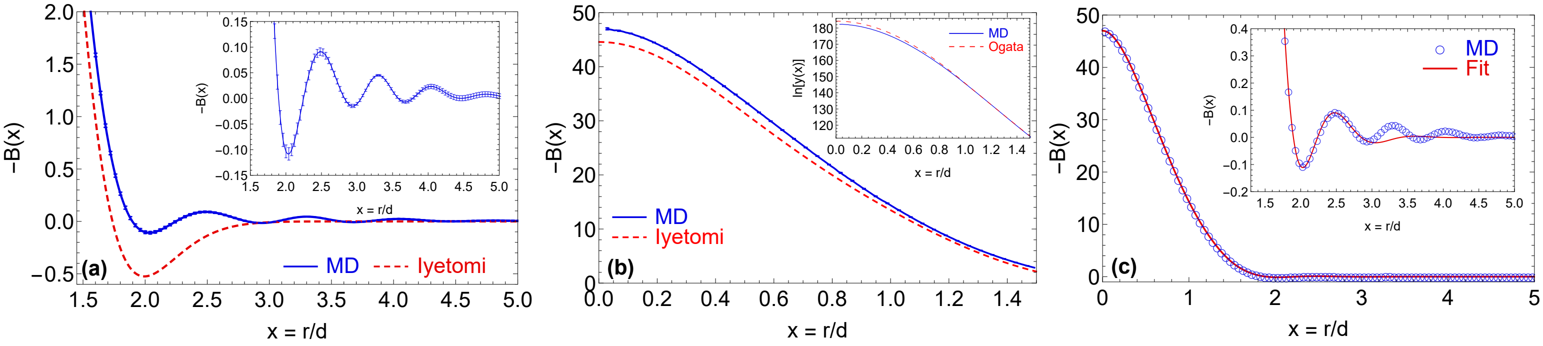


**Figure 1.** $\Gamma = 170$. (a) The OCP bridge functions in the intermediate and long range $1.5 \leq x \leq 5$ as computed from the OZ inversion method with input from our accurate standard MD simulations versus the OCP bridge functions as calculated from the Iyetomi *et al.* parametrization. The error bars stem from the statistical uncertainties and correspond to 95% confidence intervals. (b) *Main.* The OCP bridge functions in the short range $0 \leq x \leq 1.5$ as computed from the cavity distribution method with input from specially designed long cavity MD simulations versus the OCP bridge functions as calculated from the Iyetomi *et al.* parametrization. The small error bars, that originate from the statistical uncertainties, correspond to 95% confidence intervals. *Inset.* The OCP screening potentials in the short range $0 \leq x \leq 1.5$ as computed from the cavity distribution method with input from specially designed long cavity MD simulations versus the OCP screening potentials as calculated from the Ogata parametrization. (c) The indirectly extracted OCP bridge functions (blue circles, downsampled) versus the analytically parameterized bridge functions (red solid lines). *Main.* The OCP bridge functions in the entire non-trivial interval $0 \leq x \leq 5.0$, where only the monotonic behavior of the short range is discernible. *Inset.* Zoom-in on the OCP bridge functions in the intermediate & long range interval $1.5 \leq x \leq 5.0$, where only the oscillatory decaying behavior is discernible.

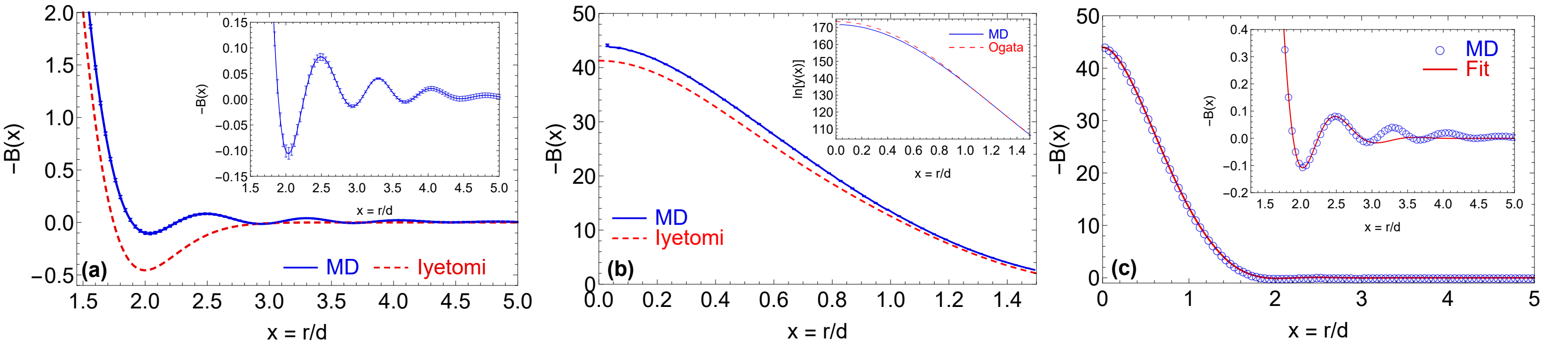


**Figure 2.** $\Gamma = 160$. (a) The OCP bridge functions in the intermediate and long range $1.5 \leq x \leq 5$ as computed from the OZ inversion method with input from our accurate standard MD simulations versus the OCP bridge functions as calculated from the Iyetomi *et al.* parametrization. The error bars stem from the statistical uncertainties and correspond to 95% confidence intervals. (b) *Main.* The OCP bridge functions in the short range $0 \leq x \leq 1.5$ as computed from the cavity distribution method with input from specially designed long cavity MD simulations versus the OCP bridge functions as calculated from the Iyetomi *et al.* parametrization. The small error bars, that originate from the statistical uncertainties, correspond to 95% confidence intervals. *Inset.* The OCP screening potentials in the short range $0 \leq x \leq 1.5$ as computed from the cavity distribution method with input from specially designed long cavity MD simulations versus the OCP screening potentials as calculated from the Ogata parametrization. (c) The indirectly extracted OCP bridge functions (blue circles, downsampled) versus the analytically parameterized bridge functions (red solid lines). *Main.* The OCP bridge functions in the entire non-trivial interval $0 \leq x \leq 5.0$, where only the monotonic behavior of the short range is discernible. *Inset.* Zoom-in on the OCP bridge functions in the intermediate & long range interval $1.5 \leq x \leq 5.0$, where only the oscillatory decaying behavior is discernible.

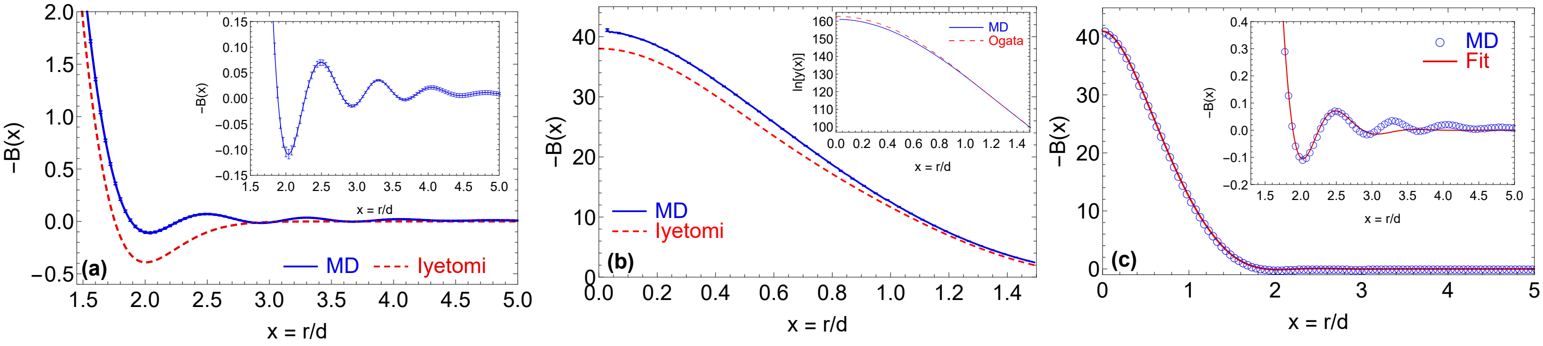


**Figure 3.** $\Gamma = 150$. (a) The OCP bridge functions in the intermediate and long range $1.5 \leq x \leq 5$ as computed from the OZ inversion method with input from our accurate standard MD simulations versus the OCP bridge functions as calculated from the Iyetomi *et al.* parametrization. The error bars stem from the statistical uncertainties and correspond to 95% confidence intervals. (b) *Main.* The OCP bridge functions in the short range $0 \leq x \leq 1.5$ as computed from the cavity distribution method with input from specially designed long cavity MD simulations versus the OCP bridge functions as calculated from the Iyetomi *et al.* parametrization. The small error bars, that originate from the statistical uncertainties, correspond to 95% confidence intervals. *Inset.* The OCP screening potentials in the short range $0 \leq x \leq 1.5$ as computed from the cavity distribution method with input from specially designed long cavity MD simulations versus the OCP screening potentials as calculated from the Ogata parametrization. (c) The indirectly extracted OCP bridge functions (blue circles, downsampled) versus the analytically parameterized bridge functions (red solid lines). *Main.* The OCP bridge functions in the entire non-trivial interval $0 \leq x \leq 5.0$, where only the monotonic behavior of the short range is discernible. *Inset.* Zoom-in on the OCP bridge functions in the intermediate & long range interval $1.5 \leq x \leq 5.0$, where only the oscillatory decaying behavior is discernible.

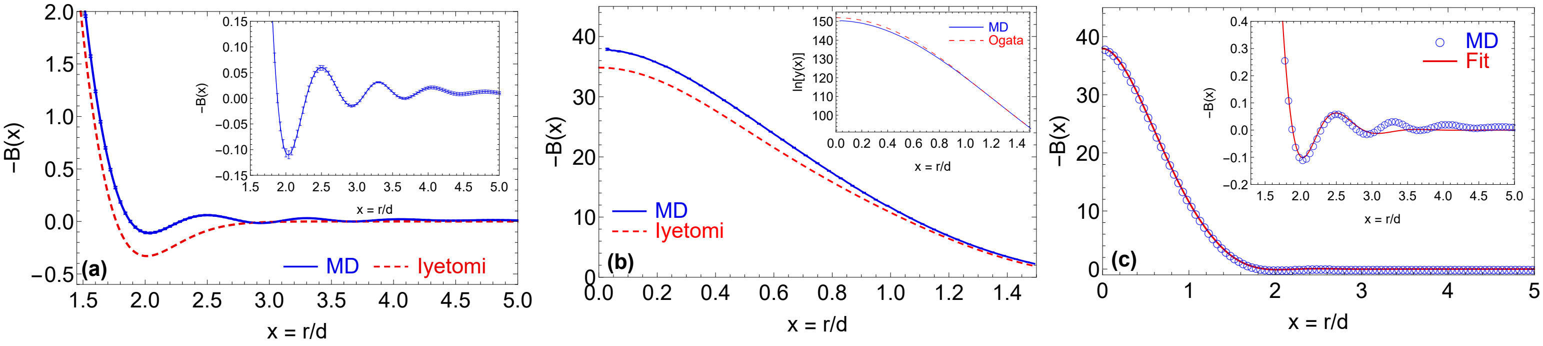


**Figure 4.** $\Gamma = 140$. (a) The OCP bridge functions in the intermediate and long range $1.5 \leq x \leq 5$ as computed from the OZ inversion method with input from our accurate standard MD simulations versus the OCP bridge functions as calculated from the Iyetomi *et al.* parametrization. The error bars stem from the statistical uncertainties and correspond to 95% confidence intervals. (b) *Main.* The OCP bridge functions in the short range $0 \leq x \leq 1.5$ as computed from the cavity distribution method with input from specially designed long cavity MD simulations versus the OCP bridge functions as calculated from the Iyetomi *et al.* parametrization. The small error bars, that originate from the statistical uncertainties, correspond to 95% confidence intervals. *Inset.* The OCP screening potentials in the short range $0 \leq x \leq 1.5$ as computed from the cavity distribution method with input from specially designed long cavity MD simulations versus the OCP screening potentials as calculated from the Ogata parametrization. (c) The indirectly extracted OCP bridge functions (blue circles, downsampled) versus the analytically parameterized bridge functions (red solid lines). *Main.* The OCP bridge functions in the entire non-trivial interval $0 \leq x \leq 5.0$, where only the monotonic behavior of the short range is discernible. *Inset.* Zoom-in on the OCP bridge functions in the intermediate & long range interval $1.5 \leq x \leq 5.0$, where only the oscillatory decaying behavior is discernible.

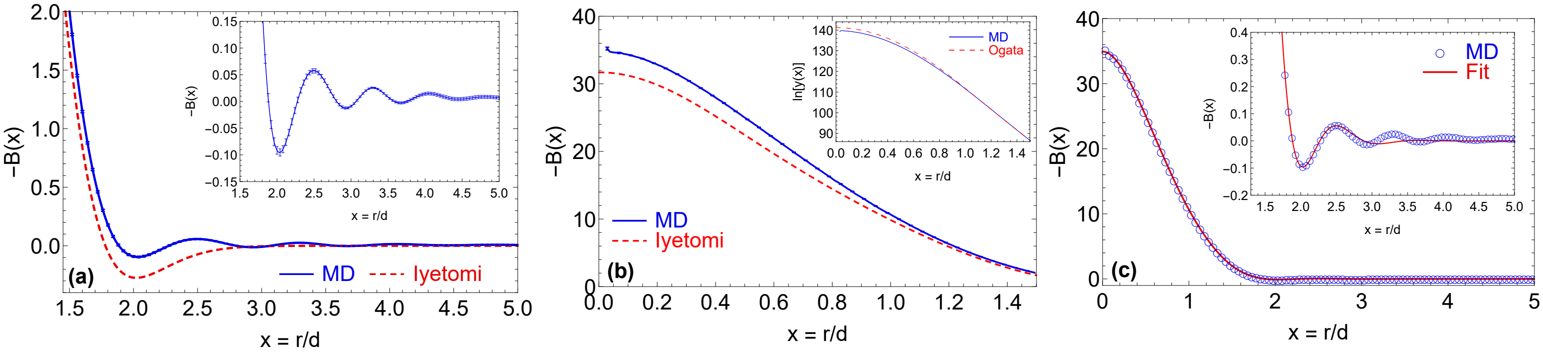


**Figure 5.** $\Gamma = 130$. (a) The OCP bridge functions in the intermediate and long range $1.5 \leq x \leq 5$ as computed from the OZ inversion method with input from our accurate standard MD simulations versus the OCP bridge functions as calculated from the Iyetomi *et al.* parametrization. The error bars stem from the statistical uncertainties and correspond to 95% confidence intervals. (b) *Main.* The OCP bridge functions in the short range $0 \leq x \leq 1.5$ as computed from the cavity distribution method with input from specially designed long cavity MD simulations versus the OCP bridge functions as calculated from the Iyetomi *et al.* parametrization. The small error bars, that originate from the statistical uncertainties, correspond to 95% confidence intervals. *Inset.* The OCP screening potentials in the short range $0 \leq x \leq 1.5$ as computed from the cavity distribution method with input from specially designed long cavity MD simulations versus the OCP screening potentials as calculated from the Ogata parametrization. (c) The indirectly extracted OCP bridge functions (blue circles, downsampled) versus the analytically parameterized bridge functions (red solid lines). *Main.* The OCP bridge functions in the entire non-trivial interval $0 \leq x \leq 5.0$, where only the monotonic behavior of the short range is discernible. *Inset.* Zoom-in on the OCP bridge functions in the intermediate & long range interval $1.5 \leq x \leq 5.0$, where only the oscillatory decaying behavior is discernible.

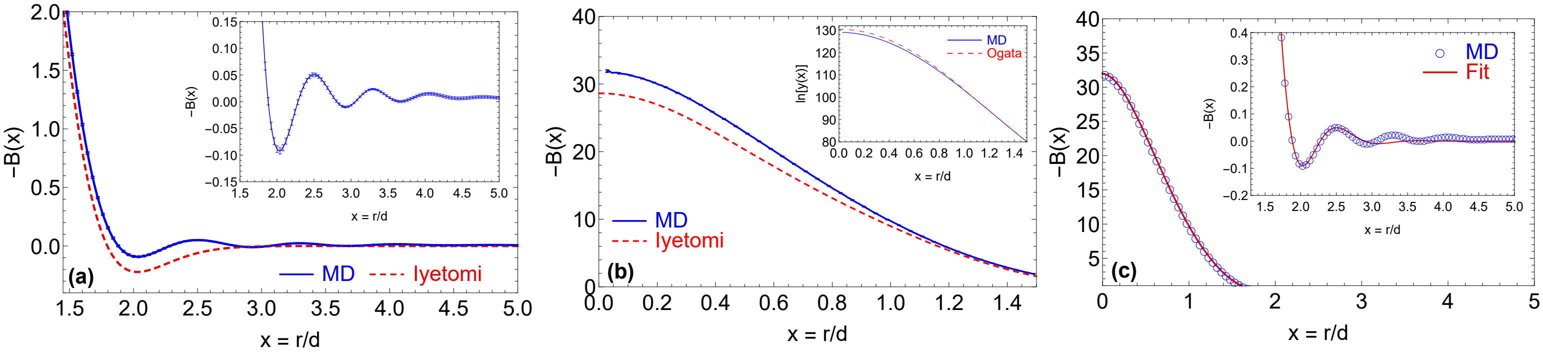


**Figure 6.** $\Gamma = 120$. (a) The OCP bridge functions in the intermediate and long range $1.5 \leq x \leq 5$ as computed from the OZ inversion method with input from our accurate standard MD simulations versus the OCP bridge functions as calculated from the Iyetomi *et al.* parametrization. The error bars stem from the statistical uncertainties and correspond to 95% confidence intervals. (b) *Main.* The OCP bridge functions in the short range $0 \leq x \leq 1.5$ as computed from the cavity distribution method with input from specially designed long cavity MD simulations versus the OCP bridge functions as calculated from the Iyetomi *et al.* parametrization. The small error bars, that originate from the statistical uncertainties, correspond to 95% confidence intervals. *Inset.* The OCP screening potentials in the short range $0 \leq x \leq 1.5$ as computed from the cavity distribution method with input from specially designed long cavity MD simulations versus the OCP screening potentials as calculated from the Ogata parametrization. (c) The indirectly extracted OCP bridge functions (blue circles, downsampled) versus the analytically parameterized bridge functions (red solid lines). *Main.* The OCP bridge functions in the entire non-trivial interval $0 \leq x \leq 5.0$, where only the monotonic behavior of the short range is discernible. *Inset.* Zoom-in on the OCP bridge functions in the intermediate & long range interval $1.5 \leq x \leq 5.0$, where only the oscillatory decaying behavior is discernible.

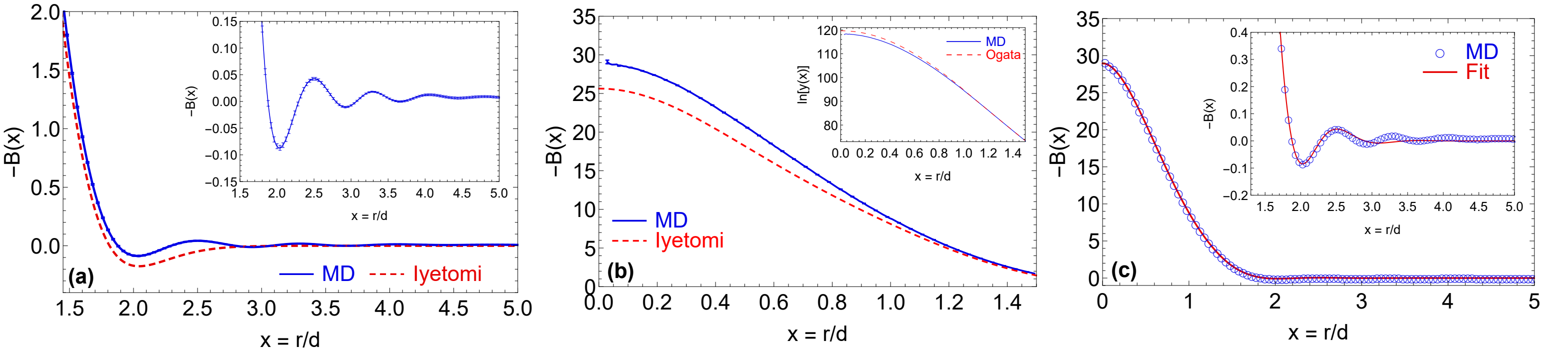


**Figure 7.** $\Gamma = 110$. (a) The OCP bridge functions in the intermediate and long range $1.5 \leq x \leq 5$ as computed from the OZ inversion method with input from our accurate standard MD simulations versus the OCP bridge functions as calculated from the Iyetomi *et al.* parametrization. The error bars stem from the statistical uncertainties and correspond to 95% confidence intervals. (b) *Main.* The OCP bridge functions in the short range $0 \leq x \leq 1.5$ as computed from the cavity distribution method with input from specially designed long cavity MD simulations versus the OCP bridge functions as calculated from the Iyetomi *et al.* parametrization. The small error bars, that originate from the statistical uncertainties, correspond to 95% confidence intervals. *Inset.* The OCP screening potentials in the short range $0 \leq x \leq 1.5$ as computed from the cavity distribution method with input from specially designed long cavity MD simulations versus the OCP screening potentials as calculated from the Ogata parametrization. (c) The indirectly extracted OCP bridge functions (blue circles, downsampled) versus the analytically parameterized bridge functions (red solid lines). *Main.* The OCP bridge functions in the entire non-trivial interval $0 \leq x \leq 5.0$, where only the monotonic behavior of the short range is discernible. *Inset.* Zoom-in on the OCP bridge functions in the intermediate & long range interval $1.5 \leq x \leq 5.0$, where only the oscillatory decaying behavior is discernible.

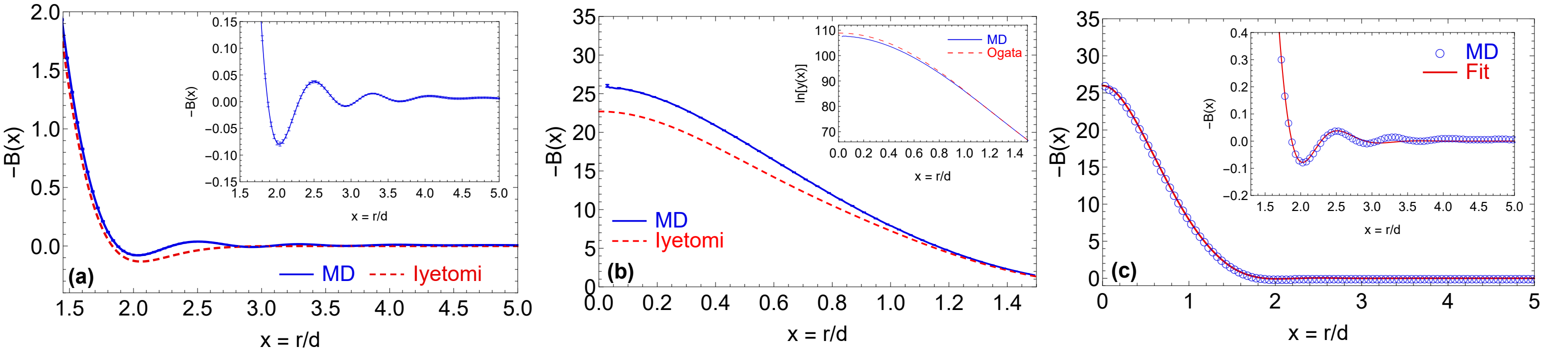


**Figure 8.** $\Gamma = 100$. (a) The OCP bridge functions in the intermediate and long range $1.5 \leq x \leq 5$ as computed from the OZ inversion method with input from our accurate standard MD simulations versus the OCP bridge functions as calculated from the Iyetomi *et al.* parametrization. The error bars stem from the statistical uncertainties and correspond to 95% confidence intervals. (b) *Main.* The OCP bridge functions in the short range $0 \leq x \leq 1.5$ as computed from the cavity distribution method with input from specially designed long cavity MD simulations versus the OCP bridge functions as calculated from the Iyetomi *et al.* parametrization. The small error bars, that originate from the statistical uncertainties, correspond to 95% confidence intervals. *Inset.* The OCP screening potentials in the short range $0 \leq x \leq 1.5$ as computed from the cavity distribution method with input from specially designed long cavity MD simulations versus the OCP screening potentials as calculated from the Ogata parametrization. (c) The indirectly extracted OCP bridge functions (blue circles, downsampled) versus the analytically parameterized bridge functions (red solid lines). *Main.* The OCP bridge functions in the entire non-trivial interval $0 \leq x \leq 5.0$, where only the monotonic behavior of the short range is discernible. *Inset.* Zoom-in on the OCP bridge functions in the intermediate & long range interval $1.5 \leq x \leq 5.0$, where only the oscillatory decaying behavior is discernible.

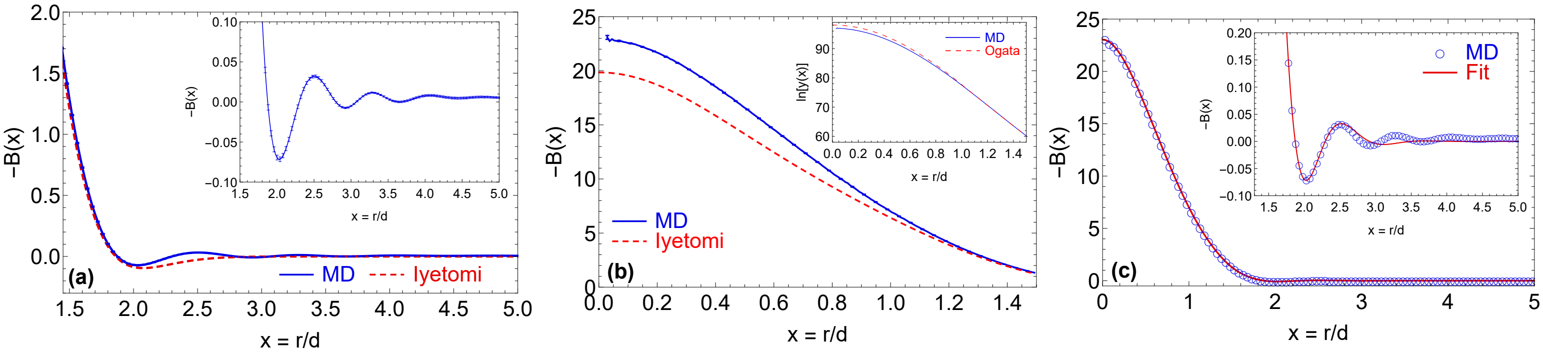


**Figure 9.** $\Gamma = 90$. (a) The OCP bridge functions in the intermediate and long range $1.5 \leq x \leq 5$ as computed from the OZ inversion method with input from our accurate standard MD simulations versus the OCP bridge functions as calculated from the Iyetomi *et al.* parametrization. The error bars stem from the statistical uncertainties and correspond to 95% confidence intervals. (b) *Main.* The OCP bridge functions in the short range $0 \leq x \leq 1.5$ as computed from the cavity distribution method with input from specially designed long cavity MD simulations versus the OCP bridge functions as calculated from the Iyetomi *et al.* parametrization. The small error bars, that originate from the statistical uncertainties, correspond to 95% confidence intervals. *Inset.* The OCP screening potentials in the short range $0 \leq x \leq 1.5$ as computed from the cavity distribution method with input from specially designed long cavity MD simulations versus the OCP screening potentials as calculated from the Ogata parametrization. (c) The indirectly extracted OCP bridge functions (blue circles, downsampled) versus the analytically parameterized bridge functions (red solid lines). *Main.* The OCP bridge functions in the entire non-trivial interval $0 \leq x \leq 5.0$, where only the monotonic behavior of the short range is discernible. *Inset.* Zoom-in on the OCP bridge functions in the intermediate & long range interval $1.5 \leq x \leq 5.0$, where only the oscillatory decaying behavior is discernible.

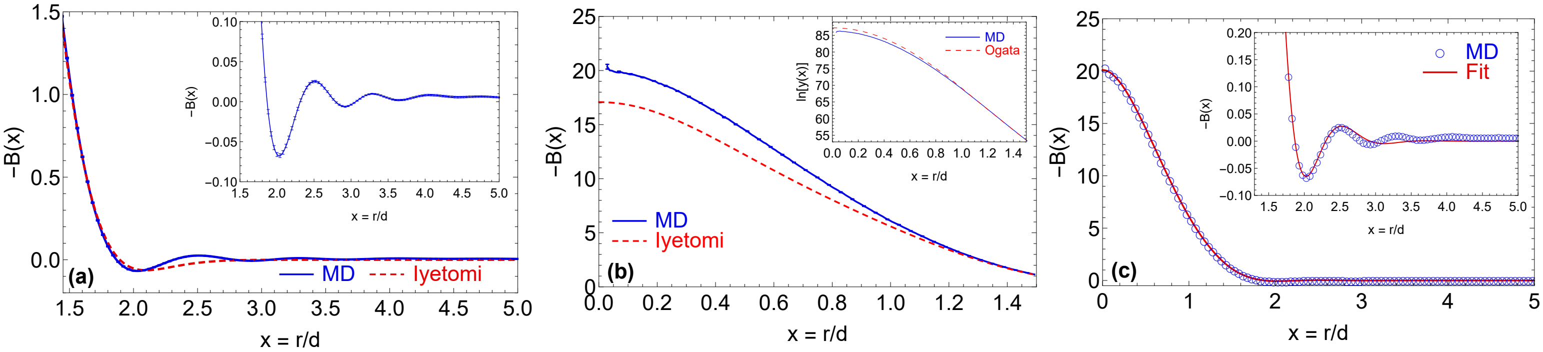


**Figure 10.** $\Gamma = 80$. (a) The OCP bridge functions in the intermediate and long range $1.5 \leq x \leq 5$ as computed from the OZ inversion method with input from our accurate standard MD simulations versus the OCP bridge functions as calculated from the Iyetomi *et al.* parametrization. The error bars stem from the statistical uncertainties and correspond to 95% confidence intervals. (b) *Main.* The OCP bridge functions in the short range $0 \leq x \leq 1.5$ as computed from the cavity distribution method with input from specially designed long cavity MD simulations versus the OCP bridge functions as calculated from the Iyetomi *et al.* parametrization. The small error bars, that originate from the statistical uncertainties, correspond to 95% confidence intervals. *Inset.* The OCP screening potentials in the short range $0 \leq x \leq 1.5$ as computed from the cavity distribution method with input from specially designed long cavity MD simulations versus the OCP screening potentials as calculated from the Ogata parametrization. (c) The indirectly extracted OCP bridge functions (blue circles, downsampled) versus the analytically parameterized bridge functions (red solid lines). *Main.* The OCP bridge functions in the entire non-trivial interval $0 \leq x \leq 5.0$, where only the monotonic behavior of the short range is discernible. *Inset.* Zoom-in on the OCP bridge functions in the intermediate & long range interval $1.5 \leq x \leq 5.0$, where only the oscillatory decaying behavior is discernible.

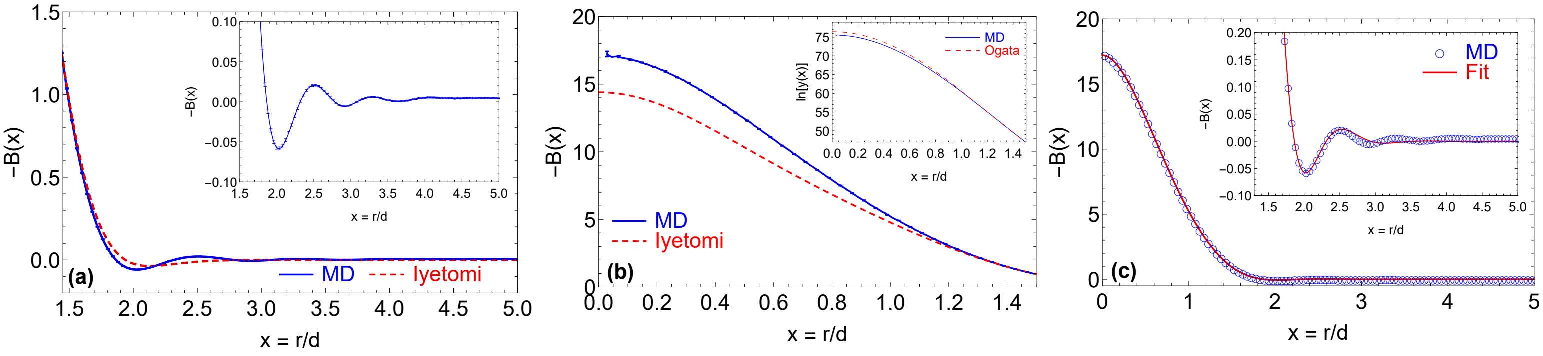


**Figure 11.** $\Gamma = 70$. (a) The OCP bridge functions in the intermediate and long range $1.5 \leq x \leq 5$ as computed from the OZ inversion method with input from our accurate standard MD simulations versus the OCP bridge functions as calculated from the Iyetomi *et al.* parametrization. The error bars stem from the statistical uncertainties and correspond to 95% confidence intervals. (b) *Main.* The OCP bridge functions in the short range $0 \leq x \leq 1.5$ as computed from the cavity distribution method with input from specially designed long cavity MD simulations versus the OCP bridge functions as calculated from the Iyetomi *et al.* parametrization. The small error bars, that originate from the statistical uncertainties, correspond to 95% confidence intervals. *Inset.* The OCP screening potentials in the short range $0 \leq x \leq 1.5$ as computed from the cavity distribution method with input from specially designed long cavity MD simulations versus the OCP screening potentials as calculated from the Ogata parametrization. (c) The indirectly extracted OCP bridge functions (blue circles, downsampled) versus the analytically parameterized bridge functions (red solid lines). *Main.* The OCP bridge functions in the entire non-trivial interval $0 \leq x \leq 5.0$, where only the monotonic behavior of the short range is discernible. *Inset.* Zoom-in on the OCP bridge functions in the intermediate & long range interval $1.5 \leq x \leq 5.0$, where only the oscillatory decaying behavior is discernible.

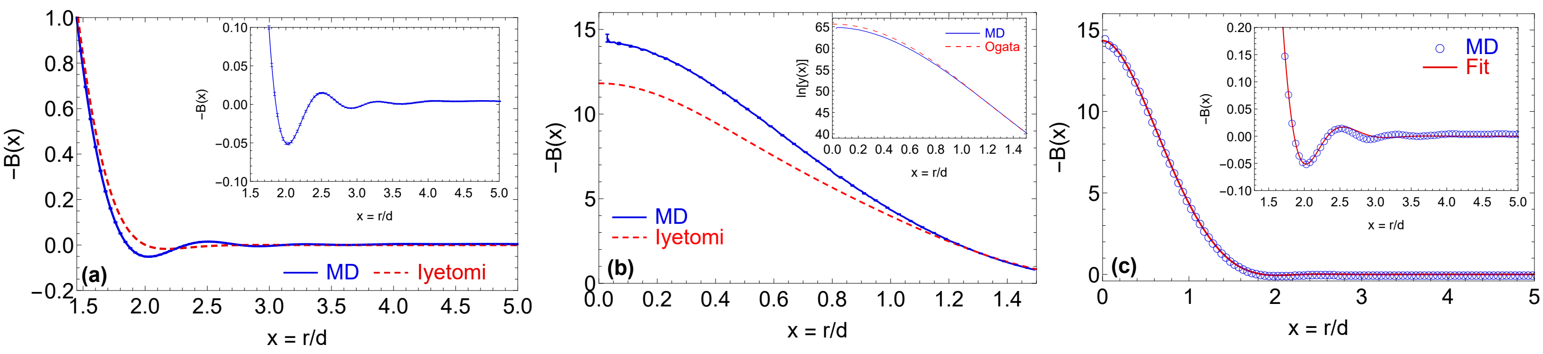


**Figure 12.** $\Gamma = 60$. (a) The OCP bridge functions in the intermediate and long range $1.5 \leq x \leq 5$ as computed from the OZ inversion method with input from our accurate standard MD simulations versus the OCP bridge functions as calculated from the Iyetomi *et al.* parametrization. The error bars stem from the statistical uncertainties and correspond to 95% confidence intervals. (b) *Main.* The OCP bridge functions in the short range $0 \leq x \leq 1.5$ as computed from the cavity distribution method with input from specially designed long cavity MD simulations versus the OCP bridge functions as calculated from the Iyetomi *et al.* parametrization. The small error bars, that originate from the statistical uncertainties, correspond to 95% confidence intervals. *Inset.* The OCP screening potentials in the short range $0 \leq x \leq 1.5$ as computed from the cavity distribution method with input from specially designed long cavity MD simulations versus the OCP screening potentials as calculated from the Ogata parametrization. (c) The indirectly extracted OCP bridge functions (blue circles, downsampled) versus the analytically parameterized bridge functions (red solid lines). *Main.* The OCP bridge functions in the entire non-trivial interval $0 \leq x \leq 5.0$, where only the monotonic behavior of the short range is discernible. *Inset.* Zoom-in on the OCP bridge functions in the intermediate & long range interval $1.5 \leq x \leq 5.0$, where only the oscillatory decaying behavior is discernible.

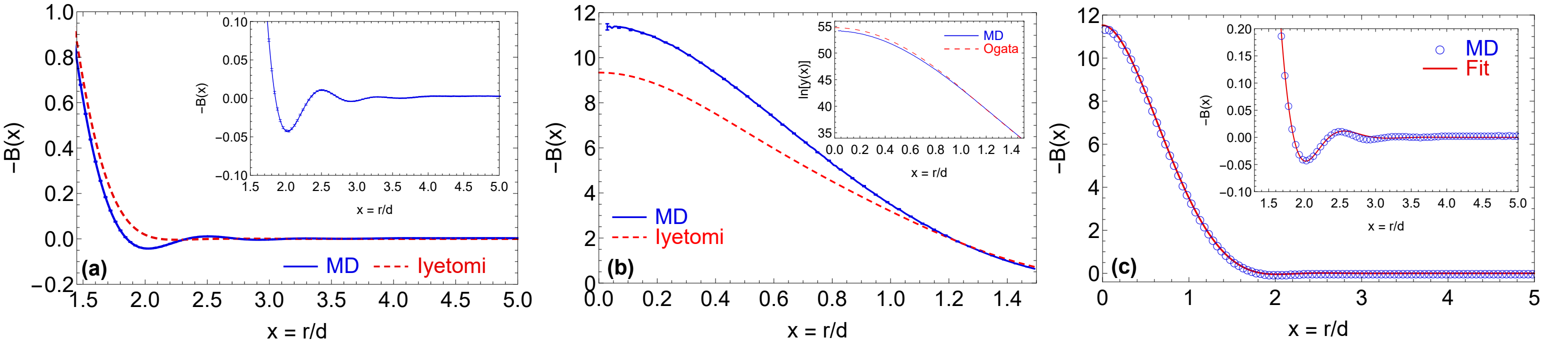


**Figure 13.** $\Gamma = 50$. (a) The OCP bridge functions in the intermediate and long range $1.5 \leq x \leq 5$ as computed from the OZ inversion method with input from our accurate standard MD simulations versus the OCP bridge functions as calculated from the Iyetomi *et al.* parametrization. The error bars stem from the statistical uncertainties and correspond to 95% confidence intervals. (b) *Main.* The OCP bridge functions in the short range $0 \leq x \leq 1.5$ as computed from the cavity distribution method with input from specially designed long cavity MD simulations versus the OCP bridge functions as calculated from the Iyetomi *et al.* parametrization. The small error bars, that originate from the statistical uncertainties, correspond to 95% confidence intervals. *Inset.* The OCP screening potentials in the short range $0 \leq x \leq 1.5$ as computed from the cavity distribution method with input from specially designed long cavity MD simulations versus the OCP screening potentials as calculated from the Ogata parametrization. (c) The indirectly extracted OCP bridge functions (blue circles, downsampled) versus the analytically parameterized bridge functions (red solid lines). *Main.* The OCP bridge functions in the entire non-trivial interval $0 \leq x \leq 5.0$, where only the monotonic behavior of the short range is discernible. *Inset.* Zoom-in on the OCP bridge functions in the intermediate & long range interval $1.5 \leq x \leq 5.0$, where only the oscillatory decaying behavior is discernible.

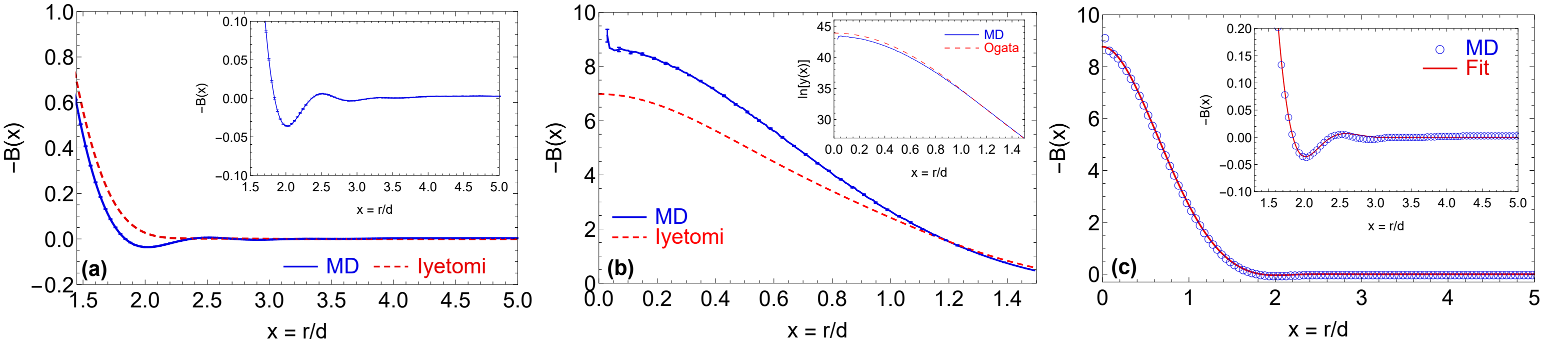


**Figure 14.** $\Gamma = 40$. (a) The OCP bridge functions in the intermediate and long range $1.5 \leq x \leq 5$ as computed from the OZ inversion method with input from our accurate standard MD simulations versus the OCP bridge functions as calculated from the Iyetomi *et al.* parametrization. The error bars stem from the statistical uncertainties and correspond to 95% confidence intervals. (b) *Main.* The OCP bridge functions in the short range $0 \leq x \leq 1.5$ as computed from the cavity distribution method with input from specially designed long cavity MD simulations versus the OCP bridge functions as calculated from the Iyetomi *et al.* parametrization. The small error bars, that originate from the statistical uncertainties, correspond to 95% confidence intervals. *Inset.* The OCP screening potentials in the short range $0 \leq x \leq 1.5$ as computed from the cavity distribution method with input from specially designed long cavity MD simulations versus the OCP screening potentials as calculated from the Ogata parametrization. (c) The indirectly extracted OCP bridge functions (blue circles, downsampled) versus the analytically parameterized bridge functions (red solid lines). *Main.* The OCP bridge functions in the entire non-trivial interval $0 \leq x \leq 5.0$, where only the monotonic behavior of the short range is discernible. *Inset.* Zoom-in on the OCP bridge functions in the intermediate & long range interval $1.5 \leq x \leq 5.0$, where only the oscillatory decaying behavior is discernible.

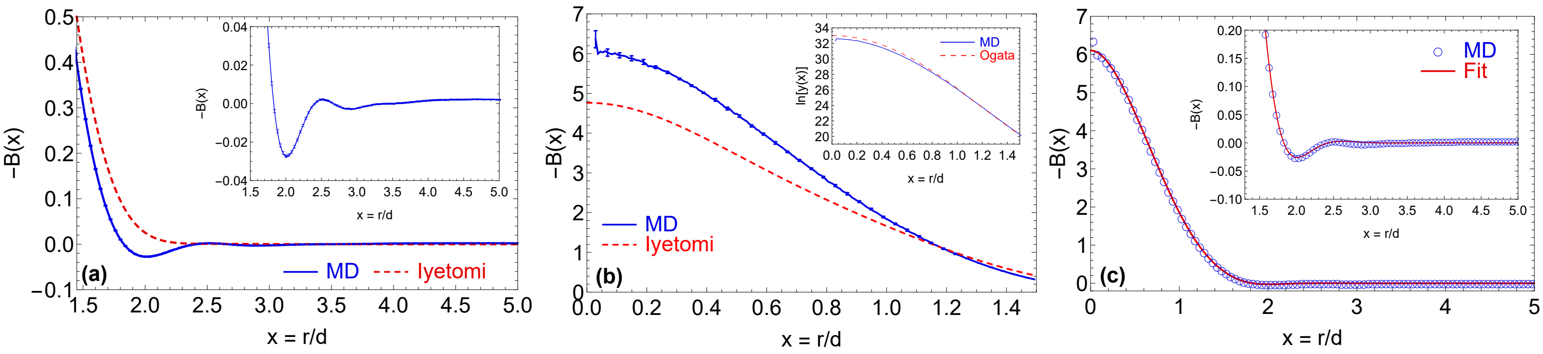


**Figure 15.** $\Gamma = 30$. (a) The OCP bridge functions in the intermediate and long range $1.5 \leq x \leq 5$ as computed from the OZ inversion method with input from our accurate standard MD simulations versus the OCP bridge functions as calculated from the Iyetomi *et al.* parametrization. The error bars stem from the statistical uncertainties and correspond to 95% confidence intervals. (b) *Main.* The OCP bridge functions in the short range $0 \leq x \leq 1.5$ as computed from the cavity distribution method with input from specially designed long cavity MD simulations versus the OCP bridge functions as calculated from the Iyetomi *et al.* parametrization. The small error bars, that originate from the statistical uncertainties, correspond to 95% confidence intervals. *Inset.* The OCP screening potentials in the short range $0 \leq x \leq 1.5$ as computed from the cavity distribution method with input from specially designed long cavity MD simulations versus the OCP screening potentials as calculated from the Ogata parametrization. (c) The indirectly extracted OCP bridge functions (blue circles, downsampled) versus the analytically parameterized bridge functions (red solid lines). *Main.* The OCP bridge functions in the entire non-trivial interval $0 \leq x \leq 5.0$, where only the monotonic behavior of the short range is discernible. *Inset.* Zoom-in on the OCP bridge functions in the intermediate & long range interval $1.5 \leq x \leq 5.0$, where only the oscillatory decaying behavior is discernible.

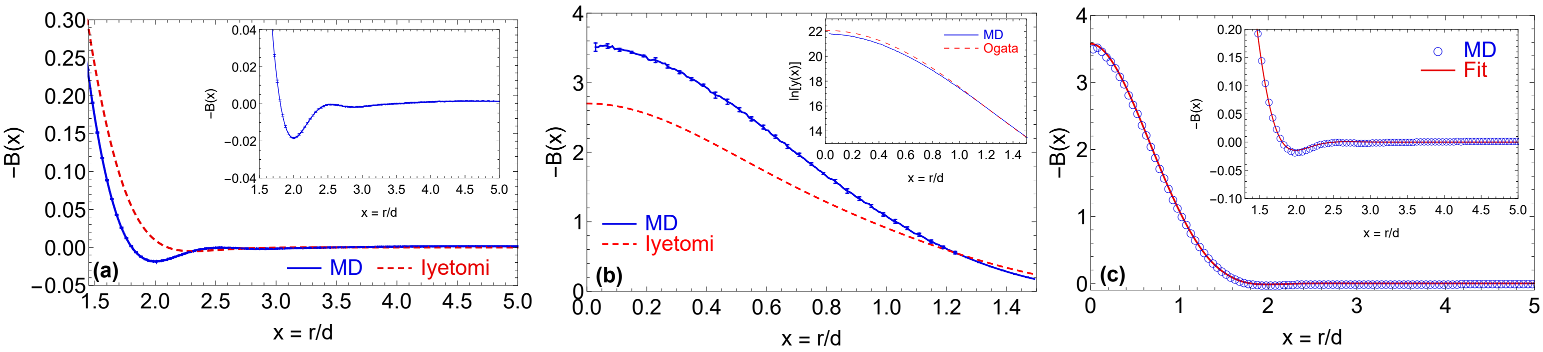


**Figure 16.** $\Gamma = 20$. (a) The OCP bridge functions in the intermediate and long range $1.5 \leq x \leq 5$ as computed from the OZ inversion method with input from our accurate standard MD simulations versus the OCP bridge functions as calculated from the Iyetomi *et al.* parametrization. The error bars stem from the statistical uncertainties and correspond to 95% confidence intervals. (b) *Main.* The OCP bridge functions in the short range $0 \leq x \leq 1.5$ as computed from the cavity distribution method with input from specially designed long cavity MD simulations versus the OCP bridge functions as calculated from the Iyetomi *et al.* parametrization. The small error bars, that originate from the statistical uncertainties, correspond to 95% confidence intervals. *Inset.* The OCP screening potentials in the short range $0 \leq x \leq 1.5$ as computed from the cavity distribution method with input from specially designed long cavity MD simulations versus the OCP screening potentials as calculated from the Ogata parametrization. (c) The indirectly extracted OCP bridge functions (blue circles, downsampled) versus the analytically parameterized bridge functions (red solid lines). *Main.* The OCP bridge functions in the entire non-trivial interval $0 \leq x \leq 5.0$, where only the monotonic behavior of the short range is discernible. *Inset.* Zoom-in on the OCP bridge functions in the intermediate & long range interval $1.5 \leq x \leq 5.0$, where only the oscillatory decaying behavior is discernible.

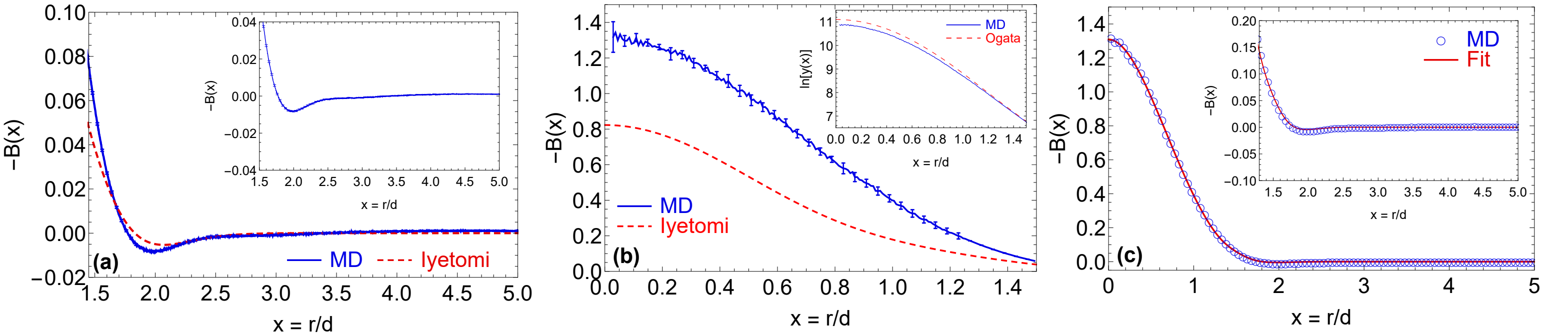


**Figure 17.** $\Gamma = 10$. (a) The OCP bridge functions in the intermediate and long range $1.5 \leq x \leq 5$ as computed from the OZ inversion method with input from our accurate standard MD simulations versus the OCP bridge functions as calculated from the Iyetomi *et al.* parametrization. The error bars stem from the statistical uncertainties and correspond to 95% confidence intervals. (b) *Main.* The OCP bridge functions in the short range $0 \leq x \leq 1.5$ as computed from the cavity distribution method with input from specially designed long cavity MD simulations versus the OCP bridge functions as calculated from the Iyetomi *et al.* parametrization. The small error bars, that originate from the statistical uncertainties, correspond to 95% confidence intervals. *Inset.* The OCP screening potentials in the short range $0 \leq x \leq 1.5$ as computed from the cavity distribution method with input from specially designed long cavity MD simulations versus the OCP screening potentials as calculated from the Ogata parametrization. (c) The indirectly extracted OCP bridge functions (blue circles, downsampled) versus the analytically parameterized bridge functions (red solid lines). *Main.* The OCP bridge functions in the entire non-trivial interval $0 \leq x \leq 5.0$, where only the monotonic behavior of the short range is discernible. *Inset.* Zoom-in on the OCP bridge functions in the intermediate & long range interval $1.5 \leq x \leq 5.0$, where only the oscillatory decaying behavior is discernible.

# Contents of the second part

**Tables 1a-1c**: Key figures of merit of the radial distribution function, results for $\mathbf{arg}_r\{g(r) = 0.5\}$. Each table contains the results for one value of the screening parameter belonging to the set $\kappa = \{0.0, 1.0, 2.0\}$.

**Tables 2a-2c**: Key figures of merit of the radial distribution function, results for the magnitude of the first maximum. Each table contains the results for one value of the screening parameter belonging to the set $\kappa = \{0.0, 1.0, 2.0\}$.

**Tables 3a-3c**: Key figures of merit of the radial distribution function, results for the position of the first maximum. Each table contains the results for one value of the screening parameter belonging to the set $\kappa = \{0.0, 1.0, 2.0\}$.

**Tables 4a-4c**: Key figures of merit of the radial distribution function, results for the magnitude of the first non-zero minimum. Each table contains the results for one value of the screening parameter belonging to the set $\kappa = \{0.0, 1.0, 2.0\}$.

**Tables 5a-5c**: Key figures of merit of the radial distribution function, results for the position of the first non-zero minimum. Each table contains the results for one value of the screening parameter belonging to the set $\kappa = \{0.0, 1.0, 2.0\}$.

**Tables 6a-6c**: Key figures of merit of the radial distribution function, results for the magnitude of the second maximum. Each table contains the results for one value of the screening parameter belonging to the set $\kappa = \{0.0, 1.0, 2.0\}$.

**Tables 7a-7c**: Key figures of merit of the radial distribution function, results for the position of the second maximum. Each table contains the results for one value of the screening parameter belonging to the set $\kappa = \{0.0, 1.0, 2.0\}$.

**Tables 8a-8o**: Reduced excess internal energy. Each table contains the results for one value of the screening parameter belonging to $\kappa = \{0.0, 0.2, 0.4, 0.6, 0.8, 1.0, 1.2, 1.4, 2.0, 2.6, 3.0, 3.6, 4.0, 4.6, 5.0\}$.

**Table 1a.** Key properties of the radial distribution function resulting from molecular dynamics (MD) simulations and from two versions of the isomorph-based empirically modified hypernetted chain (IEMHNC) approach: the version constructed with the OCP bridge function given by Iyetomi, Ogata and Ichimaru (IOI) in *H. Iyetomi, S. Ogata and S. Ichimaru, Phys. Rev. A* **46**, *1051 (1992)* and the version constructed with the new OCP bridge function parameterization proposed by the authors (LCT). The absolute relative deviation $\epsilon_{\mathrm{r}}$ between the theoretical and the simulation results is also reported together with its average and maximum values (the average deviation is denoted as $\epsilon_{\mathrm{AVE}}$ and the maximum deviation is denoted as $\epsilon_{\mathrm{MAX}}$). **Results for $\mathbf{arg}_r\{g(r)=0.5\}$ in the case of $\kappa=0.0$**. The MD results are adopted from *T. Ott and M. Bonitz, Contrib. Plasma Phys.* **55**, *243 (2015)*. Here $x=r/d$, where $d$ is the Wigner-Seitz radius.

| $\Gamma$ | $\Gamma/\Gamma_m$ | $x_{\mathrm{cv}}^{\mathrm{MD}}$ | $x_{\mathrm{cv}}^{\mathrm{IOI}}$ | $\epsilon_{\mathrm{IOI}}(\%)$ | $x_{\mathrm{cv}}^{\mathrm{LCT}}$ | $\epsilon_{\mathrm{LCT}}(\%)$ |
|---|---|---|---|---|---|---|
| 15.0 | 0.09 | 1.179 | 1.165 | 1.187 | 1.178 | 0.085 |
| 20.0 | 0.12 | 1.218 | 1.207 | 0.903 | 1.217 | 0.082 |
| 25.0 | 0.15 | 1.246 | 1.237 | 0.722 | 1.245 | 0.080 |
| 30.0 | 0.17 | 1.272 | 1.262 | 0.786 | 1.268 | 0.314 |
| 35.0 | 0.20 | 1.291 | 1.282 | 0.697 | 1.288 | 0.232 |
| 40.0 | 0.23 | 1.307 | 1.299 | 0.612 | 1.304 | 0.230 |
| 45.0 | 0.26 | 1.320 | 1.314 | 0.455 | 1.319 | 0.076 |
| 50.0 | 0.29 | 1.333 | 1.327 | 0.450 | 1.332 | 0.075 |
| 55.0 | 0.32 | 1.346 | 1.338 | 0.594 | 1.343 | 0.223 |
| 60.0 | 0.35 | 1.355 | 1.349 | 0.443 | 1.354 | 0.074 |
| 65.0 | 0.38 | 1.365 | 1.359 | 0.440 | 1.363 | 0.147 |
| 70.0 | 0.41 | 1.374 | 1.367 | 0.509 | 1.372 | 0.146 |
| 75.0 | 0.44 | 1.381 | 1.376 | 0.362 | 1.380 | 0.072 |
| 80.0 | 0.47 | 1.387 | 1.383 | 0.288 | 1.387 | 0.000 |
| 85.0 | 0.49 | 1.394 | 1.390 | 0.287 | 1.394 | 0.000 |
| 90.0 | 0.52 | 1.400 | 1.397 | 0.214 | 1.401 | 0.071 |
| 95.0 | 0.55 | 1.406 | 1.403 | 0.213 | 1.407 | 0.071 |
| 100.0 | 0.58 | 1.413 | 1.409 | 0.283 | 1.412 | 0.071 |
| 105.0 | 0.61 | 1.419 | 1.415 | 0.282 | 1.418 | 0.070 |
| 110.0 | 0.64 | 1.422 | 1.420 | 0.141 | 1.423 | 0.070 |
| 115.0 | 0.67 | 1.429 | 1.425 | 0.280 | 1.428 | 0.070 |
| 120.0 | 0.70 | 1.432 | 1.430 | 0.140 | 1.432 | 0.000 |
| 125.0 | 0.73 | 1.435 | 1.434 | 0.070 | 1.437 | 0.139 |
| 130.0 | 0.76 | 1.442 | 1.439 | 0.208 | 1.441 | 0.069 |
| 135.0 | 0.79 | 1.445 | 1.443 | 0.138 | 1.445 | 0.000 |
| 140.0 | 0.81 | 1.448 | 1.447 | 0.069 | 1.449 | 0.069 |
| 145.0 | 0.84 | 1.451 | 1.451 | 0.000 | 1.452 | 0.069 |
| 150.0 | 0.87 | 1.454 | 1.455 | 0.069 | 1.456 | 0.138 |
| 155.0 | 0.90 | 1.461 | 1.458 | 0.205 | 1.459 | 0.137 |
| 160.0 | 0.93 | 1.464 | 1.462 | 0.137 | 1.462 | 0.137 |
| 165.0 | 0.96 | 1.467 | 1.465 | 0.136 | 1.465 | 0.136 |
| $\boldsymbol{\epsilon}_{\mathbf{AVE}}(\%)$ | | | | **0.365** | | **0.102** |
| $\boldsymbol{\epsilon}_{\mathbf{MAX}}(\%)$ | | | | **1.187** | | **0.314** |

**Table 1b.** Key properties of the radial distribution function resulting from molecular dynamics (MD) simulations and from two versions of the isomorph-based empirically modified hypernetted chain (IEMHNC) approach: the version constructed with the OCP bridge function given by Iyetomi, Ogata and Ichimaru (IOI) in *H. Iyetomi, S. Ogata and S. Ichimaru, Phys. Rev. A* **46**, *1051 (1992)* and the version constructed with the new OCP bridge function parameterization proposed by the authors (LCT). The absolute relative deviation $\epsilon_{\mathrm{r}}$ between the theoretical and the simulation results is also reported together with its average and maximum values (the average deviation is denoted as $\epsilon_{\mathrm{AVE}}$ and the maximum deviation is denoted as $\epsilon_{\mathrm{MAX}}$). **Results for $\arg_r\{g(r)=0.5\}$ in the case of $\kappa=1.0$**. The MD results are adopted from *T. Ott and M. Bonitz, Contrib. Plasma Phys.* **55**, *243 (2015)*. Here $x=r/d$, where $d$ is the Wigner-Seitz radius.

| $\Gamma$ | $\Gamma/\Gamma_m$ | $x_{\mathrm{cv}}^{\mathrm{MD}}$ | $x_{\mathrm{cv}}^{\mathrm{IOI}}$ | $\epsilon_{\mathrm{IOI}}(\%)$ | $x_{\mathrm{cv}}^{\mathrm{LCT}}$ | $\epsilon_{\mathrm{LCT}}(\%)$ |
|---|---|---|---|---|---|---|
| 10.0 | 0.05 | 1.076 | 1.057 | 1.766 | 1.071 | 0.465 |
| 15.0 | 0.07 | 1.139 | 1.124 | 1.317 | 1.137 | 0.176 |
| 20.0 | 0.09 | 1.177 | 1.168 | 0.765 | 1.180 | 0.255 |
| 25.0 | 0.11 | 1.211 | 1.200 | 0.908 | 1.211 | 0.000 |
| 30.0 | 0.14 | 1.237 | 1.226 | 0.889 | 1.235 | 0.162 |
| 35.0 | 0.16 | 1.254 | 1.247 | 0.558 | 1.255 | 0.080 |
| 40.0 | 0.18 | 1.275 | 1.265 | 0.784 | 1.272 | 0.235 |
| 45.0 | 0.20 | 1.288 | 1.281 | 0.543 | 1.287 | 0.078 |
| 50.0 | 0.23 | 1.301 | 1.295 | 0.461 | 1.300 | 0.077 |
| 55.0 | 0.25 | 1.313 | 1.307 | 0.457 | 1.312 | 0.076 |
| 60.0 | 0.27 | 1.326 | 1.318 | 0.603 | 1.323 | 0.226 |
| 65.0 | 0.30 | 1.334 | 1.328 | 0.450 | 1.333 | 0.075 |
| 70.0 | 0.32 | 1.343 | 1.337 | 0.447 | 1.342 | 0.074 |
| 75.0 | 0.34 | 1.351 | 1.346 | 0.370 | 1.351 | 0.000 |
| 80.0 | 0.36 | 1.360 | 1.354 | 0.441 | 1.358 | 0.147 |
| 85.0 | 0.39 | 1.364 | 1.361 | 0.220 | 1.366 | 0.147 |
| 90.0 | 0.41 | 1.373 | 1.368 | 0.364 | 1.372 | 0.073 |
| 95.0 | 0.43 | 1.377 | 1.374 | 0.218 | 1.379 | 0.145 |
| 100.0 | 0.45 | 1.385 | 1.381 | 0.289 | 1.385 | 0.000 |
| 105.0 | 0.48 | 1.390 | 1.386 | 0.288 | 1.390 | 0.000 |
| 110.0 | 0.50 | 1.394 | 1.392 | 0.143 | 1.396 | 0.143 |
| 115.0 | 0.52 | 1.402 | 1.397 | 0.357 | 1.401 | 0.071 |
| 120.0 | 0.54 | 1.407 | 1.402 | 0.355 | 1.406 | 0.071 |
| 125.0 | 0.57 | 1.411 | 1.407 | 0.283 | 1.410 | 0.071 |
| 130.0 | 0.59 | 1.415 | 1.411 | 0.283 | 1.414 | 0.071 |
| 135.0 | 0.61 | 1.419 | 1.416 | 0.211 | 1.419 | 0.000 |
| 140.0 | 0.64 | 1.424 | 1.420 | 0.281 | 1.423 | 0.070 |
| 145.0 | 0.66 | 1.428 | 1.424 | 0.280 | 1.427 | 0.070 |
| 150.0 | 0.68 | 1.428 | 1.428 | 0.000 | 1.430 | 0.140 |
| 155.0 | 0.70 | 1.432 | 1.431 | 0.070 | 1.434 | 0.140 |
| 160.0 | 0.73 | 1.436 | 1.435 | 0.070 | 1.437 | 0.070 |
| 165.0 | 0.75 | 1.441 | 1.438 | 0.208 | 1.440 | 0.069 |
| 170.0 | 0.77 | 1.445 | 1.442 | 0.208 | 1.444 | 0.069 |
| 175.0 | 0.79 | 1.445 | 1.445 | 0.000 | 1.447 | 0.138 |
| 180.0 | 0.82 | 1.449 | 1.448 | 0.069 | 1.450 | 0.069 |
| 185.0 | 0.84 | 1.453 | 1.451 | 0.138 | 1.453 | 0.000 |
| 190.0 | 0.86 | 1.453 | 1.454 | 0.069 | 1.455 | 0.138 |
| 195.0 | 0.89 | 1.458 | 1.457 | 0.069 | 1.458 | 0.000 |
| 200.0 | 0.91 | 1.462 | 1.460 | 0.137 | 1.461 | 0.068 |
| $\boldsymbol{\epsilon_{\mathrm{AVE}}(\%)}$ | | | | **0.394** | | **0.102** |
| $\boldsymbol{\epsilon_{\mathrm{MAX}}(\%)}$ | | | | **1.766** | | **0.465** |

**Table 1c.** Key properties of the radial distribution function resulting from molecular dynamics (MD) simulations and from two versions of the isomorph-based empirically modified hypernetted chain (IEMHNC) approach: the version constructed with the OCP bridge function given by Iyetomi, Ogata and Ichimaru (IOI) in *H. Iyetomi, S. Ogata and S. Ichimaru, Phys. Rev. A* **46**, *1051 (1992)* and the version constructed with the new OCP bridge function parameterization proposed by the authors (LCT). The absolute relative deviation $\epsilon_{\mathrm{r}}$ between the theoretical and the simulation results is also reported together with its average and maximum values (the average deviation is denoted as $\epsilon_{\mathrm{AVE}}$ and the maximum deviation is denoted as $\epsilon_{\mathrm{MAX}}$). **Results for $\arg_r\{g(r)=0.5\}$ in the case of $\kappa=2.0$**. The MD results are adopted from *T. Ott and M. Bonitz, Contrib. Plasma Phys.* **55**, *243 (2015)*. Here $x=r/d$, where $d$ is the Wigner-Seitz radius.

| $\Gamma$ | $\Gamma/\Gamma_m$ | $x_{\mathrm{cv}}^{\mathrm{MD}}$ | $x_{\mathrm{cv}}^{\mathrm{IOI}}$ | $\epsilon_{\mathrm{IOI}}(\%)$ | $x_{\mathrm{cv}}^{\mathrm{LCT}}$ | $\epsilon_{\mathrm{LCT}}(\%)$ |
|---|---|---|---|---|---|---|
| 30.0 | 0.07 | 1.135 | 1.123 | 1.057 | 1.135 | 0.000 |
| 40.0 | 0.09 | 1.176 | 1.167 | 0.765 | 1.178 | 0.170 |
| 50.0 | 0.11 | 1.209 | 1.200 | 0.744 | 1.209 | 0.000 |
| 60.0 | 0.13 | 1.234 | 1.226 | 0.648 | 1.234 | 0.000 |
| 70.0 | 0.15 | 1.254 | 1.247 | 0.558 | 1.254 | 0.000 |
| 80.0 | 0.17 | 1.272 | 1.266 | 0.472 | 1.272 | 0.000 |
| 90.0 | 0.20 | 1.288 | 1.281 | 0.543 | 1.287 | 0.078 |
| 100.0 | 0.22 | 1.301 | 1.295 | 0.461 | 1.300 | 0.077 |
| 110.0 | 0.24 | 1.313 | 1.308 | 0.381 | 1.312 | 0.076 |
| 120.0 | 0.26 | 1.324 | 1.319 | 0.378 | 1.323 | 0.076 |
| 130.0 | 0.28 | 1.333 | 1.329 | 0.300 | 1.334 | 0.075 |
| 140.0 | 0.31 | 1.342 | 1.338 | 0.298 | 1.343 | 0.075 |
| 150.0 | 0.33 | 1.351 | 1.347 | 0.296 | 1.351 | 0.000 |
| 160.0 | 0.35 | 1.358 | 1.355 | 0.221 | 1.359 | 0.074 |
| 170.0 | 0.37 | 1.366 | 1.362 | 0.293 | 1.366 | 0.000 |
| 180.0 | 0.39 | 1.373 | 1.369 | 0.291 | 1.373 | 0.000 |
| 190.0 | 0.41 | 1.378 | 1.376 | 0.145 | 1.380 | 0.145 |
| 200.0 | 0.44 | 1.384 | 1.382 | 0.145 | 1.386 | 0.145 |
| 210.0 | 0.46 | 1.389 | 1.388 | 0.072 | 1.391 | 0.144 |
| 220.0 | 0.48 | 1.396 | 1.393 | 0.215 | 1.397 | 0.072 |
| 230.0 | 0.50 | 1.400 | 1.398 | 0.143 | 1.402 | 0.143 |
| 240.0 | 0.52 | 1.405 | 1.403 | 0.142 | 1.407 | 0.142 |
| 250.0 | 0.55 | 1.409 | 1.408 | 0.071 | 1.411 | 0.142 |
| 260.0 | 0.57 | 1.414 | 1.413 | 0.071 | 1.416 | 0.141 |
| 270.0 | 0.59 | 1.418 | 1.417 | 0.071 | 1.420 | 0.141 |
| 280.0 | 0.61 | 1.423 | 1.421 | 0.141 | 1.424 | 0.070 |
| 290.0 | 0.63 | 1.427 | 1.425 | 0.140 | 1.428 | 0.070 |
| 300.0 | 0.65 | 1.429 | 1.429 | 0.000 | 1.432 | 0.210 |
| 310.0 | 0.68 | 1.434 | 1.433 | 0.070 | 1.435 | 0.070 |
| 320.0 | 0.70 | 1.436 | 1.436 | 0.000 | 1.439 | 0.209 |
| 330.0 | 0.72 | 1.441 | 1.440 | 0.069 | 1.442 | 0.069 |
| 340.0 | 0.74 | 1.443 | 1.443 | 0.000 | 1.445 | 0.139 |
| 350.0 | 0.76 | 1.447 | 1.447 | 0.000 | 1.448 | 0.069 |
| 360.0 | 0.79 | 1.450 | 1.450 | 0.000 | 1.451 | 0.069 |
| 370.0 | 0.81 | 1.452 | 1.453 | 0.069 | 1.454 | 0.138 |
| 380.0 | 0.83 | 1.456 | 1.456 | 0.000 | 1.457 | 0.069 |
| 390.0 | 0.85 | 1.459 | 1.459 | 0.000 | 1.460 | 0.069 |
| 400.0 | 0.87 | 1.461 | 1.461 | 0.000 | 1.462 | 0.068 |
| $\boldsymbol{\epsilon_{\mathrm{AVE}}(\%)}$ | | | | **0.244** | | **0.085** |
| $\boldsymbol{\epsilon_{\mathrm{MAX}}(\%)}$ | | | | **1.057** | | **0.210** |

**Table 2a.** Key properties of the radial distribution function resulting from molecular dynamics (MD) simulations and from two versions of the isomorph-based empirically modified hypernetted chain (IEMHNC) approach: the version constructed with the OCP bridge function given by Iyetomi, Ogata and Ichimaru (IOI) in *H. Iyetomi, S. Ogata and S. Ichimaru, Phys. Rev. A* **46**, *1051 (1992)* and the version constructed with the new OCP bridge function parameterization proposed by the authors (LCT). The absolute relative deviation $\epsilon_{\mathrm{r}}$ between the theoretical and the simulation results is also reported together with its average and maximum values (the average deviation is denoted as $\epsilon_{\mathrm{AVE}}$ and the maximum deviation is denoted as $\epsilon_{\mathrm{MAX}}$). **Results for the magnitude of the first maximum in the case of $\boldsymbol{\kappa = 0.0}$.** The MD results are adopted from *T. Ott and M. Bonitz, Contrib. Plasma Phys.* **55**, *243 (2015)*.

| $\Gamma$ | $\Gamma/\Gamma_m$ | $g_{\mathrm{max1}}^{\mathrm{MD}}$ | $g_{\mathrm{max1}}^{\mathrm{IOI}}$ | $\epsilon_{\mathrm{IOI}}(\%)$ | $g_{\mathrm{max1}}^{\mathrm{LCT}}$ | $\epsilon_{\mathrm{LCT}}(\%)$ |
|---|---|---|---|---|---|---|
| 15.0 | 0.09 | 1.228 | 1.200 | 2.269 | 1.227 | 0.045 |
| 20.0 | 0.12 | 1.307 | 1.277 | 2.330 | 1.307 | 0.030 |
| 25.0 | 0.15 | 1.378 | 1.348 | 2.204 | 1.378 | 0.011 |
| 30.0 | 0.17 | 1.443 | 1.414 | 2.041 | 1.442 | 0.046 |
| 35.0 | 0.20 | 1.504 | 1.475 | 1.931 | 1.502 | 0.152 |
| 40.0 | 0.23 | 1.560 | 1.533 | 1.759 | 1.557 | 0.163 |
| 45.0 | 0.26 | 1.614 | 1.587 | 1.677 | 1.610 | 0.231 |
| 50.0 | 0.29 | 1.664 | 1.639 | 1.528 | 1.661 | 0.205 |
| 55.0 | 0.32 | 1.712 | 1.688 | 1.410 | 1.709 | 0.191 |
| 60.0 | 0.35 | 1.757 | 1.735 | 1.246 | 1.755 | 0.118 |
| 65.0 | 0.38 | 1.803 | 1.781 | 1.244 | 1.799 | 0.201 |
| 70.0 | 0.41 | 1.845 | 1.824 | 1.113 | 1.842 | 0.149 |
| 75.0 | 0.44 | 1.885 | 1.867 | 0.957 | 1.884 | 0.070 |
| 80.0 | 0.47 | 1.926 | 1.908 | 0.926 | 1.924 | 0.113 |
| 85.0 | 0.49 | 1.964 | 1.948 | 0.802 | 1.963 | 0.063 |
| 90.0 | 0.52 | 2.001 | 1.987 | 0.686 | 2.001 | 0.019 |
| 95.0 | 0.55 | 2.037 | 2.025 | 0.573 | 2.037 | 0.024 |
| 100.0 | 0.58 | 2.072 | 2.063 | 0.457 | 2.073 | 0.067 |
| 105.0 | 0.61 | 2.107 | 2.099 | 0.385 | 2.108 | 0.067 |
| 110.0 | 0.64 | 2.140 | 2.134 | 0.258 | 2.143 | 0.121 |
| 115.0 | 0.67 | 2.174 | 2.169 | 0.213 | 2.176 | 0.090 |
| 120.0 | 0.70 | 2.206 | 2.204 | 0.110 | 2.209 | 0.114 |
| 125.0 | 0.73 | 2.237 | 2.237 | 0.008 | 2.240 | 0.149 |
| 130.0 | 0.76 | 2.270 | 2.270 | 0.007 | 2.271 | 0.061 |
| 135.0 | 0.79 | 2.298 | 2.303 | 0.199 | 2.302 | 0.160 |
| 140.0 | 0.81 | 2.329 | 2.334 | 0.234 | 2.331 | 0.097 |
| 145.0 | 0.84 | 2.358 | 2.366 | 0.331 | 2.360 | 0.088 |
| 150.0 | 0.87 | 2.386 | 2.397 | 0.448 | 2.388 | 0.091 |
| 155.0 | 0.90 | 2.413 | 2.427 | 0.584 | 2.416 | 0.105 |
| 160.0 | 0.93 | 2.442 | 2.457 | 0.616 | 2.442 | 0.007 |
| 165.0 | 0.96 | 2.470 | 2.487 | 0.670 | 2.468 | 0.077 |
| $\boldsymbol{\epsilon_{\mathrm{AVE}}}$**(%)** | | | | **0.942** | | **0.101** |
| $\boldsymbol{\epsilon_{\mathrm{MAX}}}$**(%)** | | | | **2.330** | | **0.231** |

**Table 2b.** Key properties of the radial distribution function resulting from molecular dynamics (MD) simulations and from two versions of the isomorph-based empirically modified hypernetted chain (IEMHNC) approach: the version constructed with the OCP bridge function given by Iyetomi, Ogata and Ichimaru (IOI) in *H. Iyetomi, S. Ogata and S. Ichimaru, Phys. Rev. A* **46**, *1051 (1992)* and the version constructed with the new OCP bridge function parameterization proposed by the authors (LCT). The absolute relative deviation $\epsilon_{\mathrm{r}}$ between the theoretical and the simulation results is also reported together with its average and maximum values (the average deviation is denoted as $\epsilon_{\mathrm{AVE}}$ and the maximum deviation is denoted as $\epsilon_{\mathrm{MAX}}$). **Results for the magnitude of the first maximum in the case of $\boldsymbol{\kappa = 1.0}$.** The MD results are adopted from *T. Ott and M. Bonitz, Contrib. Plasma Phys.* **55**, *243 (2015)*.

| $\Gamma$ | $\Gamma/\Gamma_m$ | $g_{\mathrm{max1}}^{\mathrm{MD}}$ | $g_{\mathrm{max1}}^{\mathrm{IOI}}$ | $\epsilon_{\mathrm{IOI}}(\%)$ | $g_{\mathrm{max1}}^{\mathrm{LCT}}$ | $\epsilon_{\mathrm{LCT}}(\%)$ |
|---|---|---|---|---|---|---|
| 10.0 | 0.05 | 1.101 | 1.084 | 1.575 | 1.100 | 0.085 |
| 15.0 | 0.07 | 1.175 | 1.154 | 1.805 | 1.176 | 0.127 |
| 20.0 | 0.09 | 1.243 | 1.217 | 2.074 | 1.246 | 0.268 |
| 25.0 | 0.11 | 1.304 | 1.278 | 2.029 | 1.309 | 0.366 |
| 30.0 | 0.14 | 1.360 | 1.335 | 1.872 | 1.365 | 0.397 |
| 35.0 | 0.16 | 1.413 | 1.388 | 1.754 | 1.418 | 0.327 |
| 40.0 | 0.18 | 1.462 | 1.439 | 1.582 | 1.466 | 0.307 |
| 45.0 | 0.20 | 1.509 | 1.487 | 1.469 | 1.513 | 0.246 |
| 50.0 | 0.23 | 1.553 | 1.532 | 1.323 | 1.557 | 0.243 |
| 55.0 | 0.25 | 1.595 | 1.576 | 1.190 | 1.599 | 0.251 |
| 60.0 | 0.27 | 1.636 | 1.618 | 1.114 | 1.640 | 0.221 |
| 65.0 | 0.30 | 1.675 | 1.658 | 1.019 | 1.679 | 0.227 |
| 70.0 | 0.32 | 1.711 | 1.697 | 0.837 | 1.717 | 0.331 |
| 75.0 | 0.34 | 1.749 | 1.734 | 0.849 | 1.753 | 0.247 |
| 80.0 | 0.36 | 1.783 | 1.770 | 0.702 | 1.789 | 0.329 |
| 85.0 | 0.39 | 1.817 | 1.806 | 0.617 | 1.823 | 0.351 |
| 90.0 | 0.41 | 1.850 | 1.840 | 0.533 | 1.857 | 0.375 |
| 95.0 | 0.43 | 1.882 | 1.874 | 0.444 | 1.890 | 0.405 |
| 100.0 | 0.45 | 1.914 | 1.906 | 0.400 | 1.921 | 0.391 |
| 105.0 | 0.48 | 1.944 | 1.938 | 0.293 | 1.953 | 0.441 |
| 110.0 | 0.50 | 1.974 | 1.970 | 0.223 | 1.983 | 0.455 |
| 115.0 | 0.52 | 2.003 | 2.000 | 0.138 | 2.013 | 0.484 |
| 120.0 | 0.54 | 2.031 | 2.030 | 0.035 | 2.042 | 0.532 |
| 125.0 | 0.57 | 2.058 | 2.060 | 0.087 | 2.070 | 0.599 |
| 130.0 | 0.59 | 2.088 | 2.089 | 0.037 | 2.098 | 0.492 |
| 135.0 | 0.61 | 2.114 | 2.117 | 0.154 | 2.126 | 0.553 |
| 140.0 | 0.64 | 2.141 | 2.145 | 0.200 | 2.153 | 0.541 |
| 145.0 | 0.66 | 2.166 | 2.173 | 0.316 | 2.179 | 0.599 |
| 150.0 | 0.68 | 2.191 | 2.200 | 0.410 | 2.205 | 0.634 |
| 155.0 | 0.70 | 2.217 | 2.227 | 0.439 | 2.230 | 0.600 |
| 160.0 | 0.73 | 2.242 | 2.253 | 0.495 | 2.255 | 0.592 |
| 165.0 | 0.75 | 2.266 | 2.279 | 0.577 | 2.280 | 0.607 |
| 170.0 | 0.77 | 2.289 | 2.305 | 0.687 | 2.304 | 0.646 |
| 175.0 | 0.79 | 2.314 | 2.330 | 0.692 | 2.327 | 0.578 |
| 180.0 | 0.82 | 2.337 | 2.355 | 0.769 | 2.350 | 0.577 |
| 185.0 | 0.84 | 2.359 | 2.380 | 0.875 | 2.373 | 0.600 |
| 190.0 | 0.86 | 2.383 | 2.404 | 0.881 | 2.395 | 0.520 |
| 195.0 | 0.89 | 2.404 | 2.428 | 1.000 | 2.417 | 0.548 |
| 200.0 | 0.91 | 2.427 | 2.452 | 1.022 | 2.439 | 0.474 |
| $\boldsymbol{\epsilon_{\mathrm{AVE}}}(\%)$ | | | | **0.834** | | **0.425** |
| $\boldsymbol{\epsilon_{\mathrm{MAX}}}(\%)$ | | | | **2.074** | | **0.646** |

**Table 2c.** Key properties of the radial distribution function resulting from molecular dynamics (MD) simulations and from two versions of the isomorph-based empirically modified hypernetted chain (IEMHNC) approach: the version constructed with the OCP bridge function given by Iyetomi, Ogata and Ichimaru (IOI) in *H. Iyetomi, S. Ogata and S. Ichimaru, Phys. Rev. A* **46**, *1051 (1992)* and the version constructed with the new OCP bridge function parameterization proposed by the authors (LCT). The absolute relative deviation $\epsilon_{\mathrm{r}}$ between the theoretical and the simulation results is also reported together with its average and maximum values (the average deviation is denoted as $\epsilon_{\mathrm{AVE}}$ and the maximum deviation is denoted as $\epsilon_{\mathrm{MAX}}$). **Results for the magnitude of the first maximum in the case of $\boldsymbol{\kappa = 2.0}$.** The MD results are adopted from *T. Ott and M. Bonitz, Contrib. Plasma Phys.* **55**, *243 (2015)*.

| $\Gamma$ | $\Gamma/\Gamma_m$ | $g_{\mathrm{max1}}^{\mathrm{MD}}$ | $g_{\mathrm{max1}}^{\mathrm{IOI}}$ | $\epsilon_{\mathrm{IOI}}(\%)$ | $g_{\mathrm{max1}}^{\mathrm{LCT}}$ | $\epsilon_{\mathrm{LCT}}(\%)$ |
|---|---|---|---|---|---|---|
| 30.0 | 0.07 | 1.202 | 1.180 | 1.808 | 1.202 | 0.019 |
| 40.0 | 0.09 | 1.270 | 1.244 | 2.015 | 1.274 | 0.302 |
| 50.0 | 0.11 | 1.331 | 1.306 | 1.911 | 1.337 | 0.428 |
| 60.0 | 0.13 | 1.388 | 1.363 | 1.772 | 1.393 | 0.395 |
| 70.0 | 0.15 | 1.440 | 1.418 | 1.537 | 1.446 | 0.411 |
| 80.0 | 0.17 | 1.490 | 1.469 | 1.393 | 1.495 | 0.341 |
| 90.0 | 0.20 | 1.536 | 1.518 | 1.179 | 1.542 | 0.369 |
| 100.0 | 0.22 | 1.582 | 1.564 | 1.130 | 1.586 | 0.263 |
| 110.0 | 0.24 | 1.624 | 1.608 | 0.969 | 1.629 | 0.299 |
| 120.0 | 0.26 | 1.664 | 1.651 | 0.808 | 1.670 | 0.358 |
| 130.0 | 0.28 | 1.702 | 1.691 | 0.634 | 1.710 | 0.447 |
| 140.0 | 0.31 | 1.741 | 1.730 | 0.609 | 1.748 | 0.399 |
| 150.0 | 0.33 | 1.777 | 1.768 | 0.490 | 1.785 | 0.454 |
| 160.0 | 0.35 | 1.812 | 1.805 | 0.385 | 1.821 | 0.500 |
| 170.0 | 0.37 | 1.847 | 1.841 | 0.342 | 1.856 | 0.487 |
| 180.0 | 0.39 | 1.879 | 1.875 | 0.192 | 1.890 | 0.583 |
| 190.0 | 0.41 | 1.912 | 1.909 | 0.147 | 1.923 | 0.575 |
| 200.0 | 0.44 | 1.944 | 1.942 | 0.093 | 1.955 | 0.576 |
| 210.0 | 0.46 | 1.974 | 1.974 | 0.022 | 1.987 | 0.640 |
| 220.0 | 0.48 | 2.004 | 2.006 | 0.099 | 2.017 | 0.666 |
| 230.0 | 0.50 | 2.034 | 2.037 | 0.142 | 2.047 | 0.657 |
| 240.0 | 0.52 | 2.062 | 2.067 | 0.251 | 2.077 | 0.715 |
| 250.0 | 0.55 | 2.091 | 2.097 | 0.282 | 2.106 | 0.695 |
| 260.0 | 0.57 | 2.119 | 2.126 | 0.334 | 2.134 | 0.696 |
| 270.0 | 0.59 | 2.145 | 2.155 | 0.454 | 2.161 | 0.765 |
| 280.0 | 0.61 | 2.173 | 2.183 | 0.457 | 2.189 | 0.717 |
| 290.0 | 0.63 | 2.198 | 2.211 | 0.577 | 2.215 | 0.784 |
| 300.0 | 0.65 | 2.225 | 2.238 | 0.584 | 2.241 | 0.737 |
| 310.0 | 0.68 | 2.250 | 2.265 | 0.661 | 2.267 | 0.761 |
| 320.0 | 0.70 | 2.274 | 2.291 | 0.764 | 2.292 | 0.807 |
| 330.0 | 0.72 | 2.299 | 2.318 | 0.805 | 2.317 | 0.790 |
| 340.0 | 0.74 | 2.324 | 2.343 | 0.829 | 2.342 | 0.754 |
| 350.0 | 0.76 | 2.347 | 2.369 | 0.925 | 2.365 | 0.786 |
| 360.0 | 0.79 | 2.371 | 2.394 | 0.961 | 2.389 | 0.756 |
| 370.0 | 0.81 | 2.394 | 2.419 | 1.026 | 2.412 | 0.751 |
| 380.0 | 0.83 | 2.417 | 2.443 | 1.076 | 2.435 | 0.729 |
| 390.0 | 0.85 | 2.438 | 2.467 | 1.196 | 2.457 | 0.772 |
| 400.0 | 0.87 | 2.462 | 2.491 | 1.179 | 2.479 | 0.675 |
| $\boldsymbol{\epsilon_{\mathrm{AVE}}}(\%)$ | | | | **0.790** | | **0.575** |
| $\boldsymbol{\epsilon_{\mathrm{MAX}}}(\%)$ | | | | **2.015** | | **0.807** |

**Table 3a.** Key properties of the radial distribution function resulting from molecular dynamics (MD) simulations and from two versions of the isomorph-based empirically modified hypernetted chain (IEMHNC) approach: the version constructed with the OCP bridge function given by Iyetomi, Ogata and Ichimaru (IOI) in *H. Iyetomi, S. Ogata and S. Ichimaru, Phys. Rev. A* **46**, *1051 (1992)* and the version constructed with the new OCP bridge function parameterization proposed by the authors (LCT). The absolute relative deviation $\epsilon_{\mathrm{r}}$ between the theoretical and the simulation results is also reported together with its average and maximum values (the average deviation is denoted as $\epsilon_{\mathrm{AVE}}$ and the maximum deviation is denoted as $\epsilon_{\mathrm{MAX}}$). **Results for the position of the first maximum in the case of $\boldsymbol{\kappa} = \mathbf{0.0}$.** The MD results are adopted from *T. Ott and M. Bonitz, Contrib. Plasma Phys.* **55**, *243 (2015)*. Here $x = r/d$, where $d$ is the Wigner-Seitz radius.

| $\Gamma$ | $\Gamma/\Gamma_m$ | $x_{\mathrm{max1}}^{\mathrm{MD}}$ | $x_{\mathrm{max1}}^{\mathrm{IOI}}$ | $\epsilon_{\mathrm{IOI}}(\%)$ | $x_{\mathrm{max1}}^{\mathrm{LCT}}$ | $\epsilon_{\mathrm{LCT}}(\%)$ |
|---|---|---|---|---|---|---|
| 15.0 | 0.09 | 1.666 | 1.678 | 0.720 | 1.660 | 0.360 |
| 20.0 | 0.12 | 1.665 | 1.672 | 0.420 | 1.663 | 0.120 |
| 25.0 | 0.15 | 1.668 | 1.670 | 0.120 | 1.669 | 0.060 |
| 30.0 | 0.17 | 1.671 | 1.670 | 0.060 | 1.674 | 0.180 |
| 35.0 | 0.20 | 1.674 | 1.671 | 0.179 | 1.678 | 0.239 |
| 40.0 | 0.23 | 1.678 | 1.673 | 0.298 | 1.680 | 0.119 |
| 45.0 | 0.26 | 1.681 | 1.676 | 0.297 | 1.683 | 0.119 |
| 50.0 | 0.29 | 1.685 | 1.678 | 0.415 | 1.685 | 0.000 |
| 55.0 | 0.32 | 1.688 | 1.681 | 0.415 | 1.688 | 0.000 |
| 60.0 | 0.35 | 1.690 | 1.683 | 0.414 | 1.690 | 0.000 |
| 65.0 | 0.38 | 1.693 | 1.686 | 0.413 | 1.692 | 0.059 |
| 70.0 | 0.41 | 1.696 | 1.688 | 0.472 | 1.694 | 0.118 |
| 75.0 | 0.44 | 1.698 | 1.690 | 0.471 | 1.697 | 0.059 |
| 80.0 | 0.47 | 1.701 | 1.693 | 0.470 | 1.699 | 0.118 |
| 85.0 | 0.49 | 1.703 | 1.695 | 0.470 | 1.701 | 0.117 |
| 90.0 | 0.52 | 1.705 | 1.697 | 0.469 | 1.703 | 0.117 |
| 95.0 | 0.55 | 1.707 | 1.699 | 0.469 | 1.705 | 0.117 |
| 100.0 | 0.58 | 1.709 | 1.701 | 0.468 | 1.707 | 0.117 |
| 105.0 | 0.61 | 1.710 | 1.703 | 0.409 | 1.709 | 0.058 |
| 110.0 | 0.64 | 1.712 | 1.705 | 0.409 | 1.711 | 0.058 |
| 115.0 | 0.67 | 1.714 | 1.707 | 0.408 | 1.713 | 0.058 |
| 120.0 | 0.70 | 1.715 | 1.708 | 0.408 | 1.715 | 0.000 |
| 125.0 | 0.73 | 1.717 | 1.710 | 0.408 | 1.716 | 0.058 |
| 130.0 | 0.76 | 1.719 | 1.712 | 0.407 | 1.718 | 0.058 |
| 135.0 | 0.79 | 1.720 | 1.713 | 0.407 | 1.719 | 0.058 |
| 140.0 | 0.81 | 1.721 | 1.715 | 0.349 | 1.721 | 0.000 |
| 145.0 | 0.84 | 1.723 | 1.716 | 0.406 | 1.722 | 0.058 |
| 150.0 | 0.87 | 1.724 | 1.718 | 0.348 | 1.724 | 0.000 |
| 155.0 | 0.90 | 1.725 | 1.719 | 0.348 | 1.725 | 0.000 |
| 160.0 | 0.93 | 1.727 | 1.721 | 0.347 | 1.726 | 0.058 |
| 165.0 | 0.96 | 1.728 | 1.722 | 0.347 | 1.727 | 0.058 |
| $\boldsymbol{\epsilon}_{\mathbf{AVE}}(\%)$ | | | | **0.389** | | **0.082** |
| $\boldsymbol{\epsilon}_{\mathbf{MAX}}(\%)$ | | | | **0.720** | | **0.360** |

**Table 3b.** Key properties of the radial distribution function resulting from molecular dynamics (MD) simulations and from two versions of the isomorph-based empirically modified hypernetted chain (IEMHNC) approach: the version constructed with the OCP bridge function given by Iyetomi, Ogata and Ichimaru (IOI) in *H. Iyetomi, S. Ogata and S. Ichimaru, Phys. Rev. A* **46**, *1051 (1992)* and the version constructed with the new OCP bridge function parameterization proposed by the authors (LCT). The absolute relative deviation $\epsilon_{\mathrm{r}}$ between the theoretical and the simulation results is also reported together with its average and maximum values (the average deviation is denoted as $\epsilon_{\mathrm{AVE}}$ and the maximum deviation is denoted as $\epsilon_{\mathrm{MAX}}$). **Results for the position of the first maximum in the case of $\boldsymbol{\kappa = 1.0}$.** The MD results are adopted from *T. Ott and M. Bonitz, Contrib. Plasma Phys.* **55**, *243 (2015).* Here $x = r/d$, where $d$ is the Wigner-Seitz radius.

| $\Gamma$ | $\Gamma/\Gamma_m$ | $x_{\mathrm{max1}}^{\mathrm{MD}}$ | $x_{\mathrm{max1}}^{\mathrm{IOI}}$ | $\epsilon_{\mathrm{IOI}}(\%)$ | $x_{\mathrm{max1}}^{\mathrm{LCT}}$ | $\epsilon_{\mathrm{LCT}}(\%)$ |
|---|---|---|---|---|---|---|
| 10.0 | 0.05 | 1.660 | 1.664 | 0.241 | 1.679 | 1.145 |
| 15.0 | 0.07 | 1.648 | 1.659 | 0.667 | 1.645 | 0.182 |
| 20.0 | 0.09 | 1.648 | 1.657 | 0.546 | 1.643 | 0.303 |
| 25.0 | 0.11 | 1.650 | 1.656 | 0.364 | 1.649 | 0.061 |
| 30.0 | 0.14 | 1.655 | 1.656 | 0.060 | 1.655 | 0.000 |
| 35.0 | 0.16 | 1.659 | 1.658 | 0.060 | 1.661 | 0.121 |
| 40.0 | 0.18 | 1.662 | 1.660 | 0.120 | 1.665 | 0.181 |
| 45.0 | 0.20 | 1.666 | 1.662 | 0.240 | 1.669 | 0.180 |
| 50.0 | 0.23 | 1.669 | 1.665 | 0.240 | 1.672 | 0.180 |
| 55.0 | 0.25 | 1.673 | 1.667 | 0.359 | 1.675 | 0.120 |
| 60.0 | 0.27 | 1.676 | 1.669 | 0.418 | 1.677 | 0.060 |
| 65.0 | 0.30 | 1.679 | 1.672 | 0.417 | 1.679 | 0.000 |
| 70.0 | 0.32 | 1.681 | 1.674 | 0.416 | 1.681 | 0.000 |
| 75.0 | 0.34 | 1.684 | 1.677 | 0.416 | 1.683 | 0.059 |
| 80.0 | 0.36 | 1.687 | 1.679 | 0.474 | 1.685 | 0.119 |
| 85.0 | 0.39 | 1.689 | 1.681 | 0.474 | 1.687 | 0.118 |
| 90.0 | 0.41 | 1.691 | 1.683 | 0.473 | 1.689 | 0.118 |
| 95.0 | 0.43 | 1.693 | 1.685 | 0.473 | 1.691 | 0.118 |
| 100.0 | 0.45 | 1.695 | 1.687 | 0.472 | 1.693 | 0.118 |
| 105.0 | 0.48 | 1.697 | 1.689 | 0.471 | 1.695 | 0.118 |
| 110.0 | 0.50 | 1.699 | 1.691 | 0.471 | 1.697 | 0.118 |
| 115.0 | 0.52 | 1.701 | 1.693 | 0.470 | 1.699 | 0.118 |
| 120.0 | 0.54 | 1.702 | 1.695 | 0.411 | 1.701 | 0.059 |
| 125.0 | 0.57 | 1.704 | 1.696 | 0.469 | 1.702 | 0.117 |
| 130.0 | 0.59 | 1.706 | 1.698 | 0.469 | 1.704 | 0.117 |
| 135.0 | 0.61 | 1.707 | 1.700 | 0.410 | 1.706 | 0.059 |
| 140.0 | 0.64 | 1.709 | 1.701 | 0.468 | 1.707 | 0.117 |
| 145.0 | 0.66 | 1.710 | 1.703 | 0.409 | 1.709 | 0.058 |
| 150.0 | 0.68 | 1.712 | 1.704 | 0.467 | 1.710 | 0.117 |
| 155.0 | 0.70 | 1.713 | 1.706 | 0.409 | 1.712 | 0.058 |
| 160.0 | 0.73 | 1.715 | 1.707 | 0.466 | 1.713 | 0.117 |
| 165.0 | 0.75 | 1.715 | 1.709 | 0.350 | 1.714 | 0.058 |
| 170.0 | 0.77 | 1.717 | 1.710 | 0.408 | 1.716 | 0.058 |
| 175.0 | 0.79 | 1.718 | 1.711 | 0.407 | 1.717 | 0.058 |
| 180.0 | 0.82 | 1.719 | 1.713 | 0.349 | 1.718 | 0.058 |
| 185.0 | 0.84 | 1.720 | 1.714 | 0.349 | 1.719 | 0.058 |
| 190.0 | 0.86 | 1.721 | 1.715 | 0.349 | 1.720 | 0.058 |
| 195.0 | 0.89 | 1.722 | 1.716 | 0.348 | 1.722 | 0.000 |
| 200.0 | 0.91 | 1.723 | 1.717 | 0.348 | 1.723 | 0.000 |
| $\boldsymbol{\epsilon_{\mathrm{AVE}}}(\%)$ | | | | **0.391** | | **0.121** |
| $\boldsymbol{\epsilon_{\mathrm{MAX}}}(\%)$ | | | | **0.667** | | **1.145** |

**Table 3c.** Key properties of the radial distribution function resulting from molecular dynamics (MD) simulations and from two versions of the isomorph-based empirically modified hypernetted chain (IEMHNC) approach: the version constructed with the OCP bridge function given by Iyetomi, Ogata and Ichimaru (IOI) in *H. Iyetomi, S. Ogata and S. Ichimaru, Phys. Rev. A* **46**, *1051 (1992)* and the version constructed with the new OCP bridge function parameterization proposed by the authors (LCT). The absolute relative deviation $\epsilon_{\mathrm{r}}$ between the theoretical and the simulation results is also reported together with its average and maximum values (the average deviation is denoted as $\epsilon_{\mathrm{AVE}}$ and the maximum deviation is denoted as $\epsilon_{\mathrm{MAX}}$). **Results for the position of the first maximum in the case of $\boldsymbol{\kappa = 2.0}$.** The MD results are adopted from *T. Ott and M. Bonitz, Contrib. Plasma Phys.* **55**, *243 (2015)*. Here $x = r/d$, where $d$ is the Wigner-Seitz radius.

| $\Gamma$ | $\Gamma/\Gamma_m$ | $x_{\mathrm{max1}}^{\mathrm{MD}}$ | $x_{\mathrm{max1}}^{\mathrm{IOI}}$ | $\epsilon_{\mathrm{IOI}}(\%)$ | $x_{\mathrm{max1}}^{\mathrm{LCT}}$ | $\epsilon_{\mathrm{LCT}}(\%)$ |
|---|---|---|---|---|---|---|
| 30.0 | 0.07 | 1.598 | 1.599 | 0.063 | 1.597 | 0.063 |
| 40.0 | 0.09 | 1.609 | 1.611 | 0.124 | 1.605 | 0.249 |
| 50.0 | 0.11 | 1.619 | 1.619 | 0.000 | 1.616 | 0.185 |
| 60.0 | 0.13 | 1.627 | 1.625 | 0.123 | 1.627 | 0.000 |
| 70.0 | 0.15 | 1.633 | 1.631 | 0.122 | 1.635 | 0.122 |
| 80.0 | 0.17 | 1.640 | 1.636 | 0.244 | 1.642 | 0.122 |
| 90.0 | 0.20 | 1.646 | 1.640 | 0.365 | 1.648 | 0.122 |
| 100.0 | 0.22 | 1.651 | 1.645 | 0.363 | 1.652 | 0.061 |
| 110.0 | 0.24 | 1.656 | 1.649 | 0.423 | 1.656 | 0.000 |
| 120.0 | 0.26 | 1.660 | 1.653 | 0.422 | 1.660 | 0.000 |
| 130.0 | 0.28 | 1.664 | 1.656 | 0.481 | 1.663 | 0.060 |
| 140.0 | 0.31 | 1.668 | 1.659 | 0.540 | 1.666 | 0.120 |
| 150.0 | 0.33 | 1.671 | 1.662 | 0.539 | 1.669 | 0.120 |
| 160.0 | 0.35 | 1.674 | 1.665 | 0.538 | 1.672 | 0.119 |
| 170.0 | 0.37 | 1.677 | 1.668 | 0.537 | 1.674 | 0.179 |
| 180.0 | 0.39 | 1.680 | 1.671 | 0.536 | 1.677 | 0.179 |
| 190.0 | 0.41 | 1.683 | 1.674 | 0.535 | 1.679 | 0.238 |
| 200.0 | 0.44 | 1.685 | 1.676 | 0.534 | 1.681 | 0.237 |
| 210.0 | 0.46 | 1.687 | 1.678 | 0.533 | 1.684 | 0.178 |
| 220.0 | 0.48 | 1.690 | 1.681 | 0.533 | 1.686 | 0.237 |
| 230.0 | 0.50 | 1.691 | 1.683 | 0.473 | 1.688 | 0.177 |
| 240.0 | 0.52 | 1.693 | 1.685 | 0.473 | 1.690 | 0.177 |
| 250.0 | 0.55 | 1.696 | 1.687 | 0.531 | 1.692 | 0.236 |
| 260.0 | 0.57 | 1.698 | 1.689 | 0.530 | 1.694 | 0.236 |
| 270.0 | 0.59 | 1.699 | 1.691 | 0.471 | 1.696 | 0.177 |
| 280.0 | 0.61 | 1.701 | 1.693 | 0.470 | 1.698 | 0.176 |
| 290.0 | 0.63 | 1.703 | 1.694 | 0.528 | 1.700 | 0.176 |
| 300.0 | 0.65 | 1.704 | 1.696 | 0.469 | 1.701 | 0.176 |
| 310.0 | 0.68 | 1.706 | 1.698 | 0.469 | 1.703 | 0.176 |
| 320.0 | 0.70 | 1.708 | 1.699 | 0.527 | 1.704 | 0.234 |
| 330.0 | 0.72 | 1.709 | 1.701 | 0.468 | 1.706 | 0.176 |
| 340.0 | 0.74 | 1.711 | 1.702 | 0.526 | 1.707 | 0.234 |
| 350.0 | 0.76 | 1.712 | 1.704 | 0.467 | 1.709 | 0.175 |
| 360.0 | 0.79 | 1.713 | 1.705 | 0.467 | 1.710 | 0.175 |
| 370.0 | 0.81 | 1.715 | 1.707 | 0.466 | 1.712 | 0.175 |
| 380.0 | 0.83 | 1.716 | 1.708 | 0.466 | 1.713 | 0.175 |
| 390.0 | 0.85 | 1.717 | 1.709 | 0.466 | 1.714 | 0.175 |
| 400.0 | 0.87 | 1.718 | 1.711 | 0.407 | 1.715 | 0.175 |
| $\boldsymbol{\epsilon_{\mathrm{AVE}}}(\%)$ | | | | **0.427** | | **0.158** |
| $\boldsymbol{\epsilon_{\mathrm{MAX}}}(\%)$ | | | | **0.540** | | **0.249** |

**Table 4a.** Key properties of the radial distribution function resulting from molecular dynamics (MD) simulations and from two versions of the isomorph-based empirically modified hypernetted chain (IEMHNC) approach: the version constructed with the OCP bridge function given by Iyetomi, Ogata and Ichimaru (IOI) in *H. Iyetomi, S. Ogata and S. Ichimaru, Phys. Rev. A* **46**, *1051 (1992)* and the version constructed with the new OCP bridge function parameterization proposed by the authors (LCT). The absolute relative deviation $\epsilon_{\mathrm{r}}$ between the theoretical and the simulation results is also reported together with its average and maximum values (the average deviation is denoted as $\epsilon_{\mathrm{AVE}}$ and the maximum deviation is denoted as $\epsilon_{\mathrm{MAX}}$). **Results for the magnitude of the first non-zero minimum in the case of $\boldsymbol{\kappa = 0.0}$**. The MD results are adopted from *T. Ott and M. Bonitz, Contrib. Plasma Phys.* **55**, *243 (2015)*.

| $\Gamma$ | $\Gamma/\Gamma_m$ | $g_{\mathrm{min1}}^{\mathrm{MD}}$ | $g_{\mathrm{min1}}^{\mathrm{IOI}}$ | $\epsilon_{\mathrm{IOI}}(\%)$ | $g_{\mathrm{min1}}^{\mathrm{LCT}}$ | $\epsilon_{\mathrm{LCT}}(\%)$ |
|---|---|---|---|---|---|---|
| 15.0 | 0.09 | 0.952 | 0.959 | 0.743 | 0.953 | 0.140 |
| 20.0 | 0.12 | 0.925 | 0.935 | 1.092 | 0.927 | 0.182 |
| 25.0 | 0.15 | 0.899 | 0.912 | 1.397 | 0.901 | 0.236 |
| 30.0 | 0.17 | 0.876 | 0.889 | 1.521 | 0.877 | 0.140 |
| 35.0 | 0.20 | 0.853 | 0.869 | 1.837 | 0.855 | 0.243 |
| 40.0 | 0.23 | 0.833 | 0.850 | 1.987 | 0.835 | 0.190 |
| 45.0 | 0.26 | 0.814 | 0.832 | 2.192 | 0.816 | 0.198 |
| 50.0 | 0.29 | 0.796 | 0.815 | 2.434 | 0.798 | 0.250 |
| 55.0 | 0.32 | 0.780 | 0.800 | 2.565 | 0.782 | 0.202 |
| 60.0 | 0.35 | 0.765 | 0.786 | 2.691 | 0.766 | 0.159 |
| 65.0 | 0.38 | 0.750 | 0.772 | 2.935 | 0.752 | 0.239 |
| 70.0 | 0.41 | 0.737 | 0.759 | 3.008 | 0.738 | 0.161 |
| 75.0 | 0.44 | 0.724 | 0.747 | 3.173 | 0.725 | 0.182 |
| 80.0 | 0.47 | 0.711 | 0.735 | 3.426 | 0.713 | 0.294 |
| 85.0 | 0.49 | 0.700 | 0.724 | 3.466 | 0.701 | 0.206 |
| 90.0 | 0.52 | 0.689 | 0.714 | 3.576 | 0.690 | 0.190 |
| 95.0 | 0.55 | 0.678 | 0.703 | 3.751 | 0.680 | 0.243 |
| 100.0 | 0.58 | 0.668 | 0.694 | 3.835 | 0.669 | 0.211 |
| 105.0 | 0.61 | 0.658 | 0.684 | 3.975 | 0.660 | 0.236 |
| 110.0 | 0.64 | 0.648 | 0.675 | 4.169 | 0.650 | 0.316 |
| 115.0 | 0.67 | 0.639 | 0.666 | 4.253 | 0.641 | 0.290 |
| 120.0 | 0.70 | 0.630 | 0.658 | 4.384 | 0.632 | 0.310 |
| 125.0 | 0.73 | 0.621 | 0.649 | 4.561 | 0.623 | 0.373 |
| 130.0 | 0.76 | 0.613 | 0.641 | 4.612 | 0.615 | 0.314 |
| 135.0 | 0.79 | 0.605 | 0.633 | 4.701 | 0.607 | 0.290 |
| 140.0 | 0.81 | 0.596 | 0.626 | 5.005 | 0.599 | 0.467 |
| 145.0 | 0.84 | 0.588 | 0.618 | 5.173 | 0.591 | 0.510 |
| 150.0 | 0.87 | 0.581 | 0.611 | 5.197 | 0.583 | 0.410 |
| 155.0 | 0.90 | 0.574 | 0.604 | 5.253 | 0.576 | 0.335 |
| 160.0 | 0.93 | 0.567 | 0.597 | 5.340 | 0.569 | 0.283 |
| 165.0 | 0.96 | 0.560 | 0.591 | 5.459 | 0.561 | 0.254 |
| $\boldsymbol{\epsilon_{\mathrm{AVE}}}(\%)$ | | | | **3.474** | | **0.260** |
| $\boldsymbol{\epsilon_{\mathrm{MAX}}}(\%)$ | | | | **5.459** | | **0.510** |

**Table 4b.** Key properties of the radial distribution function resulting from molecular dynamics (MD) simulations and from two versions of the isomorph-based empirically modified hypernetted chain (IEMHNC) approach: the version constructed with the OCP bridge function given by Iyetomi, Ogata and Ichimaru (IOI) in *H. Iyetomi, S. Ogata and S. Ichimaru, Phys. Rev. A* **46**, *1051 (1992)* and the version constructed with the new OCP bridge function parameterization proposed by the authors (LCT). The absolute relative deviation $\epsilon_{\mathrm{r}}$ between the theoretical and the simulation results is also reported together with its average and maximum values (the average deviation is denoted as $\epsilon_{\mathrm{AVE}}$ and the maximum deviation is denoted as $\epsilon_{\mathrm{MAX}}$). **Results for the magnitude of the first non-zero minimum in the case of $\boldsymbol{\kappa = 1.0}$**. The MD results are adopted from *T. Ott and M. Bonitz, Contrib. Plasma Phys.* **55**, *243 (2015).*

| $\Gamma$ | $\Gamma/\Gamma_m$ | $g_{\mathrm{min1}}^{\mathrm{MD}}$ | $g_{\mathrm{min1}}^{\mathrm{IOI}}$ | $\epsilon_{\mathrm{IOI}}(\%)$ | $g_{\mathrm{min1}}^{\mathrm{LCT}}$ | $\epsilon_{\mathrm{LCT}}(\%)$ |
|---|---|---|---|---|---|---|
| 10.0 | 0.05 | 0.987 | 0.991 | 0.429 | 0.987 | 0.010 |
| 15.0 | 0.07 | 0.969 | 0.973 | 0.447 | 0.968 | 0.052 |
| 20.0 | 0.09 | 0.948 | 0.955 | 0.707 | 0.948 | 0.030 |
| 25.0 | 0.11 | 0.927 | 0.936 | 0.937 | 0.927 | 0.024 |
| 30.0 | 0.14 | 0.907 | 0.917 | 1.096 | 0.907 | 0.049 |
| 35.0 | 0.16 | 0.887 | 0.899 | 1.349 | 0.887 | 0.040 |
| 40.0 | 0.18 | 0.869 | 0.882 | 1.493 | 0.869 | 0.027 |
| 45.0 | 0.20 | 0.853 | 0.866 | 1.523 | 0.852 | 0.096 |
| 50.0 | 0.23 | 0.836 | 0.851 | 1.792 | 0.836 | 0.018 |
| 55.0 | 0.25 | 0.822 | 0.837 | 1.809 | 0.821 | 0.116 |
| 60.0 | 0.27 | 0.807 | 0.824 | 2.052 | 0.807 | 0.022 |
| 65.0 | 0.30 | 0.794 | 0.811 | 2.139 | 0.793 | 0.078 |
| 70.0 | 0.32 | 0.781 | 0.799 | 2.313 | 0.781 | 0.045 |
| 75.0 | 0.34 | 0.769 | 0.788 | 2.435 | 0.769 | 0.056 |
| 80.0 | 0.36 | 0.758 | 0.777 | 2.495 | 0.757 | 0.122 |
| 85.0 | 0.39 | 0.747 | 0.767 | 2.621 | 0.746 | 0.119 |
| 90.0 | 0.41 | 0.736 | 0.757 | 2.809 | 0.736 | 0.051 |
| 95.0 | 0.43 | 0.726 | 0.747 | 2.915 | 0.726 | 0.058 |
| 100.0 | 0.45 | 0.716 | 0.738 | 3.073 | 0.716 | 0.010 |
| 105.0 | 0.48 | 0.707 | 0.729 | 3.137 | 0.707 | 0.051 |
| 110.0 | 0.50 | 0.698 | 0.721 | 3.245 | 0.698 | 0.044 |
| 115.0 | 0.52 | 0.689 | 0.712 | 3.395 | 0.689 | 0.007 |
| 120.0 | 0.54 | 0.681 | 0.704 | 3.437 | 0.681 | 0.045 |
| 125.0 | 0.57 | 0.672 | 0.697 | 3.668 | 0.673 | 0.089 |
| 130.0 | 0.59 | 0.664 | 0.689 | 3.783 | 0.665 | 0.112 |
| 135.0 | 0.61 | 0.657 | 0.682 | 3.774 | 0.657 | 0.019 |
| 140.0 | 0.64 | 0.649 | 0.675 | 3.955 | 0.650 | 0.109 |
| 145.0 | 0.66 | 0.642 | 0.668 | 4.007 | 0.642 | 0.076 |
| 150.0 | 0.68 | 0.634 | 0.661 | 4.252 | 0.635 | 0.228 |
| 155.0 | 0.70 | 0.627 | 0.654 | 4.362 | 0.629 | 0.252 |
| 160.0 | 0.73 | 0.620 | 0.648 | 4.500 | 0.622 | 0.300 |
| 165.0 | 0.75 | 0.614 | 0.642 | 4.495 | 0.615 | 0.212 |
| 170.0 | 0.77 | 0.608 | 0.635 | 4.513 | 0.609 | 0.143 |
| 175.0 | 0.79 | 0.601 | 0.629 | 4.727 | 0.603 | 0.261 |
| 180.0 | 0.82 | 0.595 | 0.624 | 4.791 | 0.596 | 0.234 |
| 185.0 | 0.84 | 0.588 | 0.618 | 5.056 | 0.590 | 0.395 |
| 190.0 | 0.86 | 0.582 | 0.612 | 5.166 | 0.584 | 0.405 |
| 195.0 | 0.89 | 0.577 | 0.607 | 5.115 | 0.578 | 0.259 |
| 200.0 | 0.91 | 0.571 | 0.601 | 5.266 | 0.573 | 0.301 |
| $\boldsymbol{\epsilon_{\mathrm{AVE}}}(\%)$ | | | | **3.053** | | **0.117** |
| $\boldsymbol{\epsilon_{\mathrm{MAX}}}(\%)$ | | | | **5.266** | | **0.405** |

**Table 4c.** Key properties of the radial distribution function resulting from molecular dynamics (MD) simulations and from two versions of the isomorph-based empirically modified hypernetted chain (IEMHNC) approach: the version constructed with the OCP bridge function given by Iyetomi, Ogata and Ichimaru (IOI) in *H. Iyetomi, S. Ogata and S. Ichimaru, Phys. Rev. A* **46**, *1051 (1992)* and the version constructed with the new OCP bridge function parameterization proposed by the authors (LCT). The absolute relative deviation $\epsilon_{\mathrm{r}}$ between the theoretical and the simulation results is also reported together with its average and maximum values (the average deviation is denoted as $\epsilon_{\mathrm{AVE}}$ and the maximum deviation is denoted as $\epsilon_{\mathrm{MAX}}$). **Results for the magnitude of the first non-zero minimum in the case of $\boldsymbol{\kappa = 2.0}$**. The MD results are adopted from *T. Ott and M. Bonitz, Contrib. Plasma Phys.* **55**, *243 (2015)*.

| $\Gamma$ | $\Gamma/\Gamma_m$ | $g_{\mathrm{min1}}^{\mathrm{MD}}$ | $g_{\mathrm{min1}}^{\mathrm{IOI}}$ | $\epsilon_{\mathrm{IOI}}(\%)$ | $g_{\mathrm{min1}}^{\mathrm{LCT}}$ | $\epsilon_{\mathrm{LCT}}(\%)$ |
|---|---|---|---|---|---|---|
| 30.0 | 0.07 | 0.963 | 0.968 | 0.546 | 0.962 | 0.082 |
| 40.0 | 0.09 | 0.941 | 0.949 | 0.853 | 0.941 | 0.031 |
| 50.0 | 0.11 | 0.920 | 0.930 | 1.035 | 0.920 | 0.032 |
| 60.0 | 0.13 | 0.900 | 0.911 | 1.171 | 0.900 | 0.031 |
| 70.0 | 0.15 | 0.881 | 0.893 | 1.311 | 0.881 | 0.014 |
| 80.0 | 0.17 | 0.863 | 0.876 | 1.471 | 0.863 | 0.020 |
| 90.0 | 0.20 | 0.846 | 0.860 | 1.648 | 0.847 | 0.065 |
| 100.0 | 0.22 | 0.831 | 0.845 | 1.710 | 0.831 | 0.008 |
| 110.0 | 0.24 | 0.816 | 0.831 | 1.887 | 0.816 | 0.029 |
| 120.0 | 0.26 | 0.802 | 0.818 | 2.046 | 0.802 | 0.047 |
| 130.0 | 0.28 | 0.789 | 0.806 | 2.173 | 0.789 | 0.035 |
| 140.0 | 0.31 | 0.776 | 0.795 | 2.387 | 0.777 | 0.113 |
| 150.0 | 0.33 | 0.764 | 0.783 | 2.549 | 0.765 | 0.143 |
| 160.0 | 0.35 | 0.753 | 0.773 | 2.647 | 0.754 | 0.115 |
| 170.0 | 0.37 | 0.742 | 0.763 | 2.811 | 0.743 | 0.156 |
| 180.0 | 0.39 | 0.732 | 0.753 | 2.896 | 0.733 | 0.124 |
| 190.0 | 0.41 | 0.721 | 0.744 | 3.179 | 0.723 | 0.288 |
| 200.0 | 0.44 | 0.712 | 0.735 | 3.228 | 0.714 | 0.229 |
| 210.0 | 0.46 | 0.702 | 0.726 | 3.470 | 0.705 | 0.362 |
| 220.0 | 0.48 | 0.693 | 0.718 | 3.611 | 0.696 | 0.401 |
| 230.0 | 0.50 | 0.684 | 0.710 | 3.796 | 0.687 | 0.483 |
| 240.0 | 0.52 | 0.676 | 0.702 | 3.868 | 0.679 | 0.460 |
| 250.0 | 0.55 | 0.667 | 0.695 | 4.132 | 0.671 | 0.626 |
| 260.0 | 0.57 | 0.659 | 0.687 | 4.278 | 0.663 | 0.678 |
| 270.0 | 0.59 | 0.651 | 0.680 | 4.458 | 0.656 | 0.767 |
| 280.0 | 0.61 | 0.644 | 0.673 | 4.510 | 0.649 | 0.733 |
| 290.0 | 0.63 | 0.636 | 0.666 | 4.756 | 0.642 | 0.886 |
| 300.0 | 0.65 | 0.628 | 0.660 | 5.034 | 0.635 | 1.072 |
| 310.0 | 0.68 | 0.622 | 0.653 | 5.007 | 0.628 | 0.964 |
| 320.0 | 0.70 | 0.614 | 0.647 | 5.346 | 0.621 | 1.208 |
| 330.0 | 0.72 | 0.608 | 0.641 | 5.370 | 0.615 | 1.149 |
| 340.0 | 0.74 | 0.602 | 0.635 | 5.417 | 0.609 | 1.110 |
| 350.0 | 0.76 | 0.595 | 0.629 | 5.664 | 0.603 | 1.263 |
| 360.0 | 0.79 | 0.588 | 0.623 | 5.937 | 0.596 | 1.440 |
| 370.0 | 0.81 | 0.583 | 0.617 | 5.874 | 0.591 | 1.291 |
| 380.0 | 0.83 | 0.577 | 0.612 | 6.012 | 0.585 | 1.334 |
| 390.0 | 0.85 | 0.571 | 0.606 | 6.172 | 0.579 | 1.395 |
| 400.0 | 0.87 | 0.565 | 0.601 | 6.353 | 0.573 | 1.474 |
| $\boldsymbol{\epsilon_{\mathrm{AVE}}}(\%)$ | | | | **3.542** | | **0.544** |
| $\boldsymbol{\epsilon_{\mathrm{MAX}}}(\%)$ | | | | **6.353** | | **1.474** |

**Table 5a.** Key properties of the radial distribution function resulting from molecular dynamics (MD) simulations and from two versions of the isomorph-based empirically modified hypernetted chain (IEMHNC) approach: the version constructed with the OCP bridge function given by Iyetomi, Ogata and Ichimaru (IOI) in *H. Iyetomi, S. Ogata and S. Ichimaru, Phys. Rev. A* **46**, *1051 (1992)* and the version constructed with the new OCP bridge function parameterization proposed by the authors (LCT). The absolute relative deviation $\epsilon_{\mathrm{r}}$ between the theoretical and the simulation results is also reported together with its average and maximum values (the average deviation is denoted as $\epsilon_{\mathrm{AVE}}$ and the maximum deviation is denoted as $\epsilon_{\mathrm{MAX}}$). **Results for the position of the first non-zero minimum in the case of $\boldsymbol{\kappa = 0.0}$.** The MD results are adopted from *T. Ott and M. Bonitz, Contrib. Plasma Phys.* **55**, *243 (2015)*. Here $x = r/d$, where $d$ is the Wigner-Seitz radius.

| $\Gamma$ | $\Gamma/\Gamma_m$ | $x_{\mathrm{min1}}^{\mathrm{MD}}$ | $x_{\mathrm{min1}}^{\mathrm{IOI}}$ | $\epsilon_{\mathrm{IOI}}(\%)$ | $x_{\mathrm{min1}}^{\mathrm{LCT}}$ | $\epsilon_{\mathrm{LCT}}(\%)$ |
|---|---|---|---|---|---|---|
| 15.0 | 0.09 | 2.489 | 2.538 | 1.969 | 2.486 | 0.121 |
| 20.0 | 0.12 | 2.472 | 2.510 | 1.537 | 2.474 | 0.081 |
| 25.0 | 0.15 | 2.467 | 2.494 | 1.094 | 2.470 | 0.122 |
| 30.0 | 0.17 | 2.463 | 2.485 | 0.893 | 2.468 | 0.203 |
| 35.0 | 0.20 | 2.461 | 2.480 | 0.772 | 2.466 | 0.203 |
| 40.0 | 0.23 | 2.461 | 2.476 | 0.610 | 2.464 | 0.122 |
| 45.0 | 0.26 | 2.459 | 2.473 | 0.569 | 2.463 | 0.163 |
| 50.0 | 0.29 | 2.459 | 2.471 | 0.488 | 2.461 | 0.081 |
| 55.0 | 0.32 | 2.456 | 2.468 | 0.489 | 2.459 | 0.122 |
| 60.0 | 0.35 | 2.455 | 2.466 | 0.448 | 2.457 | 0.081 |
| 65.0 | 0.38 | 2.454 | 2.464 | 0.407 | 2.455 | 0.041 |
| 70.0 | 0.41 | 2.453 | 2.462 | 0.367 | 2.452 | 0.041 |
| 75.0 | 0.44 | 2.451 | 2.459 | 0.326 | 2.450 | 0.041 |
| 80.0 | 0.47 | 2.449 | 2.457 | 0.327 | 2.448 | 0.041 |
| 85.0 | 0.49 | 2.448 | 2.455 | 0.286 | 2.446 | 0.082 |
| 90.0 | 0.52 | 2.446 | 2.453 | 0.286 | 2.443 | 0.123 |
| 95.0 | 0.55 | 2.443 | 2.450 | 0.287 | 2.441 | 0.082 |
| 100.0 | 0.58 | 2.441 | 2.448 | 0.287 | 2.439 | 0.082 |
| 105.0 | 0.61 | 2.439 | 2.446 | 0.287 | 2.437 | 0.082 |
| 110.0 | 0.64 | 2.439 | 2.444 | 0.205 | 2.435 | 0.164 |
| 115.0 | 0.67 | 2.437 | 2.442 | 0.205 | 2.432 | 0.205 |
| 120.0 | 0.70 | 2.435 | 2.440 | 0.205 | 2.430 | 0.205 |
| 125.0 | 0.73 | 2.434 | 2.438 | 0.164 | 2.428 | 0.247 |
| 130.0 | 0.76 | 2.432 | 2.436 | 0.164 | 2.427 | 0.206 |
| 135.0 | 0.79 | 2.431 | 2.434 | 0.123 | 2.425 | 0.247 |
| 140.0 | 0.81 | 2.428 | 2.432 | 0.165 | 2.423 | 0.206 |
| 145.0 | 0.84 | 2.428 | 2.430 | 0.082 | 2.421 | 0.288 |
| 150.0 | 0.87 | 2.426 | 2.429 | 0.124 | 2.419 | 0.289 |
| 155.0 | 0.90 | 2.425 | 2.427 | 0.082 | 2.418 | 0.289 |
| 160.0 | 0.93 | 2.424 | 2.425 | 0.041 | 2.416 | 0.330 |
| 165.0 | 0.96 | 2.423 | 2.424 | 0.041 | 2.415 | 0.330 |
| $\boldsymbol{\epsilon_{\mathrm{AVE}}}(\%)$ | | | | **0.430** | | **0.159** |
| $\boldsymbol{\epsilon_{\mathrm{MAX}}}(\%)$ | | | | **1.969** | | **0.330** |

**Table 5b.** Key properties of the radial distribution function resulting from molecular dynamics (MD) simulations and from two versions of the isomorph-based empirically modified hypernetted chain (IEMHNC) approach: the version constructed with the OCP bridge function given by Iyetomi, Ogata and Ichimaru (IOI) in *H. Iyetomi, S. Ogata and S. Ichimaru, Phys. Rev. A* **46**, *1051 (1992)* and the version constructed with the new OCP bridge function parameterization proposed by the authors (LCT). The absolute relative deviation $\epsilon_{\mathrm{r}}$ between the theoretical and the simulation results is also reported together with its average and maximum values (the average deviation is denoted as $\epsilon_{\mathrm{AVE}}$ and the maximum deviation is denoted as $\epsilon_{\mathrm{MAX}}$). **Results for the position of the first non-zero minimum in the case of $\boldsymbol{\kappa}$ = 1.0**. The MD results are adopted from *T. Ott and M. Bonitz, Contrib. Plasma Phys.* **55**, *243 (2015)*. Here $x = r/d$, where $d$ is the Wigner-Seitz radius.

| $\Gamma$ | $\Gamma/\Gamma_m$ | $x_{\mathrm{min1}}^{\mathrm{MD}}$ | $x_{\mathrm{min1}}^{\mathrm{IOI}}$ | $\epsilon_{\mathrm{IOI}}(\%)$ | $x_{\mathrm{min1}}^{\mathrm{LCT}}$ | $\epsilon_{\mathrm{LCT}}(\%)$ |
|---|---|---|---|---|---|---|
| 10.0 | 0.05 | 2.520 | 2.576 | 2.222 | 2.536 | 0.635 |
| 15.0 | 0.07 | 2.482 | 2.526 | 1.773 | 2.475 | 0.282 |
| 20.0 | 0.09 | 2.464 | 2.505 | 1.664 | 2.459 | 0.203 |
| 25.0 | 0.11 | 2.457 | 2.489 | 1.302 | 2.455 | 0.081 |
| 30.0 | 0.14 | 2.454 | 2.479 | 1.019 | 2.454 | 0.000 |
| 35.0 | 0.16 | 2.452 | 2.473 | 0.856 | 2.454 | 0.082 |
| 40.0 | 0.18 | 2.452 | 2.469 | 0.693 | 2.455 | 0.122 |
| 45.0 | 0.20 | 2.454 | 2.467 | 0.530 | 2.455 | 0.041 |
| 50.0 | 0.23 | 2.452 | 2.465 | 0.530 | 2.455 | 0.122 |
| 55.0 | 0.25 | 2.452 | 2.464 | 0.489 | 2.454 | 0.082 |
| 60.0 | 0.27 | 2.452 | 2.462 | 0.408 | 2.454 | 0.082 |
| 65.0 | 0.30 | 2.452 | 2.461 | 0.367 | 2.453 | 0.041 |
| 70.0 | 0.32 | 2.451 | 2.460 | 0.367 | 2.452 | 0.041 |
| 75.0 | 0.34 | 2.450 | 2.458 | 0.327 | 2.450 | 0.000 |
| 80.0 | 0.36 | 2.449 | 2.457 | 0.327 | 2.449 | 0.000 |
| 85.0 | 0.39 | 2.448 | 2.456 | 0.327 | 2.448 | 0.000 |
| 90.0 | 0.41 | 2.447 | 2.454 | 0.286 | 2.446 | 0.041 |
| 95.0 | 0.43 | 2.446 | 2.453 | 0.286 | 2.445 | 0.041 |
| 100.0 | 0.45 | 2.445 | 2.451 | 0.245 | 2.443 | 0.082 |
| 105.0 | 0.48 | 2.443 | 2.450 | 0.287 | 2.441 | 0.082 |
| 110.0 | 0.50 | 2.442 | 2.448 | 0.246 | 2.440 | 0.082 |
| 115.0 | 0.52 | 2.442 | 2.446 | 0.164 | 2.438 | 0.164 |
| 120.0 | 0.54 | 2.440 | 2.445 | 0.205 | 2.436 | 0.164 |
| 125.0 | 0.57 | 2.438 | 2.443 | 0.205 | 2.435 | 0.123 |
| 130.0 | 0.59 | 2.437 | 2.442 | 0.205 | 2.433 | 0.164 |
| 135.0 | 0.61 | 2.437 | 2.440 | 0.123 | 2.432 | 0.205 |
| 140.0 | 0.64 | 2.436 | 2.439 | 0.123 | 2.430 | 0.246 |
| 145.0 | 0.66 | 2.434 | 2.437 | 0.123 | 2.429 | 0.205 |
| 150.0 | 0.68 | 2.432 | 2.436 | 0.164 | 2.427 | 0.206 |
| 155.0 | 0.70 | 2.432 | 2.434 | 0.082 | 2.426 | 0.247 |
| 160.0 | 0.73 | 2.430 | 2.433 | 0.123 | 2.424 | 0.247 |
| 165.0 | 0.75 | 2.429 | 2.431 | 0.082 | 2.423 | 0.247 |
| 170.0 | 0.77 | 2.428 | 2.430 | 0.082 | 2.421 | 0.288 |
| 175.0 | 0.79 | 2.427 | 2.428 | 0.041 | 2.420 | 0.288 |
| 180.0 | 0.82 | 2.426 | 2.427 | 0.041 | 2.419 | 0.289 |
| 185.0 | 0.84 | 2.425 | 2.426 | 0.041 | 2.418 | 0.289 |
| 190.0 | 0.86 | 2.424 | 2.425 | 0.041 | 2.416 | 0.330 |
| 195.0 | 0.89 | 2.423 | 2.423 | 0.000 | 2.415 | 0.330 |
| 200.0 | 0.91 | 2.422 | 2.422 | 0.000 | 2.414 | 0.330 |
| $\boldsymbol{\epsilon}_{\mathbf{AVE}}(\%)$ | | | | **0.420** | | **0.167** |
| $\boldsymbol{\epsilon}_{\mathbf{MAX}}(\%)$ | | | | **2.222** | | **0.635** |

**Table 5c.** Key properties of the radial distribution function resulting from molecular dynamics (MD) simulations and from two versions of the isomorph-based empirically modified hypernetted chain (IEMHNC) approach: the version constructed with the OCP bridge function given by Iyetomi, Ogata and Ichimaru (IOI) in *H. Iyetomi, S. Ogata and S. Ichimaru, Phys. Rev. A* **46**, *1051 (1992)* and the version constructed with the new OCP bridge function parameterization proposed by the authors (LCT). The absolute relative deviation $\epsilon_{\mathrm{r}}$ between the theoretical and the simulation results is also reported together with its average and maximum values (the average deviation is denoted as $\epsilon_{\mathrm{AVE}}$ and the maximum deviation is denoted as $\epsilon_{\mathrm{MAX}}$). **Results for the position of the first non-zero minimum in the case of $\boldsymbol{\kappa = 2.0}$**. The MD results are adopted from *T. Ott and M. Bonitz, Contrib. Plasma Phys.* **55**, *243 (2015)*. Here $x = r/d$, where $d$ is the Wigner-Seitz radius.

| $\Gamma$ | $\Gamma/\Gamma_m$ | $x_{\mathrm{min1}}^{\mathrm{MD}}$ | $x_{\mathrm{min1}}^{\mathrm{IOI}}$ | $\epsilon_{\mathrm{IOI}}(\%)$ | $x_{\mathrm{min1}}^{\mathrm{LCT}}$ | $\epsilon_{\mathrm{LCT}}(\%)$ |
|---|---|---|---|---|---|---|
| 30.0 | 0.07 | 2.409 | 2.438 | 1.204 | 2.406 | 0.125 |
| 40.0 | 0.09 | 2.408 | 2.441 | 1.370 | 2.407 | 0.042 |
| 50.0 | 0.11 | 2.414 | 2.439 | 1.036 | 2.413 | 0.041 |
| 60.0 | 0.13 | 2.419 | 2.438 | 0.785 | 2.419 | 0.000 |
| 70.0 | 0.15 | 2.422 | 2.438 | 0.661 | 2.424 | 0.083 |
| 80.0 | 0.17 | 2.427 | 2.439 | 0.494 | 2.428 | 0.041 |
| 90.0 | 0.20 | 2.428 | 2.439 | 0.453 | 2.431 | 0.124 |
| 100.0 | 0.22 | 2.431 | 2.440 | 0.370 | 2.433 | 0.082 |
| 110.0 | 0.24 | 2.432 | 2.440 | 0.329 | 2.434 | 0.082 |
| 120.0 | 0.26 | 2.434 | 2.440 | 0.247 | 2.435 | 0.041 |
| 130.0 | 0.28 | 2.433 | 2.440 | 0.288 | 2.435 | 0.082 |
| 140.0 | 0.31 | 2.434 | 2.440 | 0.247 | 2.435 | 0.041 |
| 150.0 | 0.33 | 2.434 | 2.440 | 0.247 | 2.435 | 0.041 |
| 160.0 | 0.35 | 2.433 | 2.439 | 0.247 | 2.434 | 0.041 |
| 170.0 | 0.37 | 2.435 | 2.438 | 0.123 | 2.433 | 0.082 |
| 180.0 | 0.39 | 2.433 | 2.437 | 0.164 | 2.432 | 0.041 |
| 190.0 | 0.41 | 2.432 | 2.436 | 0.164 | 2.431 | 0.041 |
| 200.0 | 0.44 | 2.433 | 2.435 | 0.082 | 2.430 | 0.123 |
| 210.0 | 0.46 | 2.432 | 2.434 | 0.082 | 2.429 | 0.123 |
| 220.0 | 0.48 | 2.430 | 2.433 | 0.123 | 2.428 | 0.082 |
| 230.0 | 0.50 | 2.429 | 2.432 | 0.124 | 2.426 | 0.124 |
| 240.0 | 0.52 | 2.429 | 2.431 | 0.082 | 2.425 | 0.165 |
| 250.0 | 0.55 | 2.429 | 2.429 | 0.000 | 2.424 | 0.206 |
| 260.0 | 0.57 | 2.426 | 2.428 | 0.082 | 2.422 | 0.165 |
| 270.0 | 0.59 | 2.427 | 2.427 | 0.000 | 2.421 | 0.247 |
| 280.0 | 0.61 | 2.426 | 2.426 | 0.000 | 2.420 | 0.247 |
| 290.0 | 0.63 | 2.423 | 2.424 | 0.041 | 2.419 | 0.165 |
| 300.0 | 0.65 | 2.424 | 2.423 | 0.041 | 2.417 | 0.289 |
| 310.0 | 0.68 | 2.424 | 2.422 | 0.083 | 2.416 | 0.330 |
| 320.0 | 0.70 | 2.421 | 2.421 | 0.000 | 2.415 | 0.248 |
| 330.0 | 0.72 | 2.421 | 2.420 | 0.041 | 2.414 | 0.289 |
| 340.0 | 0.74 | 2.421 | 2.418 | 0.124 | 2.412 | 0.372 |
| 350.0 | 0.76 | 2.419 | 2.417 | 0.083 | 2.411 | 0.331 |
| 360.0 | 0.79 | 2.418 | 2.416 | 0.083 | 2.410 | 0.331 |
| 370.0 | 0.81 | 2.417 | 2.415 | 0.083 | 2.409 | 0.331 |
| 380.0 | 0.83 | 2.417 | 2.414 | 0.124 | 2.408 | 0.372 |
| 390.0 | 0.85 | 2.416 | 2.413 | 0.124 | 2.407 | 0.373 |
| 400.0 | 0.87 | 2.415 | 2.412 | 0.124 | 2.406 | 0.373 |
| $\boldsymbol{\epsilon_{\mathrm{AVE}}}(\%)$ | | | | **0.262** | | **0.166** |
| $\boldsymbol{\epsilon_{\mathrm{MAX}}}(\%)$ | | | | **1.370** | | **0.373** |

**Table 6a.** Key properties of the radial distribution function resulting from molecular dynamics (MD) simulations and from two versions of the isomorph-based empirically modified hypernetted chain (IEMHNC) approach: the version constructed with the OCP bridge function given by Iyetomi, Ogata and Ichimaru (IOI) in *H. Iyetomi, S. Ogata and S. Ichimaru, Phys. Rev. A* **46**, *1051 (1992)* and the version constructed with the new OCP bridge function parameterization proposed by the authors (LCT). The absolute relative deviation $\epsilon_{\mathrm{r}}$ between the theoretical and the simulation results is also reported together with its average and maximum values (the average deviation is denoted as $\epsilon_{\mathrm{AVE}}$ and the maximum deviation is denoted as $\epsilon_{\mathrm{MAX}}$). **Results for the magnitude of the second maximum in the case of** $\boldsymbol{\kappa = 0.0}$. The MD results are adopted from *T. Ott and M. Bonitz, Contrib. Plasma Phys.* **55**, *243 (2015)*.

| $\Gamma$ | $\Gamma/\Gamma_m$ | $g_{\mathrm{max2}}^{\mathrm{MD}}$ | $g_{\mathrm{max2}}^{\mathrm{IOI}}$ | $\epsilon_{\mathrm{IOI}}(\%)$ | $g_{\mathrm{max2}}^{\mathrm{LCT}}$ | $\epsilon_{\mathrm{LCT}}(\%)$ |
|---|---|---|---|---|---|---|
| 15.0 | 0.09 | 1.012 | 1.010 | 0.189 | 1.012 | 0.025 |
| 20.0 | 0.12 | 1.023 | 1.019 | 0.369 | 1.023 | 0.047 |
| 25.0 | 0.15 | 1.035 | 1.030 | 0.493 | 1.035 | 0.014 |
| 30.0 | 0.17 | 1.047 | 1.042 | 0.523 | 1.048 | 0.094 |
| 35.0 | 0.20 | 1.060 | 1.054 | 0.597 | 1.061 | 0.138 |
| 40.0 | 0.23 | 1.073 | 1.066 | 0.645 | 1.075 | 0.189 |
| 45.0 | 0.26 | 1.085 | 1.079 | 0.590 | 1.089 | 0.327 |
| 50.0 | 0.29 | 1.098 | 1.091 | 0.627 | 1.102 | 0.356 |
| 55.0 | 0.32 | 1.110 | 1.104 | 0.580 | 1.115 | 0.455 |
| 60.0 | 0.35 | 1.122 | 1.116 | 0.542 | 1.128 | 0.530 |
| 65.0 | 0.38 | 1.133 | 1.128 | 0.429 | 1.141 | 0.668 |
| 70.0 | 0.41 | 1.145 | 1.140 | 0.419 | 1.153 | 0.691 |
| 75.0 | 0.44 | 1.156 | 1.152 | 0.338 | 1.165 | 0.775 |
| 80.0 | 0.47 | 1.166 | 1.164 | 0.188 | 1.177 | 0.919 |
| 85.0 | 0.49 | 1.176 | 1.175 | 0.056 | 1.188 | 1.036 |
| 90.0 | 0.52 | 1.186 | 1.187 | 0.057 | 1.199 | 1.126 |
| 95.0 | 0.55 | 1.196 | 1.198 | 0.152 | 1.210 | 1.191 |
| 100.0 | 0.58 | 1.205 | 1.209 | 0.311 | 1.221 | 1.315 |
| 105.0 | 0.61 | 1.213 | 1.219 | 0.535 | 1.231 | 1.497 |
| 110.0 | 0.64 | 1.222 | 1.230 | 0.658 | 1.241 | 1.570 |
| 115.0 | 0.67 | 1.231 | 1.240 | 0.761 | 1.251 | 1.621 |
| 120.0 | 0.70 | 1.238 | 1.251 | 1.011 | 1.260 | 1.812 |
| 125.0 | 0.73 | 1.246 | 1.260 | 1.159 | 1.270 | 1.896 |
| 130.0 | 0.76 | 1.253 | 1.270 | 1.371 | 1.279 | 2.039 |
| 135.0 | 0.79 | 1.260 | 1.280 | 1.565 | 1.287 | 2.158 |
| 140.0 | 0.81 | 1.267 | 1.289 | 1.741 | 1.296 | 2.254 |
| 145.0 | 0.84 | 1.273 | 1.298 | 1.980 | 1.304 | 2.408 |
| 150.0 | 0.87 | 1.279 | 1.307 | 2.202 | 1.311 | 2.538 |
| 155.0 | 0.90 | 1.285 | 1.316 | 2.407 | 1.319 | 2.644 |
| 160.0 | 0.93 | 1.291 | 1.324 | 2.594 | 1.326 | 2.727 |
| 165.0 | 0.96 | 1.297 | 1.333 | 2.766 | 1.333 | 2.787 |
| $\boldsymbol{\epsilon_{\mathrm{AVE}}}(\%)$ | | | | **0.899** | | **1.221** |
| $\boldsymbol{\epsilon_{\mathrm{MAX}}}(\%)$ | | | | **2.766** | | **2.787** |

**Table 6b.** Key properties of the radial distribution function resulting from molecular dynamics (MD) simulations and from two versions of the isomorph-based empirically modified hypernetted chain (IEMHNC) approach: the version constructed with the OCP bridge function given by Iyetomi, Ogata and Ichimaru (IOI) in *H. Iyetomi, S. Ogata and S. Ichimaru, Phys. Rev. A* **46**, *1051 (1992)* and the version constructed with the new OCP bridge function parameterization proposed by the authors (LCT). The absolute relative deviation $\epsilon_{\mathrm{r}}$ between the theoretical and the simulation results is also reported together with its average and maximum values (the average deviation is denoted as $\epsilon_{\mathrm{AVE}}$ and the maximum deviation is denoted as $\epsilon_{\mathrm{MAX}}$). **Results for the magnitude of the second maximum in the case of $\boldsymbol{\kappa = 1.0}$**. The MD results are adopted from *T. Ott and M. Bonitz, Contrib. Plasma Phys.* **55**, *243 (2015)*.

| $\Gamma$ | $\Gamma/\Gamma_m$ | $g_{\mathrm{max2}}^{\mathrm{MD}}$ | $g_{\mathrm{max2}}^{\mathrm{IOI}}$ | $\epsilon_{\mathrm{IOI}}(\%)$ | $g_{\mathrm{max2}}^{\mathrm{LCT}}$ | $\epsilon_{\mathrm{LCT}}(\%)$ |
|---|---|---|---|---|---|---|
| 10.0 | 0.05 | 1.002 | 1.001 | 0.093 | 1.002 | 0.005 |
| 15.0 | 0.07 | 1.007 | 1.005 | 0.152 | 1.007 | 0.033 |
| 20.0 | 0.09 | 1.014 | 1.012 | 0.245 | 1.014 | 0.027 |
| 25.0 | 0.11 | 1.022 | 1.019 | 0.309 | 1.022 | 0.036 |
| 30.0 | 0.14 | 1.031 | 1.027 | 0.372 | 1.032 | 0.093 |
| 35.0 | 0.16 | 1.041 | 1.036 | 0.466 | 1.042 | 0.108 |
| 40.0 | 0.18 | 1.050 | 1.046 | 0.424 | 1.053 | 0.248 |
| 45.0 | 0.20 | 1.060 | 1.055 | 0.453 | 1.063 | 0.306 |
| 50.0 | 0.23 | 1.070 | 1.065 | 0.468 | 1.074 | 0.367 |
| 55.0 | 0.25 | 1.080 | 1.075 | 0.477 | 1.085 | 0.425 |
| 60.0 | 0.27 | 1.090 | 1.085 | 0.485 | 1.095 | 0.475 |
| 65.0 | 0.30 | 1.100 | 1.095 | 0.495 | 1.106 | 0.513 |
| 70.0 | 0.32 | 1.109 | 1.104 | 0.420 | 1.116 | 0.629 |
| 75.0 | 0.34 | 1.118 | 1.114 | 0.352 | 1.126 | 0.729 |
| 80.0 | 0.36 | 1.127 | 1.124 | 0.292 | 1.136 | 0.812 |
| 85.0 | 0.39 | 1.137 | 1.133 | 0.330 | 1.146 | 0.789 |
| 90.0 | 0.41 | 1.145 | 1.143 | 0.201 | 1.156 | 0.928 |
| 95.0 | 0.43 | 1.153 | 1.152 | 0.084 | 1.165 | 1.048 |
| 100.0 | 0.45 | 1.162 | 1.161 | 0.064 | 1.174 | 1.064 |
| 105.0 | 0.48 | 1.170 | 1.170 | 0.031 | 1.183 | 1.151 |
| 110.0 | 0.50 | 1.178 | 1.179 | 0.115 | 1.192 | 1.221 |
| 115.0 | 0.52 | 1.185 | 1.188 | 0.272 | 1.201 | 1.360 |
| 120.0 | 0.54 | 1.193 | 1.197 | 0.332 | 1.210 | 1.398 |
| 125.0 | 0.57 | 1.200 | 1.206 | 0.466 | 1.218 | 1.505 |
| 130.0 | 0.59 | 1.207 | 1.214 | 0.587 | 1.226 | 1.596 |
| 135.0 | 0.61 | 1.214 | 1.222 | 0.697 | 1.234 | 1.672 |
| 140.0 | 0.64 | 1.220 | 1.231 | 0.877 | 1.242 | 1.815 |
| 145.0 | 0.66 | 1.227 | 1.239 | 0.964 | 1.250 | 1.861 |
| 150.0 | 0.68 | 1.233 | 1.247 | 1.122 | 1.257 | 1.974 |
| 155.0 | 0.70 | 1.239 | 1.255 | 1.267 | 1.265 | 2.073 |
| 160.0 | 0.73 | 1.246 | 1.262 | 1.321 | 1.272 | 2.074 |
| 165.0 | 0.75 | 1.251 | 1.270 | 1.525 | 1.279 | 2.226 |
| 170.0 | 0.77 | 1.256 | 1.278 | 1.718 | 1.286 | 2.363 |
| 175.0 | 0.79 | 1.262 | 1.285 | 1.820 | 1.292 | 2.404 |
| 180.0 | 0.82 | 1.267 | 1.292 | 1.991 | 1.299 | 2.512 |
| 185.0 | 0.84 | 1.272 | 1.299 | 2.151 | 1.305 | 2.605 |
| 190.0 | 0.86 | 1.277 | 1.306 | 2.301 | 1.311 | 2.685 |
| 195.0 | 0.89 | 1.281 | 1.313 | 2.520 | 1.317 | 2.830 |
| 200.0 | 0.91 | 1.286 | 1.320 | 2.649 | 1.323 | 2.880 |
| $\boldsymbol{\epsilon_{\mathrm{AVE}}}(\%)$ | | | | **0.793** | | **1.252** |
| $\boldsymbol{\epsilon_{\mathrm{MAX}}}(\%)$ | | | | **2.649** | | **2.880** |

**Table 6c.** Key properties of the radial distribution function resulting from molecular dynamics (MD) simulations and from two versions of the isomorph-based empirically modified hypernetted chain (IEMHNC) approach: the version constructed with the OCP bridge function given by Iyetomi, Ogata and Ichimaru (IOI) in *H. Iyetomi, S. Ogata and S. Ichimaru, Phys. Rev. A* **46**, *1051 (1992)* and the version constructed with the new OCP bridge function parameterization proposed by the authors (LCT). The absolute relative deviation $\epsilon_{\mathrm{r}}$ between the theoretical and the simulation results is also reported together with its average and maximum values (the average deviation is denoted as $\epsilon_{\mathrm{AVE}}$ and the maximum deviation is denoted as $\epsilon_{\mathrm{MAX}}$). **Results for the magnitude of the second maximum in the case of $\boldsymbol{\kappa = 2.0}$**. The MD results are adopted from *T. Ott and M. Bonitz, Contrib. Plasma Phys.* **55**, *243 (2015)*.

| $\Gamma$ | $\Gamma/\Gamma_m$ | $g_{\mathrm{max2}}^{\mathrm{MD}}$ | $g_{\mathrm{max2}}^{\mathrm{IOI}}$ | $\epsilon_{\mathrm{IOI}}(\%)$ | $g_{\mathrm{max2}}^{\mathrm{LCT}}$ | $\epsilon_{\mathrm{LCT}}(\%)$ |
|---|---|---|---|---|---|---|
| 30.0 | 0.07 | 1.008 | 1.007 | 0.126 | 1.008 | 0.046 |
| 40.0 | 0.09 | 1.016 | 1.013 | 0.270 | 1.016 | 0.020 |
| 50.0 | 0.11 | 1.025 | 1.021 | 0.381 | 1.025 | 0.027 |
| 60.0 | 0.13 | 1.034 | 1.030 | 0.399 | 1.035 | 0.113 |
| 70.0 | 0.15 | 1.044 | 1.039 | 0.456 | 1.046 | 0.148 |
| 80.0 | 0.17 | 1.054 | 1.049 | 0.480 | 1.056 | 0.208 |
| 90.0 | 0.20 | 1.064 | 1.059 | 0.487 | 1.067 | 0.279 |
| 100.0 | 0.22 | 1.074 | 1.069 | 0.486 | 1.078 | 0.350 |
| 110.0 | 0.24 | 1.084 | 1.079 | 0.483 | 1.089 | 0.417 |
| 120.0 | 0.26 | 1.093 | 1.089 | 0.391 | 1.099 | 0.565 |
| 130.0 | 0.28 | 1.103 | 1.099 | 0.396 | 1.110 | 0.608 |
| 140.0 | 0.31 | 1.113 | 1.108 | 0.407 | 1.120 | 0.637 |
| 150.0 | 0.33 | 1.122 | 1.118 | 0.338 | 1.130 | 0.740 |
| 160.0 | 0.35 | 1.131 | 1.128 | 0.278 | 1.140 | 0.825 |
| 170.0 | 0.37 | 1.140 | 1.137 | 0.229 | 1.150 | 0.892 |
| 180.0 | 0.39 | 1.149 | 1.147 | 0.191 | 1.160 | 0.942 |
| 190.0 | 0.41 | 1.158 | 1.156 | 0.164 | 1.169 | 0.975 |
| 200.0 | 0.44 | 1.165 | 1.165 | 0.024 | 1.179 | 1.163 |
| 210.0 | 0.46 | 1.173 | 1.174 | 0.113 | 1.188 | 1.248 |
| 220.0 | 0.48 | 1.181 | 1.183 | 0.191 | 1.197 | 1.315 |
| 230.0 | 0.50 | 1.189 | 1.192 | 0.256 | 1.205 | 1.365 |
| 240.0 | 0.52 | 1.196 | 1.201 | 0.394 | 1.214 | 1.485 |
| 250.0 | 0.55 | 1.204 | 1.209 | 0.436 | 1.222 | 1.503 |
| 260.0 | 0.57 | 1.210 | 1.218 | 0.633 | 1.230 | 1.675 |
| 270.0 | 0.59 | 1.217 | 1.226 | 0.734 | 1.238 | 1.746 |
| 280.0 | 0.61 | 1.224 | 1.234 | 0.825 | 1.246 | 1.803 |
| 290.0 | 0.63 | 1.230 | 1.242 | 0.985 | 1.254 | 1.928 |
| 300.0 | 0.65 | 1.236 | 1.250 | 1.134 | 1.261 | 2.037 |
| 310.0 | 0.68 | 1.243 | 1.258 | 1.189 | 1.268 | 2.050 |
| 320.0 | 0.70 | 1.248 | 1.265 | 1.396 | 1.276 | 2.213 |
| 330.0 | 0.72 | 1.254 | 1.273 | 1.511 | 1.283 | 2.280 |
| 340.0 | 0.74 | 1.259 | 1.280 | 1.695 | 1.289 | 2.414 |
| 350.0 | 0.76 | 1.264 | 1.288 | 1.868 | 1.296 | 2.533 |
| 360.0 | 0.79 | 1.270 | 1.295 | 1.950 | 1.302 | 2.558 |
| 370.0 | 0.81 | 1.275 | 1.302 | 2.102 | 1.309 | 2.651 |
| 380.0 | 0.83 | 1.279 | 1.309 | 2.323 | 1.315 | 2.810 |
| 390.0 | 0.85 | 1.283 | 1.315 | 2.533 | 1.321 | 2.955 |
| 400.0 | 0.87 | 1.288 | 1.322 | 2.653 | 1.327 | 3.006 |
| $\boldsymbol{\epsilon_{\mathrm{AVE}}(\%)}$ | | | | **0.813** | | **1.330** |
| $\boldsymbol{\epsilon_{\mathrm{MAX}}(\%)}$ | | | | **2.653** | | **3.006** |

**Table 7a.** Key properties of the radial distribution function resulting from molecular dynamics (MD) simulations and from two versions of the isomorph-based empirically modified hypernetted chain (IEMHNC) approach: the version constructed with the OCP bridge function given by Iyetomi, Ogata and Ichimaru (IOI) in *H. Iyetomi, S. Ogata and S. Ichimaru, Phys. Rev. A* **46**, *1051 (1992)* and the version constructed with the new OCP bridge function parameterization proposed by the authors (LCT). The absolute relative deviation $\epsilon_{\mathrm{r}}$ between the theoretical and the simulation results is also reported together with its average and maximum values (the average deviation is denoted as $\epsilon_{\mathrm{AVE}}$ and the maximum deviation is denoted as $\epsilon_{\mathrm{MAX}}$). **Results for the position of the second maximum in the case of $\boldsymbol{\kappa = 0.0}$.** The MD results are adopted from *T. Ott and M. Bonitz, Contrib. Plasma Phys.* **55**, *243 (2015)*. Here $x = r/d$, where $d$ is the Wigner-Seitz radius.

| $\Gamma$ | $\Gamma/\Gamma_m$ | $x_{\mathrm{max2}}^{\mathrm{MD}}$ | $x_{\mathrm{max2}}^{\mathrm{IOI}}$ | $\epsilon_{\mathrm{IOI}}(\%)$ | $x_{\mathrm{max2}}^{\mathrm{LCT}}$ | $\epsilon_{\mathrm{LCT}}(\%)$ |
|---|---|---|---|---|---|---|
| 15.0 | 0.09 | 3.298 | 3.384 | 2.608 | 3.306 | 0.243 |
| 20.0 | 0.12 | 3.278 | 3.332 | 1.647 | 3.277 | 0.031 |
| 25.0 | 0.15 | 3.259 | 3.300 | 1.258 | 3.263 | 0.123 |
| 30.0 | 0.17 | 3.248 | 3.280 | 0.985 | 3.254 | 0.185 |
| 35.0 | 0.20 | 3.244 | 3.267 | 0.709 | 3.248 | 0.123 |
| 40.0 | 0.23 | 3.240 | 3.259 | 0.586 | 3.243 | 0.093 |
| 45.0 | 0.26 | 3.238 | 3.253 | 0.463 | 3.240 | 0.062 |
| 50.0 | 0.29 | 3.236 | 3.249 | 0.402 | 3.237 | 0.031 |
| 55.0 | 0.32 | 3.235 | 3.247 | 0.371 | 3.236 | 0.031 |
| 60.0 | 0.35 | 3.233 | 3.245 | 0.371 | 3.234 | 0.031 |
| 65.0 | 0.38 | 3.234 | 3.244 | 0.309 | 3.234 | 0.000 |
| 70.0 | 0.41 | 3.231 | 3.243 | 0.371 | 3.233 | 0.062 |
| 75.0 | 0.44 | 3.232 | 3.243 | 0.340 | 3.233 | 0.031 |
| 80.0 | 0.47 | 3.232 | 3.243 | 0.340 | 3.233 | 0.031 |
| 85.0 | 0.49 | 3.233 | 3.243 | 0.309 | 3.234 | 0.031 |
| 90.0 | 0.52 | 3.234 | 3.244 | 0.309 | 3.234 | 0.000 |
| 95.0 | 0.55 | 3.232 | 3.244 | 0.371 | 3.235 | 0.093 |
| 100.0 | 0.58 | 3.232 | 3.245 | 0.402 | 3.236 | 0.124 |
| 105.0 | 0.61 | 3.233 | 3.246 | 0.402 | 3.237 | 0.124 |
| 110.0 | 0.64 | 3.233 | 3.246 | 0.402 | 3.238 | 0.155 |
| 115.0 | 0.67 | 3.233 | 3.247 | 0.433 | 3.238 | 0.155 |
| 120.0 | 0.70 | 3.234 | 3.248 | 0.433 | 3.239 | 0.155 |
| 125.0 | 0.73 | 3.233 | 3.249 | 0.495 | 3.240 | 0.217 |
| 130.0 | 0.76 | 3.233 | 3.250 | 0.526 | 3.241 | 0.247 |
| 135.0 | 0.79 | 3.235 | 3.251 | 0.495 | 3.242 | 0.216 |
| 140.0 | 0.81 | 3.234 | 3.252 | 0.557 | 3.243 | 0.278 |
| 145.0 | 0.84 | 3.235 | 3.253 | 0.556 | 3.244 | 0.278 |
| 150.0 | 0.87 | 3.235 | 3.254 | 0.587 | 3.244 | 0.278 |
| 155.0 | 0.90 | 3.235 | 3.255 | 0.618 | 3.245 | 0.309 |
| 160.0 | 0.93 | 3.235 | 3.256 | 0.649 | 3.246 | 0.340 |
| 165.0 | 0.96 | 3.234 | 3.257 | 0.711 | 3.246 | 0.371 |
| $\boldsymbol{\epsilon_{\mathrm{AVE}}}(\%)$ | | | | **0.613** | | **0.143** |
| $\boldsymbol{\epsilon_{\mathrm{MAX}}}(\%)$ | | | | **2.608** | | **0.371** |

**Table 7b.** Key properties of the radial distribution function resulting from molecular dynamics (MD) simulations and from two versions of the isomorph-based empirically modified hypernetted chain (IEMHNC) approach: the version constructed with the OCP bridge function given by Iyetomi, Ogata and Ichimaru (IOI) in *H. Iyetomi, S. Ogata and S. Ichimaru, Phys. Rev. A* **46**, *1051 (1992)* and the version constructed with the new OCP bridge function parameterization proposed by the authors (LCT). The absolute relative deviation $\epsilon_{\mathrm{r}}$ between the theoretical and the simulation results is also reported together with its average and maximum values (the average deviation is denoted as $\epsilon_{\mathrm{AVE}}$ and the maximum deviation is denoted as $\epsilon_{\mathrm{MAX}}$). **Results for the position of the second maximum in the case of $\boldsymbol{\kappa = 1.0}$.** The MD results are adopted from *T. Ott and M. Bonitz, Contrib. Plasma Phys.* **55**, *243 (2015)*. Here $x = r/d$, where $d$ is the Wigner-Seitz radius.

| $\Gamma$ | $\Gamma/\Gamma_m$ | $x_{\mathrm{max2}}^{\mathrm{MD}}$ | $x_{\mathrm{max2}}^{\mathrm{IOI}}$ | $\epsilon_{\mathrm{IOI}}(\%)$ | $x_{\mathrm{max2}}^{\mathrm{LCT}}$ | $\epsilon_{\mathrm{LCT}}(\%)$ |
|---|---|---|---|---|---|---|
| 10.0 | 0.05 | 3.437 | 3.480 | 1.251 | 3.408 | 0.844 |
| 15.0 | 0.07 | 3.322 | 3.378 | 1.686 | 3.303 | 0.572 |
| 20.0 | 0.09 | 3.277 | 3.336 | 1.800 | 3.266 | 0.336 |
| 25.0 | 0.11 | 3.253 | 3.303 | 1.537 | 3.250 | 0.092 |
| 30.0 | 0.14 | 3.241 | 3.281 | 1.234 | 3.243 | 0.062 |
| 35.0 | 0.16 | 3.236 | 3.266 | 0.927 | 3.238 | 0.062 |
| 40.0 | 0.18 | 3.237 | 3.256 | 0.587 | 3.234 | 0.093 |
| 45.0 | 0.20 | 3.230 | 3.249 | 0.588 | 3.232 | 0.062 |
| 50.0 | 0.23 | 3.228 | 3.244 | 0.496 | 3.230 | 0.062 |
| 55.0 | 0.25 | 3.228 | 3.240 | 0.372 | 3.228 | 0.000 |
| 60.0 | 0.27 | 3.224 | 3.238 | 0.434 | 3.227 | 0.093 |
| 65.0 | 0.30 | 3.227 | 3.236 | 0.279 | 3.226 | 0.031 |
| 70.0 | 0.32 | 3.224 | 3.235 | 0.341 | 3.225 | 0.031 |
| 75.0 | 0.34 | 3.226 | 3.234 | 0.248 | 3.225 | 0.031 |
| 80.0 | 0.36 | 3.224 | 3.234 | 0.310 | 3.224 | 0.000 |
| 85.0 | 0.39 | 3.225 | 3.234 | 0.279 | 3.225 | 0.000 |
| 90.0 | 0.41 | 3.224 | 3.234 | 0.310 | 3.225 | 0.031 |
| 95.0 | 0.43 | 3.224 | 3.234 | 0.310 | 3.225 | 0.031 |
| 100.0 | 0.45 | 3.226 | 3.235 | 0.279 | 3.226 | 0.000 |
| 105.0 | 0.48 | 3.226 | 3.235 | 0.279 | 3.226 | 0.000 |
| 110.0 | 0.50 | 3.226 | 3.236 | 0.310 | 3.227 | 0.031 |
| 115.0 | 0.52 | 3.227 | 3.236 | 0.279 | 3.228 | 0.031 |
| 120.0 | 0.54 | 3.227 | 3.237 | 0.310 | 3.229 | 0.062 |
| 125.0 | 0.57 | 3.227 | 3.238 | 0.341 | 3.229 | 0.062 |
| 130.0 | 0.59 | 3.227 | 3.239 | 0.372 | 3.230 | 0.093 |
| 135.0 | 0.61 | 3.227 | 3.240 | 0.403 | 3.231 | 0.124 |
| 140.0 | 0.64 | 3.228 | 3.241 | 0.403 | 3.232 | 0.124 |
| 145.0 | 0.66 | 3.228 | 3.241 | 0.403 | 3.233 | 0.155 |
| 150.0 | 0.68 | 3.229 | 3.242 | 0.403 | 3.234 | 0.155 |
| 155.0 | 0.70 | 3.228 | 3.243 | 0.465 | 3.235 | 0.217 |
| 160.0 | 0.73 | 3.228 | 3.244 | 0.496 | 3.236 | 0.248 |
| 165.0 | 0.75 | 3.229 | 3.245 | 0.496 | 3.236 | 0.217 |
| 170.0 | 0.77 | 3.229 | 3.246 | 0.526 | 3.237 | 0.248 |
| 175.0 | 0.79 | 3.230 | 3.247 | 0.526 | 3.238 | 0.248 |
| 180.0 | 0.82 | 3.230 | 3.248 | 0.557 | 3.239 | 0.279 |
| 185.0 | 0.84 | 3.231 | 3.249 | 0.557 | 3.240 | 0.279 |
| 190.0 | 0.86 | 3.230 | 3.250 | 0.619 | 3.240 | 0.310 |
| 195.0 | 0.89 | 3.231 | 3.251 | 0.619 | 3.241 | 0.310 |
| 200.0 | 0.91 | 3.232 | 3.252 | 0.619 | 3.242 | 0.309 |
| $\boldsymbol{\epsilon_{\mathrm{AVE}}}(\%)$ | | | | **0.571** | | **0.152** |
| $\boldsymbol{\epsilon_{\mathrm{MAX}}}(\%)$ | | | | **1.800** | | **0.844** |

**Table 7c.** Key properties of the radial distribution function resulting from molecular dynamics (MD) simulations and from two versions of the isomorph-based empirically modified hypernetted chain (IEMHNC) approach: the version constructed with the OCP bridge function given by Iyetomi, Ogata and Ichimaru (IOI) in *H. Iyetomi, S. Ogata and S. Ichimaru, Phys. Rev. A* **46**, *1051 (1992)* and the version constructed with the new OCP bridge function parameterization proposed by the authors (LCT). The absolute relative deviation $\epsilon_{\mathrm{r}}$ between the theoretical and the simulation results is also reported together with its average and maximum values (the average deviation is denoted as $\epsilon_{\mathrm{AVE}}$ and the maximum deviation is denoted as $\epsilon_{\mathrm{MAX}}$). **Results for the position of the second maximum in the case of $\boldsymbol{\kappa = 2.0}$.** The MD results are adopted from *T. Ott and M. Bonitz, Contrib. Plasma Phys.* **55**, *243 (2015)*. Here $x = r/d$, where $d$ is the Wigner-Seitz radius.

| $\Gamma$ | $\Gamma/\Gamma_m$ | $x^{\mathrm{MD}}_{\mathrm{max2}}$ | $x^{\mathrm{IOI}}_{\mathrm{max2}}$ | $\epsilon_{\mathrm{IOI}}(\%)$ | $x^{\mathrm{LCT}}_{\mathrm{max2}}$ | $\epsilon_{\mathrm{LCT}}(\%)$ |
|---|---|---|---|---|---|---|
| 30.0 | 0.07 | 3.213 | 3.255 | 1.307 | 3.204 | 0.280 |
| 40.0 | 0.09 | 3.199 | 3.245 | 1.438 | 3.191 | 0.250 |
| 50.0 | 0.11 | 3.193 | 3.231 | 1.190 | 3.189 | 0.125 |
| 60.0 | 0.13 | 3.192 | 3.220 | 0.877 | 3.191 | 0.031 |
| 70.0 | 0.15 | 3.196 | 3.214 | 0.563 | 3.193 | 0.094 |
| 80.0 | 0.17 | 3.193 | 3.210 | 0.532 | 3.195 | 0.063 |
| 90.0 | 0.20 | 3.194 | 3.208 | 0.438 | 3.196 | 0.063 |
| 100.0 | 0.22 | 3.194 | 3.207 | 0.407 | 3.197 | 0.094 |
| 110.0 | 0.24 | 3.198 | 3.206 | 0.250 | 3.198 | 0.000 |
| 120.0 | 0.26 | 3.198 | 3.206 | 0.250 | 3.199 | 0.031 |
| 130.0 | 0.28 | 3.200 | 3.207 | 0.219 | 3.200 | 0.000 |
| 140.0 | 0.31 | 3.201 | 3.208 | 0.219 | 3.201 | 0.000 |
| 150.0 | 0.33 | 3.201 | 3.209 | 0.250 | 3.202 | 0.031 |
| 160.0 | 0.35 | 3.205 | 3.210 | 0.156 | 3.204 | 0.031 |
| 170.0 | 0.37 | 3.203 | 3.211 | 0.250 | 3.205 | 0.062 |
| 180.0 | 0.39 | 3.207 | 3.213 | 0.187 | 3.206 | 0.031 |
| 190.0 | 0.41 | 3.206 | 3.214 | 0.250 | 3.207 | 0.031 |
| 200.0 | 0.44 | 3.207 | 3.215 | 0.249 | 3.209 | 0.062 |
| 210.0 | 0.46 | 3.209 | 3.217 | 0.249 | 3.210 | 0.031 |
| 220.0 | 0.48 | 3.210 | 3.218 | 0.249 | 3.212 | 0.062 |
| 230.0 | 0.50 | 3.211 | 3.220 | 0.280 | 3.213 | 0.062 |
| 240.0 | 0.52 | 3.211 | 3.221 | 0.311 | 3.214 | 0.093 |
| 250.0 | 0.55 | 3.212 | 3.223 | 0.342 | 3.216 | 0.125 |
| 260.0 | 0.57 | 3.212 | 3.224 | 0.374 | 3.217 | 0.156 |
| 270.0 | 0.59 | 3.213 | 3.226 | 0.405 | 3.219 | 0.187 |
| 280.0 | 0.61 | 3.214 | 3.227 | 0.404 | 3.220 | 0.187 |
| 290.0 | 0.63 | 3.214 | 3.228 | 0.436 | 3.221 | 0.218 |
| 300.0 | 0.65 | 3.216 | 3.230 | 0.435 | 3.223 | 0.218 |
| 310.0 | 0.68 | 3.216 | 3.231 | 0.466 | 3.224 | 0.249 |
| 320.0 | 0.70 | 3.216 | 3.233 | 0.529 | 3.225 | 0.280 |
| 330.0 | 0.72 | 3.218 | 3.234 | 0.497 | 3.226 | 0.249 |
| 340.0 | 0.74 | 3.218 | 3.235 | 0.528 | 3.227 | 0.280 |
| 350.0 | 0.76 | 3.218 | 3.237 | 0.590 | 3.229 | 0.342 |
| 360.0 | 0.79 | 3.220 | 3.238 | 0.559 | 3.230 | 0.311 |
| 370.0 | 0.81 | 3.219 | 3.239 | 0.621 | 3.231 | 0.373 |
| 380.0 | 0.83 | 3.221 | 3.240 | 0.590 | 3.232 | 0.342 |
| 390.0 | 0.85 | 3.221 | 3.242 | 0.652 | 3.233 | 0.373 |
| 400.0 | 0.87 | 3.221 | 3.243 | 0.683 | 3.234 | 0.404 |
| $\boldsymbol{\epsilon_{\mathrm{AVE}}}(\%)$ | | | | **0.480** | | **0.153** |
| $\boldsymbol{\epsilon_{\mathrm{MAX}}}(\%)$ | | | | **1.438** | | **0.404** |

**Table 8a.** The reduced excess internal energy due to particle-particle interactions $u_{\mathrm{ex}}^{\mathrm{pp}}$ resulting from molecular dynamics (MD) simulations and from two versions of the isomorph-based empirically modified hypernetted chain (IEMHNC) approach: the version constructed with the OCP bridge function given by Iyetomi, Ogata and Ichimaru (IOI) in *H. Iyetomi, S. Ogata and S. Ichimaru, Phys. Rev. A* **46**, *1051 (1992)* and the version constructed with the new OCP bridge function parameterization proposed by the authors (LCT). The absolute relative deviation $\epsilon_{\mathrm{r}}$ between the theoretical and the simulation results is also reported together with its average and maximum values (the average deviation is denoted as $\epsilon_{\mathrm{AVE}}$ and the maximum deviation is denoted as $\epsilon_{\mathrm{MAX}}$). **Results in the case of $\boldsymbol{\kappa = 0.0}$**. The MD results are adopted from *R. T. Farouki and S. Hamaguchi, J. Chem. Phys.* **101**, *9885 (1994)*.

| $\Gamma$ | $\Gamma/\Gamma_m$ | $u_{\mathrm{ex}}^{\mathrm{pp,MD}}$ | $u_{\mathrm{ex}}^{pp,\mathrm{pp,IOI}}$ | $\epsilon_{\mathrm{IOI}}(\%)$ | $u_{\mathrm{ex}}^{\mathrm{pp,LCT}}$ | $\epsilon_{\mathrm{LCT}}(\%)$ |
|---|---|---|---|---|---|---|
| 10.0 | 0.06 | -7.995 | -7.963 | 0.395 | -7.995 | 0.006 |
| 20.0 | 0.12 | -16.668 | -16.639 | 0.177 | -16.672 | 0.022 |
| 40.0 | 0.23 | -34.259 | -34.221 | 0.110 | -34.258 | 0.004 |
| 60.0 | 0.35 | -51.957 | -51.925 | 0.061 | -51.966 | 0.018 |
| 80.0 | 0.47 | -69.725 | -69.690 | 0.051 | -69.730 | 0.007 |
| 100.0 | 0.58 | -87.519 | -87.486 | 0.038 | -87.518 | 0.001 |
| 120.0 | 0.70 | -105.343 | -105.284 | 0.056 | -105.301 | 0.040 |
| 140.0 | 0.81 | -123.175 | -123.046 | 0.105 | -123.052 | 0.100 |
| 160.0 | 0.93 | -141.698 | -140.727 | 0.685 | -140.758 | 0.663 |
| $\boldsymbol{\epsilon_{\mathrm{AVE}}}(\%)$ | | | | **0.186** | | **0.096** |
| $\boldsymbol{\epsilon_{\mathrm{MAX}}}(\%)$ | | | | **0.685** | | **0.663** |

**Table 8b.** The reduced excess internal energy due to particle-particle interactions $u_{\mathrm{ex}}^{\mathrm{pp}}$ resulting from molecular dynamics (MD) simulations and from two versions of the isomorph-based empirically modified hypernetted chain (IEMHNC) approach: the version constructed with the OCP bridge function given by Iyetomi, Ogata and Ichimaru (IOI) in *H. Iyetomi, S. Ogata and S. Ichimaru, Phys. Rev. A* **46**, *1051 (1992)* and the version constructed with the new OCP bridge function parameterization proposed by the authors (LCT). The absolute relative deviation $\epsilon_{\mathrm{r}}$ between the theoretical and the simulation results is also reported together with its average and maximum values (the average deviation is denoted as $\epsilon_{\mathrm{AVE}}$ and the maximum deviation is denoted as $\epsilon_{\mathrm{MAX}}$). **Results in the case of $\boldsymbol{\kappa = 0.2}$**. The MD results are adopted from *R. T. Farouki and S. Hamaguchi, J. Chem. Phys.* **101**, *9885 (1994)*.

| $\Gamma$ | $\Gamma/\Gamma_m$ | $u_{\mathrm{ex}}^{\mathrm{pp,MD}}$ | $u_{\mathrm{ex}}^{pp,\mathrm{pp,IOI}}$ | $\epsilon_{\mathrm{IOI}}(\%)$ | $u_{\mathrm{ex}}^{\mathrm{pp,LCT}}$ | $\epsilon_{\mathrm{LCT}}(\%)$ |
|---|---|---|---|---|---|---|
| 10.0 | 0.06 | 367.955 | 367.990 | 0.010 | 367.958 | 0.001 |
| 20.0 | 0.12 | 735.243 | 735.272 | 0.004 | 735.239 | 0.001 |
| 40.0 | 0.23 | 1469.574 | 1469.605 | 0.002 | 1469.569 | 0.000 |
| 60.0 | 0.35 | 2203.783 | 2203.818 | 0.002 | 2203.777 | 0.000 |
| 80.0 | 0.46 | 2937.938 | 2937.970 | 0.001 | 2937.928 | 0.000 |
| 100.0 | 0.58 | 3672.056 | 3672.084 | 0.001 | 3672.043 | 0.000 |
| 120.0 | 0.70 | 4406.160 | 4406.171 | 0.000 | 4406.135 | 0.001 |
| 140.0 | 0.81 | 5140.234 | 5140.238 | 0.000 | 5140.211 | 0.000 |
| 160.0 | 0.93 | 5873.712 | 5874.292 | 0.010 | 5874.277 | 0.010 |
| $\boldsymbol{\epsilon_{\mathrm{AVE}}}(\%)$ | | | | **0.003** | | **0.001** |
| $\boldsymbol{\epsilon_{\mathrm{MAX}}}(\%)$ | | | | **0.010** | | **0.010** |

**Table 8c.** The reduced excess internal energy due to particle-particle interactions $u_{\rm ex}^{\rm pp}$ resulting from molecular dynamics (MD) simulations and from two versions of the isomorph-based empirically modified hypernetted chain (IEMHNC) approach: the version constructed with the OCP bridge function given by Iyetomi, Ogata and Ichimaru (IOI) in *H. Iyetomi, S. Ogata and S. Ichimaru, Phys. Rev. A* **46**, *1051 (1992)* and the version constructed with the new OCP bridge function parameterization proposed by the authors (LCT). The absolute relative deviation $\epsilon_{\rm r}$ between the theoretical and the simulation results is also reported together with its average and maximum values (the average deviation is denoted as $\epsilon_{\rm AVE}$ and the maximum deviation is denoted as $\epsilon_{\rm MAX}$). **Results in the case of $\boldsymbol{\kappa} = 0.4$.** The MD results are adopted from *R. T. Farouki and S. Hamaguchi, J. Chem. Phys.* **101**, *9885 (1994)*.

| $\Gamma$ | $\Gamma/\Gamma_m$ | $u_{\rm ex}^{\rm pp,MD}$ | $u_{\rm ex}^{pp,{\rm pp,IOI}}$ | $\epsilon_{\rm IOI}(\%)$ | $u_{\rm ex}^{\rm pp,LCT}$ | $\epsilon_{\rm LCT}(\%)$ |
|---|---|---|---|---|---|---|
| 10.0 | 0.06 | 87.571 | 87.602 | 0.035 | 87.569 | 0.002 |
| 20.0 | 0.11 | 174.480 | 174.508 | 0.016 | 174.474 | 0.003 |
| 40.0 | 0.23 | 348.064 | 348.091 | 0.008 | 348.054 | 0.003 |
| 60.0 | 0.34 | 521.526 | 521.555 | 0.005 | 521.514 | 0.002 |
| 80.0 | 0.45 | 694.927 | 694.959 | 0.005 | 694.917 | 0.001 |
| 100.0 | 0.57 | 868.304 | 868.325 | 0.002 | 868.284 | 0.002 |
| 120.0 | 0.68 | 1041.667 | 1041.665 | 0.000 | 1041.628 | 0.004 |
| 140.0 | 0.79 | 1214.982 | 1214.985 | 0.000 | 1214.955 | 0.002 |
| 160.0 | 0.91 | 1387.654 | 1388.289 | 0.046 | 1388.271 | 0.044 |
| $\boldsymbol{\epsilon_{\rm AVE}}(\%)$ | | | | **0.013** | | **0.007** |
| $\boldsymbol{\epsilon_{\rm MAX}}(\%)$ | | | | **0.046** | | **0.044** |

**Table 8d.** The reduced excess internal energy due to particle-particle interactions $u_{\rm ex}^{\rm pp}$ resulting from molecular dynamics (MD) simulations and from two versions of the isomorph-based empirically modified hypernetted chain (IEMHNC) approach: the version constructed with the OCP bridge function given by Iyetomi, Ogata and Ichimaru (IOI) in *H. Iyetomi, S. Ogata and S. Ichimaru, Phys. Rev. A* **46**, *1051 (1992)* and the version constructed with the new OCP bridge function parameterization proposed by the authors (LCT). The absolute relative deviation $\epsilon_{\rm r}$ between the theoretical and the simulation results is also reported together with its average and maximum values (the average deviation is denoted as $\epsilon_{\rm AVE}$ and the maximum deviation is denoted as $\epsilon_{\rm MAX}$). **Results in the case of $\boldsymbol{\kappa} = 0.6$.** The MD results are adopted from *R. T. Farouki and S. Hamaguchi, J. Chem. Phys.* **101**, *9885 (1994)*.

| $\Gamma$ | $\Gamma/\Gamma_m$ | $u_{\rm ex}^{\rm pp,MD}$ | $u_{\rm ex}^{pp,{\rm pp,IOI}}$ | $\epsilon_{\rm IOI}(\%)$ | $u_{\rm ex}^{\rm pp,LCT}$ | $\epsilon_{\rm LCT}(\%)$ |
|---|---|---|---|---|---|---|
| 10.0 | 0.05 | 36.262 | 36.292 | 0.082 | 36.259 | 0.008 |
| 20.0 | 0.11 | 71.877 | 71.906 | 0.040 | 71.873 | 0.006 |
| 40.0 | 0.22 | 142.878 | 142.910 | 0.022 | 142.874 | 0.003 |
| 60.0 | 0.32 | 213.769 | 213.798 | 0.013 | 213.758 | 0.005 |
| 80.0 | 0.43 | 284.608 | 284.627 | 0.007 | 284.585 | 0.008 |
| 100.0 | 0.54 | 355.406 | 355.420 | 0.004 | 355.378 | 0.008 |
| 120.0 | 0.65 | 426.172 | 426.186 | 0.003 | 426.147 | 0.006 |
| 140.0 | 0.75 | 496.928 | 496.932 | 0.001 | 496.900 | 0.006 |
| 160.0 | 0.86 | 567.668 | 567.663 | 0.001 | 567.640 | 0.005 |
| 180.0 | 0.97 | 637.721 | 638.382 | 0.104 | 638.373 | 0.102 |
| $\boldsymbol{\epsilon_{\rm AVE}}(\%)$ | | | | **0.028** | | **0.016** |
| $\boldsymbol{\epsilon_{\rm MAX}}(\%)$ | | | | **0.104** | | **0.102** |

**Table 8e.** The reduced excess internal energy due to particle-particle interactions $u_{\mathrm{ex}}^{\mathrm{pp}}$ resulting from molecular dynamics (MD) simulations and from two versions of the isomorph-based empirically modified hypernetted chain (IEMHNC) approach: the version constructed with the OCP bridge function given by Iyetomi, Ogata and Ichimaru (IOI) in *H. Iyetomi, S. Ogata and S. Ichimaru, Phys. Rev. A* **46**, *1051 (1992)* and the version constructed with the new OCP bridge function parameterization proposed by the authors (LCT). The absolute relative deviation $\epsilon_{\mathrm{r}}$ between the theoretical and the simulation results is also reported together with its average and maximum values (the average deviation is denoted as $\epsilon_{\mathrm{AVE}}$ and the maximum deviation is denoted as $\epsilon_{\mathrm{MAX}}$). **Results in the case of $\boldsymbol{\kappa = 0.8}$**. The MD results are adopted from *R. T. Farouki and S. Hamaguchi, J. Chem. Phys.* **101**, *9885 (1994)*.

| $\Gamma$ | $\Gamma/\Gamma_m$ | $u_{\mathrm{ex}}^{\mathrm{pp,MD}}$ | $u_{\mathrm{ex}}^{pp,\mathrm{pp,IOI}}$ | $\epsilon_{\mathrm{IOI}}(\%)$ | $u_{\mathrm{ex}}^{\mathrm{pp,LCT}}$ | $\epsilon_{\mathrm{LCT}}(\%)$ |
|---|---|---|---|---|---|---|
| 10.0 | 0.05 | 18.718 | 18.751 | 0.174 | 18.717 | 0.003 |
| 20.0 | 0.10 | 36.821 | 36.848 | 0.073 | 36.815 | 0.016 |
| 40.0 | 0.20 | 72.801 | 72.826 | 0.034 | 72.791 | 0.014 |
| 60.0 | 0.30 | 108.666 | 108.690 | 0.022 | 108.650 | 0.014 |
| 80.0 | 0.40 | 144.482 | 144.497 | 0.011 | 144.455 | 0.019 |
| 100.0 | 0.50 | 180.249 | 180.269 | 0.011 | 180.226 | 0.012 |
| 120.0 | 0.60 | 216.011 | 216.015 | 0.002 | 215.975 | 0.017 |
| 140.0 | 0.70 | 251.747 | 251.742 | 0.002 | 251.706 | 0.016 |
| 160.0 | 0.80 | 287.472 | 287.454 | 0.006 | 287.425 | 0.016 |
| 180.0 | 0.90 | 322.564 | 323.154 | 0.183 | 323.135 | 0.177 |
| $\boldsymbol{\epsilon_{\mathrm{AVE}}}(\%)$ | | | | **0.052** | | **0.031** |
| $\boldsymbol{\epsilon_{\mathrm{MAX}}}(\%)$ | | | | **0.183** | | **0.177** |

**Table 8f.** The reduced excess internal energy due to particle-particle interactions $u_{\mathrm{ex}}^{\mathrm{pp}}$ resulting from molecular dynamics (MD) simulations and from two versions of the isomorph-based empirically modified hypernetted chain (IEMHNC) approach: the version constructed with the OCP bridge function given by Iyetomi, Ogata and Ichimaru (IOI) in *H. Iyetomi, S. Ogata and S. Ichimaru, Phys. Rev. A* **46**, *1051 (1992)* and the version constructed with the new OCP bridge function parameterization proposed by the authors (LCT). The absolute relative deviation $\epsilon_{\mathrm{r}}$ between the theoretical and the simulation results is also reported together with its average and maximum values (the average deviation is denoted as $\epsilon_{\mathrm{AVE}}$ and the maximum deviation is denoted as $\epsilon_{\mathrm{MAX}}$). **Results in the case of $\boldsymbol{\kappa = 1.0}$**. The MD results are adopted from *R. T. Farouki and S. Hamaguchi, J. Chem. Phys.* **101**, *9885 (1994)*.

| $\Gamma$ | $\Gamma/\Gamma_m$ | $u_{\mathrm{ex}}^{\mathrm{pp,MD}}$ | $u_{\mathrm{ex}}^{pp,\mathrm{pp,IOI}}$ | $\epsilon_{\mathrm{IOI}}(\%)$ | $u_{\mathrm{ex}}^{\mathrm{pp,LCT}}$ | $\epsilon_{\mathrm{LCT}}(\%)$ |
|---|---|---|---|---|---|---|
| 10.0 | 0.05 | 10.890 | 10.920 | 0.275 | 10.887 | 0.032 |
| 20.0 | 0.09 | 21.194 | 21.217 | 0.110 | 21.185 | 0.043 |
| 40.0 | 0.18 | 41.575 | 41.602 | 0.065 | 41.568 | 0.017 |
| 60.0 | 0.27 | 61.854 | 61.877 | 0.037 | 61.839 | 0.024 |
| 80.0 | 0.36 | 82.074 | 82.098 | 0.029 | 82.057 | 0.021 |
| 100.0 | 0.45 | 102.265 | 102.284 | 0.019 | 102.241 | 0.023 |
| 120.0 | 0.54 | 122.429 | 122.446 | 0.014 | 122.404 | 0.021 |
| 140.0 | 0.64 | 142.582 | 142.589 | 0.005 | 142.549 | 0.023 |
| 160.0 | 0.73 | 162.715 | 162.717 | 0.001 | 162.683 | 0.020 |
| 180.0 | 0.82 | 182.839 | 182.834 | 0.003 | 182.806 | 0.018 |
| 200.0 | 0.91 | 202.358 | 202.941 | 0.288 | 202.923 | 0.279 |
| $\boldsymbol{\epsilon_{\mathrm{AVE}}}(\%)$ | | | | **0.077** | | **0.047** |
| $\boldsymbol{\epsilon_{\mathrm{MAX}}}(\%)$ | | | | **0.288** | | **0.279** |

**Table 8g.** The reduced excess internal energy due to particle-particle interactions $u_{\mathrm{ex}}^{\mathrm{pp}}$ resulting from molecular dynamics (MD) simulations and from two versions of the isomorph-based empirically modified hypernetted chain (IEMHNC) approach: the version constructed with the OCP bridge function given by Iyetomi, Ogata and Ichimaru (IOI) in *H. Iyetomi, S. Ogata and S. Ichimaru, Phys. Rev. A* **46**, *1051 (1992)* and the version constructed with the new OCP bridge function parameterization proposed by the authors (LCT). The absolute relative deviation $\epsilon_{\mathrm{r}}$ between the theoretical and the simulation results is also reported together with its average and maximum values (the average deviation is denoted as $\epsilon_{\mathrm{AVE}}$ and the maximum deviation is denoted as $\epsilon_{\mathrm{MAX}}$). **Results in the case of $\boldsymbol{\kappa = 1.2}$**. The MD results are adopted from *S. Hamaguchi, R. T. Farouki, D. H. E. Dubin, Phys. Rev. E* **56**, *4671 (1997)*.

| $\Gamma$ | $\Gamma/\Gamma_m$ | $u_{\mathrm{ex}}^{\mathrm{pp,MD}}$ | $u_{\mathrm{ex}}^{pp,\mathrm{pp,IOI}}$ | $\epsilon_{\mathrm{IOI}}(\%)$ | $u_{\mathrm{ex}}^{\mathrm{pp,LCT}}$ | $\epsilon_{\mathrm{LCT}}(\%)$ |
|---|---|---|---|---|---|---|
| 10.0 | 0.04 | 6.831 | 6.867 | 0.523 | 6.834 | 0.049 |
| 20.0 | 0.08 | 13.124 | 13.149 | 0.189 | 13.116 | 0.058 |
| 40.0 | 0.16 | 25.485 | 25.508 | 0.091 | 25.475 | 0.040 |
| 60.0 | 0.24 | 37.734 | 37.762 | 0.074 | 37.726 | 0.022 |
| 80.0 | 0.32 | 49.942 | 49.964 | 0.044 | 49.924 | 0.036 |
| 100.0 | 0.40 | 62.098 | 62.133 | 0.057 | 62.091 | 0.012 |
| 120.0 | 0.49 | 74.273 | 74.279 | 0.008 | 74.236 | 0.050 |
| 140.0 | 0.57 | 86.398 | 86.407 | 0.010 | 86.365 | 0.038 |
| 160.0 | 0.65 | 98.520 | 98.521 | 0.001 | 98.482 | 0.039 |
| 180.0 | 0.73 | 110.606 | 110.624 | 0.016 | 110.589 | 0.015 |
| 200.0 | 0.81 | 122.732 | 122.718 | 0.012 | 122.689 | 0.035 |
| $\boldsymbol{\epsilon_{\mathrm{AVE}}}(\%)$ | | | | **0.093** | | **0.036** |
| $\boldsymbol{\epsilon_{\mathrm{MAX}}}(\%)$ | | | | **0.523** | | **0.058** |

**Table 8h.** The reduced excess internal energy due to particle-particle interactions $u_{\mathrm{ex}}^{\mathrm{pp}}$ resulting from molecular dynamics (MD) simulations and from two versions of the isomorph-based empirically modified hypernetted chain (IEMHNC) approach: the version constructed with the OCP bridge function given by Iyetomi, Ogata and Ichimaru (IOI) in *H. Iyetomi, S. Ogata and S. Ichimaru, Phys. Rev. A* **46**, *1051 (1992)* and the version constructed with the new OCP bridge function parameterization proposed by the authors (LCT). The absolute relative deviation $\epsilon_{\mathrm{r}}$ between the theoretical and the simulation results is also reported together with its average and maximum values (the average deviation is denoted as $\epsilon_{\mathrm{AVE}}$ and the maximum deviation is denoted as $\epsilon_{\mathrm{MAX}}$). **Results in the case of $\boldsymbol{\kappa = 1.4}$**. The MD results are adopted from *S. Hamaguchi, R. T. Farouki, D. H. E. Dubin, Phys. Rev. E* **56**, *4671 (1997)*.

| $\Gamma$ | $\Gamma/\Gamma_m$ | $u_{\mathrm{ex}}^{\mathrm{pp,MD}}$ | $u_{\mathrm{ex}}^{pp,\mathrm{pp,IOI}}$ | $\epsilon_{\mathrm{IOI}}(\%)$ | $u_{\mathrm{ex}}^{\mathrm{pp,LCT}}$ | $\epsilon_{\mathrm{LCT}}(\%)$ |
|---|---|---|---|---|---|---|
| 10.0 | 0.04 | 4.533 | 4.561 | 0.614 | 4.532 | 0.015 |
| 20.0 | 0.07 | 8.564 | 8.585 | 0.241 | 8.552 | 0.138 |
| 40.0 | 0.14 | 16.406 | 16.427 | 0.125 | 16.394 | 0.074 |
| 60.0 | 0.21 | 24.153 | 24.168 | 0.062 | 24.133 | 0.082 |
| 80.0 | 0.28 | 31.853 | 31.860 | 0.022 | 31.822 | 0.097 |
| 100.0 | 0.35 | 39.498 | 39.521 | 0.059 | 39.480 | 0.045 |
| 120.0 | 0.42 | 47.135 | 47.160 | 0.054 | 47.118 | 0.036 |
| 140.0 | 0.50 | 54.771 | 54.783 | 0.022 | 54.740 | 0.057 |
| 160.0 | 0.57 | 62.374 | 62.392 | 0.029 | 62.350 | 0.038 |
| 180.0 | 0.64 | 69.991 | 69.991 | 0.000 | 69.951 | 0.057 |
| 200.0 | 0.71 | 77.564 | 77.580 | 0.021 | 77.544 | 0.026 |
| 240.0 | 0.85 | 92.744 | 92.738 | 0.006 | 92.713 | 0.034 |
| $\boldsymbol{\epsilon_{\mathrm{AVE}}}(\%)$ | | | | **0.105** | | **0.058** |
| $\boldsymbol{\epsilon_{\mathrm{MAX}}}(\%)$ | | | | **0.614** | | **0.138** |

**Table 8i.** The reduced excess internal energy due to particle-particle interactions $u_{\rm ex}^{\rm pp}$ resulting from molecular dynamics (MD) simulations and from two versions of the isomorph-based empirically modified hypernetted chain (IEMHNC) approach: the version constructed with the OCP bridge function given by Iyetomi, Ogata and Ichimaru (IOI) in *H. Iyetomi, S. Ogata and S. Ichimaru, Phys. Rev. A* **46**, *1051 (1992)* and the version constructed with the new OCP bridge function parameterization proposed by the authors (LCT). The absolute relative deviation $\epsilon_{\rm r}$ between the theoretical and the simulation results is also reported together with its average and maximum values (the average deviation is denoted as $\epsilon_{\rm AVE}$ and the maximum deviation is denoted as $\epsilon_{\rm MAX}$). **Results in the case of $\boldsymbol{\kappa = 2.0}$**. The MD results are adopted from *S. Hamaguchi, R. T. Farouki, D. H. E. Dubin, Phys. Rev. E* **56**, *4671 (1997)*.

| $\Gamma$ | $\Gamma/\Gamma_m$ | $u_{\rm ex}^{\rm pp,MD}$ | $u_{\rm ex}^{pp,\rm pp,IOI}$ | $\epsilon_{\rm IOI}(\%)$ | $u_{\rm ex}^{\rm pp,LCT}$ | $\epsilon_{\rm LCT}(\%)$ |
|---|---|---|---|---|---|---|
| 20.0 | 0.04 | 2.944 | 2.976 | 1.091 | 2.943 | 0.029 |
| 40.0 | 0.09 | 5.343 | 5.361 | 0.333 | 5.329 | 0.262 |
| 60.0 | 0.13 | 7.630 | 7.662 | 0.421 | 7.631 | 0.008 |
| 80.0 | 0.17 | 9.903 | 9.923 | 0.198 | 9.890 | 0.128 |
| 100.0 | 0.22 | 12.133 | 12.158 | 0.204 | 12.124 | 0.077 |
| 200.0 | 0.44 | 23.107 | 23.137 | 0.130 | 23.094 | 0.055 |
| $\boldsymbol{\epsilon_{\rm AVE}}(\%)$ | | | | **0.396** | | **0.093** |
| $\boldsymbol{\epsilon_{\rm MAX}}(\%)$ | | | | **1.091** | | **0.262** |

**Table 8j.** The reduced excess internal energy due to particle-particle interactions $u_{\rm ex}^{\rm pp}$ resulting from molecular dynamics (MD) simulations and from two versions of the isomorph-based empirically modified hypernetted chain (IEMHNC) approach: the version constructed with the OCP bridge function given by Iyetomi, Ogata and Ichimaru (IOI) in *H. Iyetomi, S. Ogata and S. Ichimaru, Phys. Rev. A* **46**, *1051 (1992)* and the version constructed with the new OCP bridge function parameterization proposed by the authors (LCT). The absolute relative deviation $\epsilon_{\rm r}$ between the theoretical and the simulation results is also reported together with its average and maximum values (the average deviation is denoted as $\epsilon_{\rm AVE}$ and the maximum deviation is denoted as $\epsilon_{\rm MAX}$). **Results in the case of $\boldsymbol{\kappa = 2.6}$**. The MD results are adopted from *S. Hamaguchi, R. T. Farouki, D. H. E. Dubin, Phys. Rev. E* **56**, *4671 (1997)*.

| $\Gamma$ | $\Gamma/\Gamma_m$ | $u_{\rm ex}^{\rm pp,MD}$ | $u_{\rm ex}^{pp,\rm pp,IOI}$ | $\epsilon_{\rm IOI}(\%)$ | $u_{\rm ex}^{\rm pp,LCT}$ | $\epsilon_{\rm LCT}(\%)$ |
|---|---|---|---|---|---|---|
| 40.0 | 0.05 | 2.165 | 2.202 | 1.696 | 2.169 | 0.205 |
| 60.0 | 0.07 | 2.986 | 3.012 | 0.873 | 2.981 | 0.169 |
| 80.0 | 0.10 | 3.772 | 3.791 | 0.501 | 3.760 | 0.309 |
| 100.0 | 0.12 | 4.528 | 4.550 | 0.486 | 4.520 | 0.184 |
| 200.0 | 0.25 | 8.181 | 8.194 | 0.157 | 8.159 | 0.265 |
| 400.0 | 0.49 | 15.147 | 15.167 | 0.130 | 15.124 | 0.154 |
| 700.0 | 0.86 | 25.319 | 25.322 | 0.011 | 25.296 | 0.090 |
| $\boldsymbol{\epsilon_{\rm AVE}}(\%)$ | | | | **0.551** | | **0.196** |
| $\boldsymbol{\epsilon_{\rm MAX}}(\%)$ | | | | **1.696** | | **0.309** |

**Table 8k.** The reduced excess internal energy due to particle-particle interactions $u_{\rm ex}^{\rm pp}$ resulting from molecular dynamics (MD) simulations and from two versions of the isomorph-based empirically modified hypernetted chain (IEMHNC) approach: the version constructed with the OCP bridge function given by Iyetomi, Ogata and Ichimaru (IOI) in *H. Iyetomi, S. Ogata and S. Ichimaru, Phys. Rev. A* **46**, *1051 (1992)* and the version constructed with the new OCP bridge function parameterization proposed by the authors (LCT). The absolute relative deviation $\epsilon_{\rm r}$ between the theoretical and the simulation results is also reported together with its average and maximum values (the average deviation is denoted as $\epsilon_{\rm AVE}$ and the maximum deviation is denoted as $\epsilon_{\rm MAX}$). **Results in the case of $\boldsymbol{\kappa = 3.0}$**. The MD results are adopted from *S. Hamaguchi, R. T. Farouki, D. H. E. Dubin, Phys. Rev. E* **56**, *4671 (1997)*.

| $\Gamma$ | $\Gamma/\Gamma_m$ | $u_{\rm ex}^{\rm pp,MD}$ | $u_{\rm ex}^{pp,\rm pp,IOI}$ | $\epsilon_{\rm IOI}(\%)$ | $u_{\rm ex}^{\rm pp,LCT}$ | $\epsilon_{\rm LCT}(\%)$ |
|---|---|---|---|---|---|---|
| 40.0 | 0.03 | 1.322 | 1.345 | 1.766 | 1.323 | 0.081 |
| 60.0 | 0.05 | 1.769 | 1.798 | 1.613 | 1.766 | 0.155 |
| 80.0 | 0.06 | 2.189 | 2.211 | 1.012 | 2.181 | 0.388 |
| 100.0 | 0.08 | 2.582 | 2.608 | 1.021 | 2.578 | 0.144 |
| 200.0 | 0.16 | 4.456 | 4.470 | 0.312 | 4.440 | 0.357 |
| 400.0 | 0.32 | 7.928 | 7.938 | 0.120 | 7.899 | 0.361 |
| 700.0 | 0.57 | 12.869 | 12.897 | 0.214 | 12.854 | 0.113 |
| $\boldsymbol{\epsilon_{\rm AVE}}(\%)$ | | | | **0.865** | | **0.228** |
| $\boldsymbol{\epsilon_{\rm MAX}}(\%)$ | | | | **1.766** | | **0.388** |

**Table 8l.** The reduced excess internal energy due to particle-particle interactions $u_{\rm ex}^{\rm pp}$ resulting from molecular dynamics (MD) simulations and from two versions of the isomorph-based empirically modified hypernetted chain (IEMHNC) approach: the version constructed with the OCP bridge function given by Iyetomi, Ogata and Ichimaru (IOI) in *H. Iyetomi, S. Ogata and S. Ichimaru, Phys. Rev. A* **46**, *1051 (1992)* and the version constructed with the new OCP bridge function parameterization proposed by the authors (LCT). The absolute relative deviation $\epsilon_{\rm r}$ between the theoretical and the simulation results is also reported together with its average and maximum values (the average deviation is denoted as $\epsilon_{\rm AVE}$ and the maximum deviation is denoted as $\epsilon_{\rm MAX}$). **Results in the case of $\boldsymbol{\kappa = 3.6}$**. The MD results are adopted from *S. Hamaguchi, R. T. Farouki, D. H. E. Dubin, Phys. Rev. E* **56**, *4671 (1997)*.

| $\Gamma$ | $\Gamma/\Gamma_m$ | $u_{\rm ex}^{\rm pp,MD}$ | $u_{\rm ex}^{pp,\rm pp,IOI}$ | $\epsilon_{\rm IOI}(\%)$ | $u_{\rm ex}^{\rm pp,LCT}$ | $\epsilon_{\rm LCT}(\%)$ |
|---|---|---|---|---|---|---|
| 80.0 | 0.03 | 1.092 | 1.126 | 3.135 | 1.105 | 1.159 |
| 100.0 | 0.04 | 1.272 | 1.304 | 2.540 | 1.276 | 0.323 |
| 200.0 | 0.08 | 2.035 | 2.062 | 1.304 | 2.033 | 0.099 |
| 400.0 | 0.17 | 3.378 | 3.386 | 0.248 | 3.358 | 0.596 |
| 700.0 | 0.29 | 5.200 | 5.205 | 0.090 | 5.170 | 0.586 |
| 1000.0 | 0.42 | 6.934 | 6.930 | 0.053 | 6.890 | 0.636 |
| 2000.0 | 0.83 | 12.399 | 12.382 | 0.139 | 12.354 | 0.367 |
| $\boldsymbol{\epsilon_{\rm AVE}}(\%)$ | | | | **1.073** | | **0.538** |
| $\boldsymbol{\epsilon_{\rm MAX}}(\%)$ | | | | **3.135** | | **1.159** |

**Table 8m.** The reduced excess internal energy due to particle-particle interactions $u_{\mathrm{ex}}^{\mathrm{pp}}$ resulting from molecular dynamics (MD) simulations and from two versions of the isomorph-based empirically modified hypernetted chain (IEMHNC) approach: the version constructed with the OCP bridge function given by Iyetomi, Ogata and Ichimaru (IOI) in *H. Iyetomi, S. Ogata and S. Ichimaru, Phys. Rev. A* **46**, *1051 (1992)* and the version constructed with the new OCP bridge function parameterization proposed by the authors (LCT). The absolute relative deviation $\epsilon_{\mathrm{r}}$ between the theoretical and the simulation results is also reported together with its average and maximum values (the average deviation is denoted as $\epsilon_{\mathrm{AVE}}$ and the maximum deviation is denoted as $\epsilon_{\mathrm{MAX}}$). **Results in the case of $\boldsymbol{\kappa = 4.0}$**. The MD results are adopted from *S. Hamaguchi, R. T. Farouki, D. H. E. Dubin, Phys. Rev. E* **56**, *4671 (1997)*.

| $\Gamma$ | $\Gamma/\Gamma_m$ | $u_{\mathrm{ex}}^{\mathrm{pp,MD}}$ | $u_{\mathrm{ex}}^{pp,\mathrm{pp,IOI}}$ | $\epsilon_{\mathrm{IOI}}(\%)$ | $u_{\mathrm{ex}}^{\mathrm{pp,LCT}}$ | $\epsilon_{\mathrm{LCT}}(\%)$ |
|---|---|---|---|---|---|---|
| 200.0 | 0.05 | 1.305 | 1.345 | 3.027 | 1.316 | 0.859 |
| 400.0 | 0.10 | 2.066 | 2.091 | 1.223 | 2.064 | 0.090 |
| 700.0 | 0.18 | 3.054 | 3.077 | 0.744 | 3.049 | 0.178 |
| 1000.0 | 0.26 | 3.971 | 3.991 | 0.497 | 3.958 | 0.321 |
| 2000.0 | 0.52 | 6.824 | 6.810 | 0.209 | 6.769 | 0.807 |
| $\boldsymbol{\epsilon_{\mathrm{AVE}}}(\%)$ | | | | **1.140** | | **0.451** |
| $\boldsymbol{\epsilon_{\mathrm{MAX}}}(\%)$ | | | | **3.027** | | **0.859** |

**Table 8n.** The reduced excess internal energy due to particle-particle interactions $u_{\mathrm{ex}}^{\mathrm{pp}}$ resulting from molecular dynamics (MD) simulations and from two versions of the isomorph-based empirically modified hypernetted chain (IEMHNC) approach: the version constructed with the OCP bridge function given by Iyetomi, Ogata and Ichimaru (IOI) in *H. Iyetomi, S. Ogata and S. Ichimaru, Phys. Rev. A* **46**, *1051 (1992)* and the version constructed with the new OCP bridge function parameterization proposed by the authors (LCT). The absolute relative deviation $\epsilon_{\mathrm{r}}$ between the theoretical and the simulation results is also reported together with its average and maximum values (the average deviation is denoted as $\epsilon_{\mathrm{AVE}}$ and the maximum deviation is denoted as $\epsilon_{\mathrm{MAX}}$). **Results in the case of $\boldsymbol{\kappa = 4.6}$**. The MD results are adopted from *S. Hamaguchi, R. T. Farouki, D. H. E. Dubin, Phys. Rev. E* **56**, *4671 (1997)*.

| $\Gamma$ | $\Gamma/\Gamma_m$ | $u_{\mathrm{ex}}^{\mathrm{pp,MD}}$ | $u_{\mathrm{ex}}^{pp,\mathrm{pp,IOI}}$ | $\epsilon_{\mathrm{IOI}}(\%)$ | $u_{\mathrm{ex}}^{\mathrm{pp,LCT}}$ | $\epsilon_{\mathrm{LCT}}(\%)$ |
|---|---|---|---|---|---|---|
| 400.0 | 0.05 | 1.114 | 1.148 | 3.089 | 1.122 | 0.719 |
| 700.0 | 0.09 | 1.553 | 1.586 | 2.113 | 1.560 | 0.450 |
| 1000.0 | 0.13 | 1.947 | 1.973 | 1.325 | 1.947 | 0.016 |
| 2000.0 | 0.25 | 3.119 | 3.110 | 0.292 | 3.079 | 1.273 |
| 3000.0 | 0.38 | 4.126 | 4.136 | 0.249 | 4.099 | 0.648 |
| 4000.0 | 0.50 | 5.118 | 5.104 | 0.265 | 5.065 | 1.035 |
| 5000.0 | 0.63 | 6.047 | 6.035 | 0.199 | 5.997 | 0.827 |
| 6000.0 | 0.76 | 6.969 | 6.939 | 0.432 | 6.906 | 0.898 |
| $\boldsymbol{\epsilon_{\mathrm{AVE}}}(\%)$ | | | | **0.995** | | **0.733** |
| $\boldsymbol{\epsilon_{\mathrm{MAX}}}(\%)$ | | | | **3.089** | | **1.273** |

**Table 8o.** The reduced excess internal energy due to particle-particle interactions $u_{\rm ex}^{\rm pp}$ resulting from molecular dynamics (MD) simulations and from two versions of the isomorph-based empirically modified hypernetted chain (IEMHNC) approach: the version constructed with the OCP bridge function given by Iyetomi, Ogata and Ichimaru (IOI) in *H. Iyetomi, S. Ogata and S. Ichimaru, Phys. Rev. A* **46**, *1051 (1992)* and the version constructed with the new OCP bridge function parameterization proposed by the authors (LCT). The absolute relative deviation $\epsilon_{\rm r}$ between the theoretical and the simulation results is also reported together with its average and maximum values (the average deviation is denoted as $\epsilon_{\rm AVE}$ and the maximum deviation is denoted as $\epsilon_{\rm MAX}$). **Results in the case of $\boldsymbol{\kappa} = 5.0$**. The MD results are adopted from *S. Hamaguchi, R. T. Farouki, D. H. E. Dubin, Phys. Rev. E* **56**, *4671 (1997)*.

| $\Gamma$ | $\Gamma/\Gamma_m$ | $u_{\rm ex}^{\rm pp,MD}$ | $u_{\rm ex}^{pp,\rm pp,IOI}$ | $\epsilon_{\rm IOI}(\%)$ | $u_{\rm ex}^{\rm pp,LCT}$ | $\epsilon_{\rm LCT}(\%)$ |
|---|---|---|---|---|---|---|
| 700.0 | 0.05 | 1.067 | 1.101 | 3.191 | 1.076 | 0.826 |
| 1000.0 | 0.08 | 1.295 | 1.336 | 3.175 | 1.311 | 1.249 |
| 2000.0 | 0.15 | 1.978 | 1.999 | 1.073 | 1.974 | 0.186 |
| 3000.0 | 0.23 | 2.568 | 2.577 | 0.360 | 2.549 | 0.744 |
| 4000.0 | 0.31 | 3.108 | 3.112 | 0.141 | 3.080 | 0.914 |
| 5000.0 | 0.38 | 3.625 | 3.620 | 0.140 | 3.584 | 1.139 |
| 6000.0 | 0.46 | 4.140 | 4.108 | 0.783 | 4.070 | 1.702 |
| 8000.0 | 0.61 | 5.072 | 5.041 | 0.620 | 5.003 | 1.359 |
| 10000.0 | 0.76 | 5.900 | 5.934 | 0.571 | 5.903 | 0.044 |
| $\boldsymbol{\epsilon_{\rm AVE}}(\%)$ | | | | **1.117** | | **0.907** |
| $\boldsymbol{\epsilon_{\rm MAX}}(\%)$ | | | | **3.191** | | **1.702** |
